# Supplementary material for: Learning Causality for Longitudinal Data
Source: arXiv:2512.04980 source file (2025-12-04)
Supplement: Supplementary file 1 [file 3.tex]

\chapter{Appendix: Chapter \ref{chapter:cdvae}}
\section{Proofs}
\label{appendix_cdvae:proofs}

\subsection{Identifiability: Treatment Effects and Unobserved Adjustment Variables}
\label{appendix:proof_effect_Z}
\begin{proof}[\textbf{CATE Identifiability}]
Assuming the consistency, overlap, and ignorability assumptions (\ref{assp:consistency_seq}, \ref{assp:overlap_seq}, \ref{assp:seq_ignorability}), we demonstrate that the Conditional Average Treatment Effect (CATE), as defined in Eq. \ref{eq:CATE_Identifiability}, is identifiable from the observed data distribution:
\begin{equation}
\tau_t = \mathbb{E}(Y_{t}| \mathbf{H}_t = \mathbf{h}_t, W_{t} = 1) - \mathbb{E}(Y_{t}| \mathbf{H}_t = \mathbf{h}_t, W_{t} = 0).
\end{equation}

Establishing the identifiability of CATE requires showing that the two potential outcome expectations are identifiable. By the ignorability assumption (\ref{assp:seq_ignorability}), the potential outcome under treatment can be expressed as:
\[
m_{t}^{1}(\mathbf{h}_{t}) = \mathbb{E}_{Y_{t}(1) \mid \mathbf{H}_{t} }(Y_{t}(1) \mid \mathbf{H}_{t} = \mathbf{h}_{t}) = \mathbb{E}_{Y_{t}(1) \mid \mathbf{H}_{t}, W_t }(Y_{t}(1) \mid \mathbf{H}_{t} = \mathbf{h}_{t}, W_t = 1).
\]
Using the consistency assumption (\ref{assp:consistency_seq}), the observed response can identify \( Y_{t}(1) \) when conditioned on \( W_t = 1 \):
\[
m_{t}^{1}(\mathbf{h}_{t}) = \mathbb{E}_{Y_{t} \mid \mathbf{H}_{t}, W_t }(Y_{t}\mid \mathbf{H}_{t} = \mathbf{h}_{t}, W_t = 1).
\]
Similarly, we identify the expected potential outcome under no treatment:
\[
m_{t}^{0}(\mathbf{h}_{t}) = \mathbb{E}_{Y_{t} \mid \mathbf{H}_{t}, W_t }(Y_{t}\mid \mathbf{H}_{t} = \mathbf{h}_{t}, W_t = 0).
\]
The existence of these expectations is guaranteed by the overlap assumption.
\end{proof}

\begin{proof}[\textbf{Augmented CATE Identifiability}]
\label{proof:acate_identif}
Assuming that the adjustment variables \(\mathbf{U}\) are observed, we demonstrate the identifiability of the Augmented CATE:
\[
\tau_{t}(\mathbf{h}_{t}, \mathbf{u})= \mathbb{E}(Y_{t}| \mathbf{H}_t = \mathbf{h}_t, \mathbf{U}= \mathbf{u}, W_{t} = 1) - \mathbb{E}(Y_{t}| \mathbf{H}_t = \mathbf{h}_t, \mathbf{U}= \mathbf{u}, W_{t} = 0).
\]
The assumptions of consistency, overlap, and ignorability ensure that CATE is identifiable. Since \(\mathbf{U}\) does not affect the treatment, the overlap assumption (\ref{assp:overlap_seq}) remains valid. Further, \(\mathbf{U}\) being independent of the treatment implies that the ignorability assumption holds when conditioning on \(\mathbf{U}\):
\[
Y_{it}(\omega) \indep W_{t}| \mathbf{H}_{t} = \mathbf{h}_{t} \implies Y_{it}(\omega) \indep W_{t}| \mathbf{H}_{t} = \mathbf{h}_{t},\mathbf{U}= \mathbf{u} \quad \forall (\omega, \mathbf{h}_{t}, \mathbf{u}).
\]
The remainder of the proof follows the CATE identifiability argument.
\end{proof}

\begin{proof}[\textbf{Theorem \ref{thm:valid_Z}}]
\label{assp:regularity_y_space}
Let \(\mathbf{Z}\) be a latent variable such that \(\mathbf{Z} \sim CMM(p)\). Any static adjustment variables affecting all response series in the panel must be measurable with respect to \((\mathbf{Z}, \mathbf{H}_T)\). We assume weak regularity conditions on treatment and response domains.
\begin{assumption}[Regularity]
The response domain \(\mathcal{Y}\) is a Borel subset of a compact interval.
\end{assumption}
The treatment domain \(\mathcal{W} = \{0,1\}\) is a Borel subset of \([0,1]\). To prove the theorem, we need the following lemma:
\begin{lemma}[Kernels and Randomization \citep{Kallenberg2021FoundationsOM}]
\label{lem: kernel_RD}
Let \(\mu\) be a probability kernel from a measurable space \(S_1\) to a Borel space \(S_2\). There exists a measurable function \(f: S_1 \times [0,1] \rightarrow S_2\) such that if \(\vartheta\) is uniform on \([0,1]\), then \(f(s_1, \vartheta)\) is distributed as \(\mu(s_1, \cdot)\).
\end{lemma}
Suppose by contradiction the existence of $\mathbf{Z}\prime$ that is not measurable with respect to $(\mathbf{Z}, \mathbf{H}_T)$ and such that: 
\begin{equation*}
    Y_{it}(\omega) \notindep \mathbf{Z_i}\prime| \mathbf{H}_{it}, \mathbf{Z}_i \quad \forall \omega, t
\end{equation*}
Let $t$ be an arbitrary time step in the panel data. By lemma \ref{lem: kernel_RD}, there exists a measurable function  $f_t: \mathcal{H}_t \times \mathcal{W} \times \mathcal{Z} \times [0,1] \rightarrow \mathcal{Y}$ such that: 
\begin{equation*}
    Y_{it} = f_t(\mathbf{H}_{it}, W_{it}, \mathbf{Z}_i, \gamma_{it}), \quad \gamma_{it} \indep (\mathbf{H}_{it}, W_{it}, \mathbf{Z}_i).
\end{equation*}
The conditional Markov property implies the independence of the following conditional distributions: 
\begin{equation*}
    (Y_{it}\mid \mathbf{H}_{it}, \mathbf{Z}_i, W_{it} = \omega) \indep  (Y_{it\prime}\mid \mathbf{H}_{it\prime}, \mathbf{Z}_i, W_{it\prime} = \omega\prime).
\end{equation*}
Such that  $t\prime$ verifies $|t - t\prime| > p$. We can thus conclude that: 
\begin{equation*}
    (Y_{it}(\omega) \mid \mathbf{H}_{it}, \mathbf{Z}_i) \indep  (Y_{it\prime}(\omega\prime) \mid \mathbf{H}_{it\prime}, \mathbf{Z}_i).
\end{equation*}
Because : 
\begin{equation*}
\begin{aligned}
    (Y_{it}(\omega) \mid \mathbf{H}_{it}, \mathbf{Z}_i) &= (Y_{it}(\omega) \mid \mathbf{H}_{it}, \mathbf{Z}_i, W_{it} = \omega)     \\
 &= (Y_{it} \mid \mathbf{H}_{it}, \mathbf{Z}_i, W_{it} = \omega).\\
\end{aligned}
\end{equation*}
The first equality follows from the sequential ignorability of the theorem \ref{thm:seq_ign_augmented}, and the second equality follows the consistency assumption.
 On the other hand, we also have from the CMM(p) that: 
 \begin{equation*}
     \gamma_{it\prime} \indep Y_{it} \mid \mathbf{H}_{it}, \mathbf{Z}_i.
 \end{equation*}
From which it follows using the fact that $\gamma_{it} \indep (\mathbf{H}_{it}, W_{it}, \mathbf{Z}_i)$ and $Y_{it}(\omega) \mid \mathbf{H}_{it}, \mathbf{Z}_i = Y_{it} \mid \mathbf{H}_{it}, \mathbf{Z}_i, W_{it} = \omega $: 
\begin{equation*}
    \gamma_{it\prime} \indep Y_{it}(\omega) \mid \mathbf{H}_{it}, \mathbf{Z}_i
\end{equation*}
By using twice the lemma \ref{lem: kernel_RD}, we write: 
\begin{equation}
    \gamma_{it\prime} = h_t(\mathbf{Z}\prime_i, \eta_{it\prime}), \quad \eta_{it\prime} \indep  \mathbf{Z}\prime_i
\label{eq:gamma}
\end{equation}
And: 
\begin{equation}
    Y_{it}(\omega) = g_t(\mathbf{Z}\prime_i, \epsilon_{it}), \quad \epsilon_{it} \indep  \mathbf{Z}\prime_i.
\label{eq:y_pot}
\end{equation}
Since $ \mathbf{Z}\prime_i$ is not measurable with respect to $( \mathbf{Z}_i, \mathbf{H}_{it})$, then by \eqref{eq:gamma} and \eqref{eq:y_pot}: 
\begin{equation*}
    \gamma_{it\prime} \notindep Y_{it} \mid \mathbf{H}_{it}, \mathbf{Z}_i
\end{equation*}
We have thus a contradiction.
\end{proof}

\subsection{Derivation of CDVAE Loss}
\label{appendix:proof_elbo}
\begin{proof}[\textbf{ELBO}]
We provide proof that the bound in Eq. (\ref{eq:elbo_orig}) is indeed the Evidence Lower Bound (ELBO) for the weighted conditional log-likelihood.

By the concavity of the logarithm, for every \(t \in \{1, 2, \dots, T\}\), we have:
\begin{equation}
\label{eq:elbo_step}
\log p_\theta\left(y_{t} \mid \mathbf{h}_{t}, \omega_t\right) 
\geq 
\underbrace{\mathbb{E}_{\mathbf{Z}, C \sim q_{\phi}(\cdot , \cdot \mid \mathcal{D}_T)}  
\left[  
\log \frac{p_\theta\left(y_{t}, \mathbf{Z}, C\mid \mathbf{h}_{t}, \omega_{t}\right)}{q_{\phi}(\mathbf{Z}, C \mid \mathcal{D}_T)} 
\right]}_{(*)}
\end{equation}

We use the identity
\[
p_\theta(y_t, \mathbf{z}, c \mid \mathbf{h}_t, \omega_t)
= p_\theta(y_t \mid \mathbf{z}, \mathbf{h}_t, \omega_t)\,p(\mathbf{z}, c),
\]
and the factorization of the approximate posterior
\[
q_\phi(\mathbf{z}, c \mid \mathcal{D}_T)
= q_{\phi_z}(\mathbf{z} \mid \mathcal{D}_T)\, q_{\phi_c}(c \mid \mathcal{D}_T),
\]
to write
\[
\begin{aligned}
(*) &=
\mathbb{E}_{\mathbf{Z}, C \sim q_\phi(\cdot,\cdot \mid \mathcal{D}_T)}
\left[
    \log \frac{
        p_\theta(y_t \mid \mathbf{Z}, \mathbf{h}_t, \omega_t)\,p(C \mid \mathbf{Z})\,p(\mathbf{Z})
    }{
        q_{\phi_z}(\mathbf{Z} \mid \mathcal{D}_T)\, q_{\phi_c}(C \mid \mathcal{D}_T)
    }
\right] \\[1.2ex]
&= \mathbb{E}_{\mathbf{Z}, C \sim q_\phi(\cdot,\cdot \mid \mathcal{D}_T)}
\bigl[
    \log p_\theta(y_t \mid \mathbf{Z}, \mathbf{h}_t, \omega_t)
\bigr] \\[0.8ex]
&\hspace{2em}
- \underbrace{D_{KL}\bigl(
    q_{\phi_z}(\mathbf{Z} \mid \mathcal{D}_T)\, q_{\phi_c}(C \mid \mathcal{D}_T)
    \parallel p(C \mid \mathbf{Z})\,p(\mathbf{Z})
\bigr)}_{(**)}.
\end{aligned}
\]

The KL divergence term \((**)\) between the joint approximate posterior and prior decomposes as
\[
\begin{aligned}
(**)
&= \sum_{c=1}^K
    \mathbb{E}_{\mathbf{Z} \sim q_\phi(\cdot, c \mid \mathcal{D}_T)}
    \log\left(
        \frac{p(c \mid \mathbf{Z})\,p(\mathbf{Z})}{
            q_{\phi_z}(\mathbf{Z} \mid \mathcal{D}_T)\, q_{\phi_c}(c \mid \mathcal{D}_T)
        }
    \right) \\[1.5ex]
&= \sum_{c=1}^K
    \mathbb{E}_{\mathbf{Z} \sim q_\phi(\cdot, c \mid \mathcal{D}_T)}
    \log\left(
        \frac{p(\mathbf{Z})}{q_{\phi_z}(\mathbf{Z} \mid \mathcal{D}_T)}
    \right) \\[1.2ex]
&\hspace{2em}
+ \sum_{c=1}^K
    \mathbb{E}_{\mathbf{Z} \sim q_\phi(\cdot, c \mid \mathcal{D}_T)}
    \log\left(
        \frac{p(c \mid \mathbf{Z})}{q_{\phi_c}(c \mid \mathcal{D}_T)}
    \right) \\[1.5ex]
&= D_{KL}\bigl(
    q_{\phi_z}(\mathbf{z} \mid \mathcal{D}_T)\,\|\,p(\mathbf{z})
\bigr) \\[1.2ex]
&\hspace{2em}
+ \mathbb{E}_{\mathbf{Z} \sim q_{\phi_z}(\cdot \mid \mathcal{D}_T)}
    D_{KL}\bigl(
        q_{\phi_c}(c \mid \mathcal{D}_T)\,\|\,p(c \mid \mathbf{Z})
    \bigr).
\end{aligned}
\]

We define the individual ELBO by performing a weighted sum over log-likelihood terms and marginalizing over \(\mathcal{D}_T\):
\[
L = \sum_{t=1}^T
    \mathbb{E}_{\mathcal{D}_T}
    \bigl[
        \alpha(\mathbf{H}_t, W_t)\, \log p_\theta(Y_t \mid \mathbf{H}_t, W_t)
    \bigr]
\ge \mathbb{E}_{\mathcal{D}_T}
\underbrace{
    \sum_{t=1}^T
    \mathbb{E}_{\mathbf{Z}, C \sim q_\phi(\cdot,\cdot \mid \mathcal{D}_T)}
    \left[
        \alpha(\mathbf{h}_t, \omega_t)\,
        \log\frac{
            p_\theta(y_t, \mathbf{Z}, C \mid \mathbf{h}_t, \omega_t)
        }{
            q_\phi(\mathbf{Z}, C \mid \mathcal{D}_T)
        }
    \right]
}_{\mathrm{ELBO}_0(\mathcal{D}_T;\,\theta,\phi)}.
\]

Finally, \(\mathrm{ELBO}_0(\mathcal{D}_T; \theta,\phi)\) expands to
\[
\begin{aligned}
\mathrm{ELBO}_0(\mathcal{D}_T; \theta,\phi)
&= \sum_{t=1}^T
    \mathbb{E}_{\mathbf{Z} \sim q_{\phi_z}(\cdot \mid \mathcal{D}_T)}
    \bigl[
        \alpha(\mathbf{h}_t,\omega_t)\,
        \log p_\theta(y_t \mid \mathbf{h}_t,\omega_t,\mathbf{Z})
    \bigr] \\[1.5ex]
&\hspace{1em}
- \left(\sum_{t=1}^T \alpha(\mathbf{h}_t,\omega_t)\right)
\Biggl\{
    D_{KL}\bigl(
        q_{\phi_z}(\mathbf{z} \mid \mathcal{D}_T)\,\|\,p(\mathbf{z})
    \bigr) \\[1.2ex]
&\hspace{5em}
+ \mathbb{E}_{\mathbf{Z} \sim q_{\phi_z}(\cdot \mid \mathcal{D}_T)}
    D_{KL}\bigl(
        q_{\phi_c}(c \mid \mathcal{D}_T)\,\|\,p(c \mid \mathbf{Z})
    \bigr)
\Biggr\}.
\end{aligned}
\]
The gap in our variational approximation is defined as the difference between the true weighted log-likelihood and the ELBO:
\begin{equation*}
    \mathbb{E}_{\mathcal{D}_T}\Delta_0(\mathcal{D}_T; \theta, \phi) \coloneqq L - \mathbb{E}_{\mathcal{D}_T}\mathrm{ELBO_0}(\mathcal{D}_T; \theta, \phi)
\end{equation*}

The per-time-step gap in Eq. (\ref{eq:elbo_step}) can be rewritten as:
\begin{align*}
\log p_\theta\left(y_{t} \mid \mathbf{h}_{t}, \omega_t\right) - (*) &= \mathbb{E}_{\mathbf{Z}, C \sim q_{\phi}(\cdot , \cdot \mid \mathcal{D}_T)}  \left[ 
\log \frac{
p_\theta\left(y_{t} \mid \mathbf{h}_{t}, \omega_t\right)q_{\phi}(\mathbf{Z}, C \mid \mathcal{D}_T)
}{
p_\theta\left(y_{t}, \mathbf{Z}, C\mid \mathbf{h}_{t}, \omega_{t}\right) 
}
\right] \\
&= \mathbb{E}_{\mathbf{Z}, C \sim q_{\phi}(\cdot , \cdot \mid \mathcal{D}_T)}
\left[ 
\log \frac{
q_{\phi}(\mathbf{Z}, C \mid \mathcal{D}_T)
}{
p_\theta\left(\mathbf{Z}, C\mid \mathcal{D}_t\right) 
}
\right] \\
&= D_{KL}\left(q_{\phi}(\mathbf{Z}, C \mid \mathcal{D}_T) \parallel p_\theta\left(\mathbf{Z}, C\mid \mathcal{D}_t\right) \right)
\end{align*}

This last equation holds because 
\[
p_\theta\left(y_{t}, \mathbf{Z}, C \mid \mathbf{h}_{t}, \omega_{t}\right) = p_\theta\left(\mathbf{Z}, C \mid y_{t}, \mathbf{h}_{t}, \omega_{t}\right) p_\theta\left(y_{t} \mid \mathbf{h}_{t}, \omega_{t}\right),
\]
and \(\{y_{t}, \mathbf{h}_{t}, \omega_{t}\} = \{y_{\leq t}, \mathbf{x}_{\leq t}, \omega_{\leq t}\} = \mathcal{D}_t\). The individual gap is thus:
\[
\Delta_0(\mathcal{D}_T; \theta, \phi) = \sum_{t = 1}^{T} \alpha(\mathbf{h}_t, \omega_t) D_{KL}\left(q_{\phi}(\mathbf{Z}, C \mid \mathcal{D}_T) \parallel p_\theta\left(\mathbf{Z}, C\mid \mathcal{D}_t\right) \right)
\]
\end{proof}
\subsection{Transfer of Ignorability under Invertible Maps}
\label{appendix:proof_ignorability_invsersion}
\begin{proposition}
Let \(\Phi\) be an invertible representation function. Then, \(Y_{t}(\omega) \indep W_{t}| \Phi(\mathbf{H}_{t})\) holds if and only if \(Y_{t}(\omega) \indep W_{t}| \mathbf{H}_{t}\). Moreover, \(p(W_t=\omega|\Phi(\mathbf{h}_{t}))>0\) holds if and only if \(p(W_t=\omega|\mathbf{h}_{t})>0\).
\end{proposition}
\begin{proof}
    Assume \(Y_t(\omega) \indep W_t \mid \mathbf{H}_t\). For a non-invertible \(\Phi\), let
\(\Phi^{-1}(\mathbf{r}) = \{\mathbf{h}_t : \Phi(\mathbf{h}_t) = \mathbf{r}\}\). Then
\[
\begin{aligned}
p(Y_t(\omega)\mid \omega_t, \mathbf{r})
&= \frac{
    \displaystyle\int_{\mathbf{h}_t \in \Phi^{-1}(\mathbf{r})}
    p(Y_t(\omega)\mid \omega_t, \mathbf{h}_t)\,p(\mathbf{h}_t\mid \omega_t)\,d\mathbf{h}_t
}{
    \displaystyle\int_{\mathbf{h}_t \in \Phi^{-1}(\mathbf{r})}
    p(\mathbf{h}_t\mid \omega_t)\,d\mathbf{h}_t
} \\[2.0ex]
&= \frac{
    \displaystyle\int_{\mathbf{h}_t \in \Phi^{-1}(\mathbf{r})}
    p(Y_t(\omega)\mid \mathbf{h}_t)\,p(\mathbf{h}_t\mid \omega_t)\,d\mathbf{h}_t
}{
    \displaystyle\int_{\mathbf{h}_t \in \Phi^{-1}(\mathbf{r})}
    p(\mathbf{h}_t\mid \omega_t)\,d\mathbf{h}_t
},
\end{aligned}
\]
where ignorability implies that for general \(\Phi\),
\[
p(Y_t(\omega)\mid \omega_t, \mathbf{r})
\ne p(Y_t(\omega)\mid \mathbf{r}).
\]

For an invertible \(\Phi\), however,
\[
p(Y_t(\omega)\mid \omega_t, \Phi(\mathbf{h}_t)) = p(Y_t(\omega)\mid \Phi(\mathbf{h}_t)),
\]
and similarly,
\[
p(W_t=\omega \mid \Phi(\mathbf{h}_t)) = p(W_t=\omega \mid \mathbf{h}_t).
\]
\end{proof}

\subsection{CDVAE in the Near-Deterministic Regime}
\label{appendix:proof_cdvae_near_det}
\begin{proof}[Theorem \ref{thm:vaes_to_truell}]
\textbf{Part 1}: $lim_{s \to + \infty} p_{\theta_s}(y_{\leq T} \mid \mathbf{x}_{\leq T}, \omega_{\leq T}) = p(y_{\leq T} \mid \mathbf{x}_{\leq T}, \omega_{\leq T})$.

Define the conditional cumulative distribution function (CDF) of the response given covariates, for each $t$ as:
\[
F_t(y_t \mid \mathbf{h}_t, \omega_t) = \int_{- \infty}^{y_t} p(y_t' \mid \mathbf{h}_t, \omega_t ) dy_t'.
\]
Define the mapping \( F: \mathcal{Y}^{T} \to [0,1]^T \) as:
\[
F(y_1, \dots, y_T \mid \mathbf{x}_{\leq T}, \omega_{\leq T}) \coloneqq \left[F_1(y_1 \mid \mathbf{h}_1, \omega_1), \dots, F_T(y_T \mid \mathbf{h}_T, \omega_T)\right].
\]

The differential of the mapping is given by:
\[
dF(y_1, \dots, y_T \mid \mathbf{x}_{\leq T}, \omega_{\leq T}) = p(y_{\leq T} \mid \mathbf{x}_{\leq T}, \omega_{\leq T}) dy_{\leq T}.
\]

Now, define the following mapping for the latent variables using the Darmois construction \citep{hyvarinen1999nonlinear}:
\[
G_i(z_i \mid z_1, \dots, z_{i-1}) = \int_{- \infty}^{z_i} p(z_i' \mid z_1, \dots, z_{i-1}) dz_i'.
\]
We then define the mapping \( G: \mathbb{R}^{d_{\mathbf{z}}} \to [0,1]^T \) such that:
\[
G(\mathbf{z}) \coloneqq [G_1(z_1), G_2(z_2 \mid z_1), \dots, G_i(z_{\mathbf{z}} \mid z_1, \dots, z_{d_{\mathbf{z}}-1})].
\]
Since \(d_{\mathbf{z}} \le T\) by assumption, we can trivially augment the mapping \(G\) to \(\widetilde{G}\) so that its image lies in \([0,1]^T\). That is,
\[
\widetilde{G} : \mathbb{R}^{d_{\mathbf{z}}} \to [0,1]^T, \quad
\widetilde{G}(\mathbf{z}) \coloneqq
\bigl[G(\mathbf{z}),\,\underbrace{0,\dots,0}_{T - d_{\mathbf{z}}}\,\bigr].
\]
The differential is then given by
\[
d\widetilde{G}(\mathbf{z}) = p(\mathbf{z})\,d\mathbf{z}.
\]
We now define the mean and variance of the encoder as follows:
\[
f_t(\mathbf{h}_t, \omega_t, \mathbf{z}; \theta_{s}^*) \coloneqq [F^{-1}(\Tilde{G}(\mathbf{z}) \mid \mathbf{x}_{\leq T}, \omega_{\leq T})]_t, \quad \sigma_{s}^* = \frac{1}{\sqrt{s}}.
\]
There is a consistency issue to address with this definition. First, observe that the function $f_t(.; \theta_{s}^*)$ takes as input only data up to time step $t$, but the inverse of the cumulative CDF is defined given \textit{the whole sequence} of $(\mathbf{x}_{\leq T}, \omega_{\leq T})$. We therefore need to verify the following lemma which holds for our definition of $f_t(.; \theta_{s}^*)$.
\begin{lemma}
Let \((y_{\le T}, \mathbf{x}_{\le T}, \omega_{\le T})\) and
\((y_{\le T}', \mathbf{x}_{\le T}', \omega_{\le T}')\) be two distinct realizations of repeated measurements such that there exists \(t_0\) for which
\[
\mathbf{x}_{\le t_0} = \mathbf{x}_{\le t_0}', \quad
\omega_{\le t_0} = \omega_{\le t_0}'.
\]
Then, for every \(t \le t_0\),
\[
\bigl[F^{-1}(\widetilde{G}(\mathbf{z}) \mid \mathbf{x}_{\le t}, \omega_{\le t})\bigr]_t
= \bigl[F^{-1}(\widetilde{G}(\mathbf{z}) \mid \mathbf{x}_{\le t}', \omega_{\le t}')\bigr]_t.
\]
\end{lemma}
Now, we decompose the marginal probabilistic model:
\begin{equation*}
    \begin{split}
        p_{\theta_s}(y_{\leq T} \mid \mathbf{x}_{\leq T}, \omega_{\leq T}) &= \int_{\mathbb{R}^{d_{\mathbf{z}}}} p_{\theta_s}(y_{\leq T}, \mathbf{z} \mid \mathbf{x}_{\leq T}, \omega_{\leq T}) d\mathbf{z} \\
        &= \int_{\mathbb{R}^{d_{\mathbf{z}}}} \prod_{t=1}^T p_{\theta_s}(y_{t}, \mathbf{z} \mid y_{<t}, \mathbf{x}_{\leq t}, \omega_{\leq t}) p(\mathbf{z}) d\mathbf{z} \\
        &= \int_{\mathbb{R}^{d_{\mathbf{z}}}} \prod_{t=1}^T \mathcal{N}\left( y_t \mid [F^{-1}(\Tilde{G}(\mathbf{z}) \mid \mathbf{x}_{\leq T}, \omega_{\leq T})]_t, (\sigma_{s}^*)^2 \right) p(\mathbf{z}) d\mathbf{z} \\
        &= \int_{[0,1]^{T}} \prod_{t=1}^T \mathcal{N}\left( y_t \mid [F^{-1}(\xi \mid \mathbf{x}_{\leq T}, \omega_{\leq T})]_t, (\sigma_{s}^*)^2 \right) d\mathbf{\xi}\\
        &= \int_{\mathcal{Y}^{T}} \prod_{t=1}^T \mathcal{N}\left( y_t \mid [y_{\leq T}']_t, (\sigma_{s}^*)^2 \right) p(y_{\leq T}' \mid \mathbf{x}_{\leq T}', \omega_{\leq T}') dy_{\leq T}'.
    \end{split}
\end{equation*}
Finally, we have
\[
\begin{aligned}
\lim_{s \to +\infty} \int_{\mathcal{Y}^T}
&\prod_{t=1}^T \mathcal{N}\bigl(y_t \mid [y_{\le T}']_t, (\sigma_s^*)^2\bigr)\,
p(y_{\le T}' \mid \mathbf{x}_{\le T}', \omega_{\le T}')\,dy_{\le T}' \\[1.8ex]
&= \int_{\mathcal{Y}^T}
    \prod_{t=1}^T \delta(y_t - y_t')\,
    p(y_{\le T}' \mid \mathbf{x}_{\le T}', \omega_{\le T}')\,dy_{\le T}' \\[1.8ex]
&= p(y_{\le T} \mid \mathbf{x}_{\le T}, \omega_{\le T}).
\end{aligned}
\]
\textbf{Part 2}: Proof of $\lim_{s \to + \infty}  \Delta(\mathcal{D}_T; \theta_{s}, \phi_{s}) = 0$. \\
First, we give an explicit writing of the modified individual gap: 
\begin{equation*}
    \begin{split}
        \Delta(\mathcal{D}_T; \theta_{s}, \phi_{s}) &= L(\mathcal{D}_T; \theta_{s}, \phi_{s}) - \mathrm{ELBO_0}(\mathcal{D}_T; \theta_{s}, \phi_{s}) +  \mathrm{ELBO_0}(\mathcal{D}_T; \theta_{s}, \phi_{s}) - \mathrm{ELBO}(\mathcal{D}_T; \theta_{s}, \phi_{s}) \\
        &= \Delta_0(\mathcal{D}_T; \theta_{s}, \phi_{s}) +  \mathrm{ELBO_0}(\mathcal{D}_T; \theta_{s}, \phi_{s}) - \mathrm{ELBO}(\mathcal{D}_T; \theta_{s}, \phi_{s}) \\
        &\quad - \left[\sum_{t = 1}^{T}\alpha(\mathbf{h}_t, \omega_t)\right] \mathbb{E}_{\mathbf{Z} \sim q_{\phi_s}(\cdot \mid \mathcal{D}_T)} D_{KL}(q_{\phi_s}(c \mid \mathcal{D}_T) \parallel p(c \mid \mathbf{Z})) \\
        &\quad - \left[\sum_{t = 1}^{T}\alpha_s(\mathbf{h}_t, \omega_t)\right]\log Z(q_{\phi_s}(\cdot \mid \mathcal{D}_T)) \\
        &= \sum_{t = 1}^{T} \alpha(\mathbf{h}_t, \omega_t) D_{KL}(q_{\phi_s}(\mathbf{z}, c \mid \mathcal{D}_T) \parallel p_{\theta_s}(\mathbf{z}, c \mid \mathcal{D}_t)).
    \end{split}
\end{equation*}

The last equality holds because we assume $q_{\phi_s}(c \mid \mathcal{D}_T) = \pi_{\phi_s}(c \mid \mathcal{D}_T)$ and $\pi_{\phi_s}(c \mid \mathcal{D}_T)$ is a minimizer of 
\[
\min_{q_{\phi_s}(c \mid \mathcal{D}_T)} \mathbb{E}_{\mathbf{Z} \sim q_{\phi_s}(\cdot \mid \mathcal{D}_T)} D_{KL}(q_{\phi_s}(c \mid \mathcal{D}_T) \parallel p(c \mid \mathbf{Z})) = -\log Z(q_{\phi_s}(\cdot \mid \mathcal{D}_T)).
\]

To show that $\lim_{s \to + \infty}  \Delta(\mathcal{D}_T; \theta_{s}, \phi_{s}) = 0$, we will define $\phi_{s}$ such that for every $c \in \{1, \dots, K\}$ and \(t \in \{1, \dots, T\}\):
\[
\lim_{s \to + \infty} D_{KL}(q_{\phi_{s}}(\mathbf{z}, c \mid \mathcal{D}_T) \parallel p_{\theta_s}(\mathbf{z}, c \mid \mathcal{D}_t)) = 0.
\]

Let us define $q_{\phi_{s}}( \mathbf{z} \mid \mathcal{D}_T)$ such that 
\[
f_{\mu_{\mathbf{z}}}(\mathcal{D}_T, \phi_{s}) = G^{-1}(F(y_1, \dots, y_{d_{\mathbf{z}}}] \mid \mathbf{x}_{\leq T}, \omega_{\leq T}))
\]
and 
\[
f_{S_{\mathbf{z}}}(\mathcal{D}_T, \phi) = \sigma_{s} \sqrt{\tilde{\Sigma}_{\mathbf{z}}(\mathcal{D}_T, \phi)},
\]
with $\tilde{\Sigma}_{\mathbf{z}}(\mathcal{D}_T, \phi)$ being the inverse of:
\[
\mathrm{Jac}(F^{-1}(. \mid \mathbf{x}_{\leq T}, \omega_{\leq T}) \circ \tilde{G}(\mathbf{z}))\mathrm{Jac}(F^{-1}(. \mid \mathbf{x}_{\leq T}, \omega_{\leq T}) \circ \tilde{G}(\mathbf{z}))^{\top}.
\]

Using Bayes’ rule, the true posterior can be written as
\[
p_{\theta_s}\bigl(\mathbf{z}, c \mid \mathcal{D}_t\bigr)
= \frac{
    p_{\theta_s}\bigl(y_{\le T}, \mathbf{z}, c \mid \mathbf{x}_{\le t}, \omega_{\le t}\bigr)
}{
    p_{\theta_s}\bigl(y_{\le t} \mid \mathbf{x}_{\le t}, \omega_{\le t}\bigr)
}.
\]
Expanding the numerator, we obtain
\[
\begin{aligned}
p_{\theta_s}\bigl(\mathbf{z}, c \mid \mathcal{D}_t\bigr)
&= \frac{
    \displaystyle\prod_{l=1}^t \mathcal{N}\bigl(
        y_l \mid
        [F^{-1}(\widetilde{G}(\mathbf{z}) \mid \mathbf{x}_{\le T}, \omega_{\le T})]_l,
        \sigma_s^2
    \bigr)\, p(\mathbf{z}\mid c)\,p(c)
}{
    p_{\theta_s}\bigl(y_{\le t} \mid \mathbf{x}_{\le t}, \omega_{\le t}\bigr)
}.
\end{aligned}
\]

By the GMM assumption over the prior, we have
\[
p(\mathbf{z} \mid c) = \mathcal{N}(\mathbf{z} \mid \mu_c, \Sigma_c).
\]

The approximate posterior is of the form
\[
\begin{aligned}
q_{\phi_s}\bigl(\mathbf{z}, c \mid \mathcal{D}_T\bigr)
&= q_{\phi_s}\bigl(\mathbf{z} \mid \mathcal{D}_T\bigr)\,\pi_{\phi_s}\bigl(c \mid \mathcal{D}_T\bigr) \\[1.2ex]
&= \mathcal{N}\bigl(
    \mathbf{z} \mid
    f_{\mu_{\mathbf{z}}}(\mathcal{D}_T, \phi_s),
    \sigma_s^2\,\widetilde{\Sigma}_{\mathbf{z}}(\mathcal{D}_T, \phi)
\bigr)\,\pi_{\phi_s}\bigl(c \mid \mathcal{D}_T\bigr).
\end{aligned}
\]
We now show convergence by performing a change of variables. Define $\mathbf{z}^{\prime} = \sigma_{s}^{-\frac{t}{d_z}}(\mathbf{z} - \mathbf{z}^*)$. We analyze the behavior of the distributions $p_{\theta_{s}}^{\prime}(\mathbf{z}^{\prime}, c \mid \mathcal{D}_t)$ and $q_{\phi_{s}}^{\prime}(\mathbf{z}^{\prime}, c \mid \mathcal{D}_T)$. 

We prove that
\[
\frac{p_{\theta_{s}}^{\prime}(\mathbf{z}^{\prime}, c \mid \mathcal{D}_t)}{q_{\phi_{s}}^{\prime}(\mathbf{z}^{\prime}, c \mid \mathcal{D}_T)}
\]
converges to a constant independent of $\mathbf{z}^{\prime}$ as $s \to \infty$. Since both $q_{\phi_s}^{\prime}(\mathbf{z}^{\prime}, c \mid \mathcal{D}_T)$ and $p_{\theta_s}^{\prime}(\mathbf{z}^{\prime}, c \mid \mathcal{D}_t)$ are probability distributions, the constant must be 1. Therefore, the KL divergence between them converges to 0 as $s \to \infty$.

We have
\[
\begin{aligned}
\frac{
p_{\theta_s}'(\mathbf{z}', c \mid \mathcal{D}_t)
}{
q_{\phi_s}'(\mathbf{z}', c \mid \mathcal{D}_T)
}
&= \frac{
    \mathcal{N}\bigl(
        \mathbf{z}^* + \sigma_s^{t/d_z}\mathbf{z}'
        \,\big|\,
        \mathbf{z}^*,\, \sigma_s^2\,\widetilde{\Sigma}_{\mathbf{z}}(\mathcal{D}_T, \phi)
    \bigr)\,
    \pi_{\phi_s}(c \mid \mathcal{D}_T)\,
    p_{\theta_s}\bigl(y_{\le t} \mid \mathbf{x}_{\le t}, \omega_{\le T}\bigr)
}{
    \displaystyle\prod_{l=1}^t
    \mathcal{N}\bigl(
        y_l \mid f_l(\mathbf{h}_l, \omega_l, \mathbf{z}^* + \sigma_s^{t/d_z}\mathbf{z}'; \theta_s),\, \sigma_s^2
    \bigr) \,
    \mathcal{N}\bigl(
        \mathbf{z}^* + \sigma_s^{t/d_z}\mathbf{z}' \mid \mu_c, \Sigma_c
    \bigr)\,p(c)
}.
\end{aligned}
\]

Now let \(A_t\) be a matrix whose Moore–Penrose inverse \(A^+\) satisfies
\[
\begin{aligned}
f_{\le t}(\mathbf{h}_{\le t}, \omega_{\le t}, \mathbf{z}^* + \sigma_s^{t/d_z}\mathbf{z}'; \theta_s)
&= A^+ f_{\le T}(\mathbf{h}_{\le T}, \omega_{\le T}, \mathbf{z}^* + \sigma_s^{t/d_z}\mathbf{z}'; \theta_s), \\[1.2ex]
y_{\le t} &= A^+ y_{\le T}.
\end{aligned}
\]
That is, projecting onto \(A^+\) selects the first \(t\) responses. The matrices \(A^+\) and \(A\) have the forms
\[
A^+ =
\begin{bmatrix}
I_t & 0_{t \times (T - t)}
\end{bmatrix}, \quad
A =
\begin{bmatrix}
I_t \\[0.8ex]
0_{(T - t) \times t}
\end{bmatrix}.
\]
By noticing that \([A^{\intercal}(\sigma_s^2I_T)^{-1}A]^{-1} = \sigma_s^2I_t\) We can therefore apply the mean rearranging formula \citep{Petersen2008MatCookbook}: 
\begin{align*}
&\mathcal{N}\left(
    A^+y_{\leq T} \,\middle|\, 
    A^+f_{\leq T}(\mathbf{h}_{\leq t}, \omega_{\leq t}, \mathbf{z}^* + \sigma_{s}^{\frac{t}{d_z}} \mathbf{z}^{\prime}; \theta_{s}), 
    \left[A^{\intercal}(\sigma_s^2 I_T) A\right]^{-1}
\right) \\
&\quad = 
\frac{
    \sqrt{\det(2\pi \sigma_s^2 I_T)}
}{
    \sqrt{\det(2\pi \sigma_s^2 I_t)}
}
\mathcal{N}\left(
    y_{\leq T} \,\middle|\, 
    f_{\leq T}(\mathbf{h}_{\leq T}, \omega_{\leq T}, \mathbf{z}^* + \sigma_{s}^{\frac{t}{d_z}} \mathbf{z}^{\prime}; \theta_{s}), 
    \sigma_s^2 I_T
\right)
\end{align*}
\begin{align*}
\frac{
p_{\theta_s}'\bigl(\mathbf{z}', c \mid \mathcal{D}_t\bigr)
}{
q_{\phi_s}'\bigl(\mathbf{z}', c \mid \mathcal{D}_T\bigr)
}
&= \frac{
    \mathcal{N}\bigl(
        \mathbf{z}^* + \sigma_s^{t/d_z}\mathbf{z}'
        \mid \mathbf{z}^*,\, \sigma_s^2\,\widetilde{\Sigma}_{\mathbf{z}}(\mathcal{D}_T, \phi)
    \bigr)\,
    \pi_{\phi_s}\bigl(c \mid \mathcal{D}_T\bigr)\,
    p_{\theta_s}\bigl(y_{\le t} \mid \mathbf{x}_{\le t}, \omega_{\le T}\bigr)
}{
    \displaystyle
    \frac{\sqrt{\det(2\pi\sigma_s^2I_T)}}{\sqrt{\det(2\pi\sigma_s^2I_t)}}
    \mathcal{N}\bigl(
        y_{\le T} \mid
        f_{\le T}(\mathbf{h}_{\le T}, \omega_{\le T}, \mathbf{z}^* + \sigma_s^{t/d_z}\mathbf{z}'; \theta_s),
        \sigma_s^2I_T
    \bigr)\,
    \mathcal{N}\bigl(
        \mathbf{z}^* + \sigma_s^{t/d_z}\mathbf{z}' \mid \mu_c, \Sigma_c
    \bigr)\,p(c)
} \\[2.0ex]
&= (2\pi)^{\tfrac{t-d}{2}}\,
\frac{
    \det\bigl(\widetilde{\Sigma}_{\mathbf{z}}\bigr)^{-1/2}
}{
    \det(\Sigma_c)^{-1/2}
}
\exp\Bigg\{
    -\tfrac{1}{2}\sigma_s^{2(t/d_z - 1)}{\mathbf{z}'}^\top\widetilde{\Sigma}_{\mathbf{z}}^{-1}\mathbf{z}' \\[1.4ex]
&\qquad
    + \tfrac{1}{2\sigma_s^2}\sum_{l=1}^T
    \bigl(y_l - f_l(\mathbf{h}_l, \omega_l, \mathbf{z}^* + \sigma_s^{t/d_z}\mathbf{z}'; \theta_s)\bigr)^2 \\[1.4ex]
&\qquad
    + \tfrac{1}{2}\bigl(\mathbf{z}^* + \sigma_s^{t/d_z}\mathbf{z}' - \mu_c\bigr)^\top
    \Sigma_c^{-1}\bigl(\mathbf{z}^* + \sigma_s^{t/d_z}\mathbf{z}' - \mu_c\bigr)
\Bigg\} \\[1.8ex]
&\quad \times \frac{
    \pi_{\phi_s}\bigl(c \mid \mathcal{D}_T\bigr)\,
    p_{\theta_s}\bigl(y_{\le T} \mid \mathbf{x}_{\le t}, \omega_{\le t}\bigr)
}{
    p(c)
}.
\end{align*}
By noticing that
\[
\sum_{l=1}^{T}\bigl(y_l - f_l(\mathbf{h}_l, \omega_l, \mathbf{z}^* + \sigma_s^{t/d_z}\mathbf{z}'; \theta_s)\bigr)^2
= \bigl\| y_{\le T} - F^{-1}\bigl(\widetilde{G}(\mathbf{z}^* + \sigma_s^{t/d_z}\mathbf{z}') \mid \mathbf{x}_{\le T}, \omega_{\le T}\bigr)\bigr\|_2^2.
\]

We apply a first-order Taylor expansion:
\[
y_{\le T} - F^{-1}\bigl(\widetilde{G}(\mathbf{z}^* + \sigma_s^{t/d_z}\mathbf{z}') \mid \mathbf{x}_{\le T}, \omega_{\le T}\bigr)
\underset{s \to \infty}{\approx}
-Jac\bigl(F^{-1}\widetilde{G}\bigr)(\mathbf{z}^*)\bigl(\sigma_s^{t/d_z}\mathbf{z}'\bigr),
\]
which implies by norm continuity
\[
\begin{aligned}
\sum_{l=1}^T\bigl(y_l - f_l(\mathbf{h}_l, \omega_l, \mathbf{z}^* + \sigma_s^{t/d_z}\mathbf{z}'; \theta_s)\bigr)^2
&\underset{s \to \infty}{\approx}
\bigl\|Jac(F^{-1}\widetilde{G})(\mathbf{z}^*)\bigl(\sigma_s^{t/d_z}\mathbf{z}'\bigr)\bigr\|_2^2 \\[1.2ex]
&\underset{s \to \infty}{=}
\sigma_s^{2t/d_z}\,\mathbf{z}'^\top\widetilde{\Sigma}_{\mathbf{z}}^{-1}\mathbf{z}'.
\end{aligned}
\]

Define the constant \(\mathcal{C}\mathrm{st}(\mathcal{D}_t; \sigma_s, \theta_s, \phi_s)\) w.r.t. \(\mathbf{z}'\) as
\[
\mathcal{C}\mathrm{st}(\mathcal{D}_t; \sigma_s, \theta_s, \phi_s)
= (2\pi)^{(t-d_z)/2}
\sqrt{\frac{\det(\Sigma_c)}{\det(\widetilde{\Sigma}_{\mathbf{z}})}}
\frac{\pi_{\phi_s}(c \mid \mathcal{D}_T)\,p_{\theta_s}\bigl(y_{\le t} \mid \mathbf{x}_{\le t}, \omega_{\le t}\bigr)}{p(c)}.
\]

Thus,
\[
\begin{aligned}
\frac{p_{\theta_s}'(\mathbf{z}', c \mid \mathcal{D}_T)}{q_{\phi_s}'(\mathbf{z}', c \mid \mathcal{D}_T)}
&\underset{s \to \infty}{\approx}
\tfrac{1}{2}(\mathbf{z}^* - \mu_c)^\top\Sigma_c^{-1}(\mathbf{z}^* - \mu_c)\,\mathcal{C}\mathrm{st}(\mathcal{D}_t; \sigma_s, \theta_s, \phi_s) \\[1.4ex]
&\quad\times
\exp\Bigg\{
    -\tfrac{1}{2}\sigma_s^{2(t/d_z - 1)}\mathbf{z}'^\top\widetilde{\Sigma}_{\mathbf{z}}^{-1}\mathbf{z}'
    + \tfrac{1}{2}\sigma_s^{2(t/d_z - 1)}\mathbf{z}'^\top\mathbf{z}'
\Bigg\}.
\end{aligned}
\]

Finally,
\[
\frac{p_{\theta_s}'(\mathbf{z}', c \mid \mathcal{D}_T)}{q_{\phi_s}'(\mathbf{z}', c \mid \mathcal{D}_T)}
\underset{s \to \infty}{\approx}
\tfrac{1}{2}(\mathbf{z}^* - \mu_c)^\top\Sigma_c^{-1}(\mathbf{z}^* - \mu_c)\,\mathcal{C}\mathrm{st}(\mathcal{D}_t; \sigma_s, \theta_s, \phi_s).
\]

To conclude the proof, we still need to show that 
\(\lim_{s \to +\infty} \mathcal{C}\mathrm{st}(\mathcal{D}_t; \sigma_s, \theta_s, \phi_s)\) exists and is finite because the model parameters still depend on the chosen variance.  This was the main misapprehension of \cite{dai2018diagnosingvae} for a VAE in the static setting with an unimodal prior over the continuous latents \(\mathbf{Z}\).

We have already shown that 
\[
\lim_{\sigma \to 0^+} p_{\theta_{\sigma}}(y_{\leq T} \mid \mathbf{x}_{\leq T}, \omega_{\leq T}) = p(y_{\leq T} \mid \mathbf{x}_{\leq T}, \omega_{\leq T}),
\]
and therefore:
\[
\begin{aligned}
\lim_{s \to +\infty}\mathcal{C}\mathrm{st}(\mathcal{D}_t; \sigma_s, \theta_s, \phi_s)
&=
(2\pi)^{(t - d_z)/2}
\sqrt{\frac{\det(\Sigma_c)}{\det(\widetilde{\Sigma}_{\mathbf{z}})}} \\[1.2ex]
&\quad\times
\frac{p(y_{\le T} \mid \mathbf{x}_{\le T}, \omega_{\le T})}{p(c)}
\cdot
\lim_{s \to +\infty}\pi_{\phi_s}(c \mid \mathcal{D}_T).
\end{aligned}
\]

We verify that \(\lim_{s \to +\infty} \pi_{\phi_{s}}(c \mid \mathcal{D}_T)\) exists and is finite and not zero for all \(c \in \{1, \dots, K\}\):
\begin{align*}
\pi_{\phi_{s}}(c \mid \mathcal{D}_T)
&= \frac{\exp(\mathbb{E}_{\mathbf{Z} \sim q_{\phi_z}(\cdot \mid \mathcal{D}_T)} \log p(c \mid \mathbf{Z}))
    }{
    \sum_{c=1}^K \exp(\mathbb{E}_{\mathbf{Z} \sim q_{\phi_z}(\cdot \mid \mathcal{D}_T)} \log p(c \mid \mathbf{Z}))} \\
&= \frac{
                \exp(
                \int_{\mathcal{Z}} \log p(c\mid\mathbf{z}) \mathcal{N}\left(
        \mathbf{z} \mid \mathbf{z}^*,         
         \sigma_{s}^{2}  \tilde{\Sigma}_{\mathbf{z}}(\mathcal{D}_T, \phi) 
        \right)  d\mathbf{z}
                )
                }{
                \sum_{c=1}^K \exp(
                \int_{\mathcal{Z}} \log p(c\mid\mathbf{z}) \mathcal{N}\left(
        \mathbf{z} \mid \mathbf{z}^*,         
         \sigma_{s}^{2}  \tilde{\Sigma}_{\mathbf{z}}(\mathcal{D}_T, \phi) 
        \right)  d\mathbf{z}
                )
                } \\
&\underset{s \to \infty}{\to} \frac{
                \exp(
                \int_{\mathcal{Z}} \log p(c\mid\mathbf{z}) \delta(\mathbf{z} - \mathbf{z}^*)  d\mathbf{z}
                )
                }{
                \sum_{c=1}^K \exp(
                \int_{\mathcal{Z}} \log p(c\mid\mathbf{z})  \delta(\mathbf{z} - \mathbf{z}^*)  d\mathbf{z}
                )
                } \\
&= \frac{
                 p(c\mid\mathbf{z}^*)
                }{
                \sum_{c=1}^K  p(c\mid\mathbf{z}^*)
                } 
\end{align*}
We have therefore proved that the ratio \(\frac{p_{\theta_{s}}^{\prime}\left(\mathbf{z}^{\prime}, c \mid \mathcal{D}_T\right)}{q_{\phi_{s}}^{\prime}(\mathbf{z}^{\prime}, c \mid \mathcal{D}_T)} \)  converges into a nonzero constant which finishes the proof of the theorem.
\end{proof}

\paragraph{Proof of theorem \ref{thm:sigma_to_0}.} We start by considering the ELBO:
\begin{equation*}
\begin{split}
    \mathcal{L}(\mathcal{D}_T; \theta, \phi) 
    &=  -\sum_{t = 1}^{T} \mathbb{E}_{\mathbf{Z} \sim q_{\phi}(\cdot \mid \mathcal{D}_T)} 
    \left[ \alpha(\mathbf{h}_t, \omega_t) \log p_{\theta}(y_{t} \mid \mathbf{H}_t, W_t, \mathbf{Z}) \right] \\
    &\quad + \left[\sum_{t = 1}^{T}\alpha(\mathbf{h}_t, \omega_t)\right] D_{KL}\left(q_{\phi}(\mathbf{z} \mid \mathcal{D}_T) \parallel p(\mathbf{z})\right) \\
    &\quad - \left[\sum_{t = 1}^{T}\alpha(\mathbf{h}_t, \omega_t)\right] \log Z(q_{\phi}(\cdot \mid \mathcal{D}_T)).
\end{split}
\end{equation*}

By the positivity of the KL divergence and using the fact that $-\log Z(q_{\phi}(\cdot \mid \mathcal{D}_T))$ minimizes a positive functional (as explained in Eq.~\eqref{eq:min_VaDE_trick}), we obtain:
\begin{equation*}
\begin{split}
    \mathcal{L}(\mathcal{D}_T; \theta_{\sigma}^*, \phi_{\sigma}^*) 
    &\geq  -\sum_{t = 1}^{T} \mathbb{E}_{\mathbf{Z} \sim q_{\phi}(\cdot \mid \mathcal{D}_T)} 
    \left[ 
        \alpha(\mathbf{h}_t, \omega_t) \log \left( p_{\theta}\left( y_{t} \mid \mathbf{H}_t, W_t, \mathbf{Z} \right) \right) 
    \right] \\
    &= \sum_{t = 1}^{T} \alpha(\mathbf{h}_t, \omega_t) \mathbb{E}_{\mathbf{Z} \sim q_{\phi}(\cdot \mid \mathcal{D}_T)} 
    \left[
        \frac{1}{2} \log\left( 2 \pi \sigma^2 \right) + \frac{1}{2\sigma^2} \left( y_t - f\left( \mathbf{H}_t, \mathbf{Z}, W_t \right) \right)^2
    \right] \\
    &= \frac{1}{2\sigma^2} 
    \left[
        \left( \sum_{t = 1}^{T} \alpha(\mathbf{h}_t, \omega_t) \right) \sigma^2 \log\left( 2 \pi \sigma^2 \right) 
        + \sum_{t = 1}^{T} \alpha(\mathbf{h}_t, \omega_t) \underbrace{\mathbb{E}_{\mathbf{Z} \sim q_{\phi}(\cdot \mid \mathcal{D}_T)} 
        \left( y_t - f\left( \mathbf{H}_t, \mathbf{Z}, W_t \right) \right)^2}_{\delta_{\sigma}(t)}  
    \right].
\end{split}
\end{equation*}

Suppose there exists $t_0 \in \{1,2,\ldots, T\}$ such that $\lim_{\sigma \to 0^+} \delta_{\sigma}(t_0) > 0$. Then we have $\lim_{\sigma \to 0^+} \mathcal{L}(\mathcal{D}_T; \theta_{\sigma}^*, \phi_{\sigma}^*) = +\infty$, which is impossible since we assume $\mathcal{L}(\mathcal{D}_T; \theta_{\sigma}^*, \phi_{\sigma}^*)$ to be minimized. Therefore, we conclude that for all $t \in \{1,2,\ldots, T\}$, $\lim_{\sigma \to 0^+} \delta_{\sigma}(t) = 0$.

Consequently, we have
\begin{equation*}
\lim_{\sigma \to 0^+} \mathbb{E}_{\mathbf{\epsilon} \sim \mathcal{N}(0,I)} 
        \left( y_t - f\left( \mathbf{H}_t, W_t, f_{\mu_{\mathbf{z}}}(\mathcal{D}_T; \phi_{\sigma}^*)+ f_{S_{\mathbf{z}}}(\mathcal{D}_T; \theta_{\sigma}^*)\mathbf{\epsilon} \right) \right)^2 = 0,
\end{equation*}
which implies that 
\[
\lim_{\sigma \to 0^+} f\left( \mathbf{H}_t, W_t, f_{\mu_{\mathbf{z}}}(\mathcal{D}_T; \phi_{\sigma}^*) + f_{S_{\mathbf{z}}}(\mathcal{D}_T; \theta_{\sigma}^*)\mathbf{\epsilon} \right) = y_t, \quad \text{almost surely}.
\]
In particular, we also have
\[
\lim_{\sigma \to 0^+} f\left( \mathbf{H}_t, W_t, f_{\mu_{\mathbf{z}}}(\mathcal{D}_T; \phi_{\sigma}^*) \right) = y_t.
\]

\subsection{Upper bound on weighted PEHE}
\label{appendix:up_bound_wpehe}
\begin{proof}[\textbf{theorem} \ref{thm:pehe_wbound}]
To prove the theorem, we rely on the following key lemma, but first, we need to define further mathematical objects. We define the weighted population risk over the whole population as
\[
R_{t, g}(f, \Phi) \coloneqq \mathbb{E}_{\mathbf{H}_t, W_t} \left[ \alpha(\mathbf{H}_t, W_t) \, \ell_{f, \Phi}(\mathbf{H}_t, W_t)  \right],
\]
and the weighted population counterfactual risk as 
\[
R_{t, g}(f, \Phi)_{CF} \coloneqq \mathbb{E}_{\mathbf{H}_t, 1-W_t} \left[ \alpha(\mathbf{H}_t, 1-W_t) \, \ell_{f, \Phi}(\mathbf{H}_t, W_t)  \right].
\]
\begin{lemma}
\label{lemma:Upbound_cfrisk_byFactual} $R_{t, g}(f, \Phi) + R_{t, g}(f, \Phi)_{CF} \leq R_{t, g}^1(f, \Phi) + R_{t, g}^0(f, \Phi) +  B_{\Phi} \, \mathrm{IPM}_{G} \left( g_{\Phi}(\cdot \mid W_t = 1), \, g_{\Phi}(\cdot \mid W_t = 0) \right)$
\end{lemma}
The proof immediately follows from Lemma 1 in \cite{shalit2017estimating}.

Next, to complete the proof, we define the expected potential outcome at time $t$, given the context history $\mathbf{H}_{t} = \mathbf{h}_{t}$ and latent $\mathbf{z}$ as
\[
m_{t}^{\omega}(\mathbf{h}_{t}, \mathbf{z}) \coloneqq \mathbb{E}_{Y_{t}(\omega) \mid \mathbf{H}_{t},\mathbf{Z} }(Y_{t}(\omega) \mid \mathbf{H}_{t} = \mathbf{h}_{t}, \mathbf{Z} =  \mathbf{z}) \quad \omega \in \mathcal{W},
\]
and we show the following lemma:
\begin{lemma}
\label{lemma:mean_estim_err_decomp}
Denote \(\hat{p}_{\phi}(\mathbf{h}_t, w, \mathbf{z}) \coloneqq p(\mathbf{h}_t, w)\, q_{\phi}(\mathbf{z} \mid \mathcal{D}_{\leq t-1})\). We can decompose \(R_{t,g}(f,\Phi)\) and \(R_{t,g}(f,\Phi)_{\mathrm{CF}}\) under our distributional assumptions as:
\[
\begin{aligned}
&\mathbb{E}_{\hat{p}_{\phi}(\mathbf{h}_t, w, \mathbf{z})} 
\bigl[ \alpha(\mathbf{h}_t, w)\,\big(f(\mathbf{h}_t, w, \mathbf{z}) - m_{t}^{w}(\mathbf{h}_t, \mathbf{z})\big) \bigr] \\[1.2ex]
&\quad= 2\sigma^2 \left( R_{t,g}(f,\Phi) - \tfrac{1}{2}\log(2\pi\sigma^2) \right)
- \sum_{\omega \in \{0,1\}}\mathrm{Var}_{\hat{p}_{\phi}}(Y_t),
\end{aligned}
\]
and
\[
\begin{aligned}
&\mathbb{E}_{\hat{p}_{\phi}(\mathbf{h}_t, w, \mathbf{z})}
\bigl[ \alpha(\mathbf{h}_t, 1-w)\,\big(f(\mathbf{h}_t, 1-w, \mathbf{z}) - m_{t}^{1-w}(\mathbf{h}_t, \mathbf{z})\big) \bigr] \\[1.2ex]
&\quad= 2\sigma^2 \left( R_{t,g}(f,\Phi)_{\mathrm{CF}} - \tfrac{1}{2}\log(2\pi\sigma^2) \right)
- \sum_{\omega \in \{0,1\}}\mathrm{Var}_{\hat{p}_{\phi}}(Y_t\mid 1-w).
\end{aligned}
\]
\end{lemma}
\begin{proof}
We have: 
\begin{small}
\begin{align*}
R_{t,g}(f,\Phi)
&= \mathbb{E}_{\mathbf{H}_t,W_t} \!\left[ \alpha(\mathbf{H}_t,W_t)\,\ell_{f,\Phi}(\mathbf{H}_t,W_t) \right] \\[1.2ex]
&= \sum_{\omega\in\{0,1\}} \int_{\mathcal{H}_t}\!\!\int_{\mathcal{Z}}\!\!\int_{\mathcal{Y}} 
-\alpha(\mathbf{h}_t,\omega)\log p_\theta(y_t\mid\mathbf{h}_t,\omega,\mathbf{z})\\[-0.5ex]
&\hspace{4em}\times p(y_t\mid\mathbf{h}_t,\omega,\mathbf{z})\,p(\mathbf{h}_t,\omega)\,q_\phi(\mathbf{z}\mid\mathcal{D}_{\le t-1})
\,dy_t\,d\mathbf{z}\,d\mathbf{h}_t \\[1.5ex]
&= \sum_{\omega\in\{0,1\}} \int_{\mathcal{H}_t}\!\!\int_{\mathcal{Z}}\!\!\int_{\mathcal{Y}} 
\alpha(\mathbf{h}_t,\omega)\Bigg\{ 
\tfrac{1}{2}\log(2\pi\sigma^2) + \frac{(y_t-f(\mathbf{h}_t,\omega,\mathbf{z}))^2}{2\sigma^2} 
\Bigg\}\\[-0.5ex]
&\hspace{4em}\times p(y_t\mid\mathbf{h}_t,\omega,\mathbf{z})\,p(\mathbf{h}_t,\omega)\,q_\phi(\mathbf{z}\mid\mathcal{D}_{\le t-1})
\,dy_t\,d\mathbf{z}\,d\mathbf{h}_t \\[1.5ex]
&= \tfrac{1}{2}\log(2\pi\sigma^2)
+ \frac{1}{2\sigma^2} \sum_{\omega\in\{0,1\}} 
\mathrm{Var}_{\hat{p}_\phi(\mathbf{h}_t,\omega,\mathbf{z})}(Y_t)\\[-0.5ex]
&\quad+\int_{\mathcal{H}_t}\!\!\int_{\mathcal{Z}} 
\alpha(\mathbf{h}_t,\omega)\left( f(\mathbf{h}_t,\omega,\mathbf{z}) - m_t^\omega(\mathbf{h}_t,\mathbf{z}) \right)^2\\[-0.5ex]
&\hspace{4em}\times p(\mathbf{h}_t,\omega)\,q_\phi(\mathbf{z}\mid\mathcal{D}_{\le t-1})
\,d\mathbf{z}\,d\mathbf{h}_t.
\end{align*}
\end{small}
 
In a similar way, we can show the decomposition related to $R_{t, g}(f, \Phi) _{CF}$.
\end{proof}
The remainder idea of the proof is to decompose the PEHE in such a way we can upper bound it with an expression including $R_{t, g}(f, \Phi)$ and $R_{t, g}(f, \Phi)_{CF}$ and then use lemma \ref{lemma:Upbound_cfrisk_byFactual}. We actually have:
\begin{small}
\begin{align*}
\epsilon_{\mathrm{PEHE}_{t, g}} 
&= \mathbb{E}_{\mathbf{H}_t \sim g}\,\mathbb{E}_{\mathbf{Z} \sim q_\phi(\mathbf{Z}\mid\mathcal{D}_{\le t-1})} 
\bigl[\bigl(\tau(\mathbf{H}_t,\mathbf{Z}) - \hat{\tau}_{f,\Phi}(\mathbf{H}_t,\mathbf{Z})\bigr)^2\bigr] \\[1.2ex]
&= \mathbb{E}_{\mathbf{H}_t \sim g}\,\mathbb{E}_{\mathbf{Z} \sim q_\phi(\mathbf{Z}\mid\mathcal{D}_{\le t-1})}
\bigl[ \bigl(m_t^1(\mathbf{h}_t,\mathbf{z}) - m_t^0(\mathbf{h}_t,\mathbf{z}) - f(\mathbf{h}_t,1,\mathbf{z}) + f(\mathbf{h}_t,0,\mathbf{z})\bigr)^2 \bigr] \\[1.5ex]
&\overset{(1)}{\le} 2\,\mathbb{E}_{\mathbf{H}_t \sim g}\,\mathbb{E}_{\mathbf{Z} \sim q_\phi(\mathbf{Z}\mid\mathcal{D}_{\le t-1})}
\bigl[ (f(\mathbf{h}_t,1,\mathbf{z}) - m_t^1(\mathbf{h}_t,\mathbf{z}))^2 \bigr] \\[-0.5ex]
&\quad + 2\,\mathbb{E}_{\mathbf{H}_t \sim g}\,\mathbb{E}_{\mathbf{Z} \sim q_\phi(\mathbf{Z}\mid\mathcal{D}_{\le t-1})}
\bigl[ (f(\mathbf{h}_t,0,\mathbf{z}) - m_t^0(\mathbf{h}_t,\mathbf{z}))^2 \bigr] \\[1.5ex]
&= \mathbb{E}_{\mathbf{H}_t \mid W_t=1}\,\mathbb{E}_{\mathbf{Z}}\!\bigl[\alpha(\mathbf{h}_t,1)\,(f(\mathbf{h}_t,1,\mathbf{z})-m_t^1(\mathbf{h}_t,\mathbf{z}))^2\bigr] \\[-0.5ex]
&\quad + \mathbb{E}_{\mathbf{H}_t \mid W_t=0}\,\mathbb{E}_{\mathbf{Z}}\!\bigl[\alpha(\mathbf{h}_t,0)\,(f(\mathbf{h}_t,1,\mathbf{z})-m_t^1(\mathbf{h}_t,\mathbf{z}))^2\bigr] \\[-0.5ex]
&\quad + \mathbb{E}_{\mathbf{H}_t \mid W_t=0}\,\mathbb{E}_{\mathbf{Z}}\!\bigl[\alpha(\mathbf{h}_t,0)\,(f(\mathbf{h}_t,0,\mathbf{z})-m_t^0(\mathbf{h}_t,\mathbf{z}))^2\bigr] \\[-0.5ex]
&\quad + \mathbb{E}_{\mathbf{H}_t \mid W_t=1}\,\mathbb{E}_{\mathbf{Z}}\!\bigl[\alpha(\mathbf{h}_t,1)\,(f(\mathbf{h}_t,0,\mathbf{z})-m_t^0(\mathbf{h}_t,\mathbf{z}))^2\bigr] \\[1.5ex]
&= \mathbb{E}_{\mathbf{H}_t,W_t}\,\mathbb{E}_{\mathbf{Z}}
\bigl[\alpha(\mathbf{H}_t,W_t)\,(f(\mathbf{H}_t,W_t,\mathbf{Z})-m_t^{W_t}(\mathbf{H}_t,\mathbf{Z}))^2\bigr] \\[-0.5ex]
&\quad + \mathbb{E}_{\mathbf{H}_t,1-W_t}\,\mathbb{E}_{\mathbf{Z}}
\bigl[\alpha(\mathbf{H}_t,1-W_t)\,(f(\mathbf{H}_t,W_t,\mathbf{Z})-m_t^{W_t}(\mathbf{H}_t,\mathbf{Z}))^2\bigr] \\[1.5ex]
&\overset{(2)}{=} 2\sigma^2\bigl(R_{t,g}(f,\Phi)+R_{t,g}(f,\Phi)_{\mathrm{CF}}-\log(2\pi\sigma^2)\bigr)\\[-0.5ex]
&\quad - \sum_{\omega\in\{0,1\}}\!\bigl(\mathrm{Var}_{\hat{p}_\phi(\mathbf{h}_t,1-\omega,\mathbf{z})}(Y_t) + \mathrm{Var}_{\hat{p}_\phi(\mathbf{h}_t,\omega,\mathbf{z})}(Y_t)\bigr) \\[1.5ex]
&\overset{(3)}{\le} 2\sigma^2\bigl(R_{t,g}(f,\Phi)+R_{t,g}(f,\Phi)_{\mathrm{CF}}-\log(2\pi\sigma^2)\bigr) \\[1.5ex]
&\overset{(4)}{\le} 2\sigma^2\biggl(R_{t,g}^1(f,\Phi)+R_{t,g}^0(f,\Phi)
+B_\Phi\,\mathrm{IPM}_G\bigl(g_\Phi(\cdot|W_t=1),g_\Phi(\cdot|W_t=0)\bigr)
-\log(2\pi\sigma^2)\biggr).
\end{align*}
\end{small}

The inequality $\overset{(1)}{\leq }$ follows from the property $(a-b)^2 \leq 2a^2 + 2b^2$. The equation $\overset{(2)}{=}$ follows from plugging in the equations from Lemma \ref{lemma:mean_estim_err_decomp}, the inequality $\overset{(3)}{\leq}$ follows from the positivity of the variance terms, and $\overset{(4)}{\leq}$ follows from Lemma \ref{lemma:Upbound_cfrisk_byFactual}.
\end{proof}

\subsection{Proof of Proposition \ref{prop:approx_factual_risk}}
\label{appendix:proof_statio}
Using a Monte Carlo approximation, we can express the approximate factual risk as:
\[
R^{\omega}_{t, g}\left(f, \Phi \right) \approx \frac{1}{n_{\omega}^{(t)}} \sum_{i \in \mathcal{B}, W_{it} = \omega } \mathbb{E}_{\mathbf{Z} \sim q_{\phi}(\mathbf{Z} \mid \mathcal{D}_{i, \leq t-1})} \left[ 
 \alpha(\mathbf{h}_{it}, \omega) \log \mathcal{N}(y_{it}; f(\Phi(\mathbf{h}_{it}),\mathbf{Z}, \omega), \sigma^2) 
\right].
\]
By the stationarity assumption, for \( t \geq t_0 \), this approximation holds:
\[
R^{\omega}_{t, g}\left(f, \Phi \right) \approx \frac{1}{n_{\omega}^{(t)}} \sum_{i \in \mathcal{B}, W_{it} = \omega } \mathbb{E}_{\mathbf{Z} \sim q_{\phi}(\mathbf{Z} \mid \mathcal{D}_{iT})} \left[ 
 \alpha(\mathbf{h}_{it}, \omega) \log \mathcal{N}(y_{it}; f(\Phi(\mathbf{h}_{it}),\mathbf{Z}, \omega), \sigma^2) 
\right].
\]

On the other hand, the reconstruction term in the ELBO can be written as:
\begin{align*}
&\sum_{t = t_0}^{T} 
\mathbb{E}_{\mathbf{Z} \sim q_{\phi}(\cdot \mid \mathcal{D}_T)} 
\bigl[ \alpha(\mathbf{H}_t, W_t)\,\log p_{\theta}(Y_t \mid \mathbf{H}_t, W_t, \mathbf{Z}) \bigr] \\[1.2ex]
&\quad\approx \sum_{t = t_0}^{T} 
\frac{1}{|\mathcal{B}|} 
\sum_{i \in \mathcal{B}} 
\mathbb{E}_{\mathbf{Z} \sim q_{\phi}(\mathbf{Z} \mid \mathcal{D}_{iT})}
\biggl[
\alpha(\mathbf{h}_{it}, \omega)\,
\log\mathcal{N}\bigl(y_{it};\, f(\Phi(\mathbf{h}_{it}),\mathbf{Z},\omega),\, \sigma^2\bigr)
\biggr] \\[1.5ex]
&\quad\approx \frac{1}{|\mathcal{B}|} 
\sum_{t = t_0}^{T}
\sum_{\omega \in \mathcal{W}}
\sum_{i \in \mathcal{B},\, W_{it}=\omega} 
\mathbb{E}_{\mathbf{Z} \sim q_{\phi}(\mathbf{Z} \mid \mathcal{D}_{iT})}
\biggl[
\alpha(\mathbf{h}_{it}, \omega)\,
\log\mathcal{N}\bigl(y_{it};\, f(\Phi(\mathbf{h}_{it}),\mathbf{Z},\omega),\, \sigma^2\bigr)
\biggr] \\[1.5ex]
&\quad\approx \frac{1}{|\mathcal{B}|}
\sum_{t = t_0}^{T} 
\biggl\{-n_1^{(t)}\,R_t^1(f,\Phi)\;-\;n_0^{(t)}\,R_t^0(f,\Phi)\biggr\}.
\end{align*}

\section{Experiments on synthetic data: Details} 

\subsection{Additional results}
\label{appendix_cdvae:arsim_extended_results}
\paragraph{Results of baselines on the synthetic datasets} The following Table \ref{tab:perf_sim_combined} provides the detailed results responsible for Figures \ref{fig:perf_sim_combined} related to baselines with the three different approaches across levels of \(\gamma_{(1)}^{YU}\).
\begin{table}[!htbp]
 \caption{Results on the synthetic data reported by PEHE. Smaller is better.}
 \centering
\resizebox{\textwidth}{!}{%
\begin{tabular}{|c|c|c|c|c|c|c|c|c|c|c|c|} 
\hline
Model       & $\gamma_{(1)}^{YU} = 0$ & $\gamma_{(1)}^{YU} = 0.25$ & $\gamma_{(1)}^{YU} = 0.5$ & $\gamma_{(1)}^{YU} = 0.75$ & $\gamma_{(1)}^{YU} = 1$ & $\gamma_{(1)}^{YU} = 1.25$ & $\gamma_{(1)}^{YU} = 1.5$ & $\gamma_{(1)}^{YU} = 1.75$ & $\gamma_{(1)}^{YU} = 2$ & $\gamma_{(1)}^{YU} = 2.25$ & $\gamma_{(1)}^{YU} = 2.5$ \\ \hline 

\textbf{CDVAE (ours)} & \textbf{0.43$\pm$0.02}& \textbf{0.50$\pm$0.03}& \textbf{0.96$\pm$0.09}& \textbf{1.57$\pm$0.08}& \textbf{1.90$\pm$0.10}&  \textbf{2.35$\pm$0.18}& \textbf{3.57$\pm$0.17}& \textbf{4.80$\pm$0.20}& \textbf{6.84$\pm$0.20}& \textbf{7.64$\pm$0.48}& \textbf{9.03$\pm$0.50}\\
\hline

\textbf{Causal CPC} & 0.43$\pm$0.01 & 0.50$\pm$0.03 & 1.08$\pm$0.08 & 2.49$\pm$0.14 & 2.98$\pm$0.09 & 4.98$\pm$0.21 & 5.91$\pm$0.29 & 10.15$\pm$0.38 & 12.25$\pm$0.49 & 15.65$\pm$0.56 & 19.39$\pm$0.59 \\

\textbf{Causal CPC (with substitute)} & 0.46$\pm$0.02 & 0.49$\pm$0.01 & 1.02$\pm$0.05 & 2.38$\pm$0.08 & 2.83$\pm$0.09 & 4.81$\pm$0.13 & 5.38$\pm$0.22 & 8.13$\pm$0.39 & 10.11$\pm$0.41 & 12.01$\pm$0.54 & 14.03$\pm$0.64 \\

\textbf{Causal CPC (oracle)} & 0.45$\pm$0.02 & 0.43$\pm$0.03 & 0.96$\pm$0.04 & 1.59$\pm$0.06 & 2.14$\pm$0.08 & 4.41$\pm$0.10 & 5.08$\pm$0.30 & 6.93$\pm$0.25 & 8.70$\pm$0.17 & 10.15$\pm$0.47 & 12.91$\pm$0.51 \\
\hline
 
\textbf{Causal Transformer} & 0.46$\pm$0.02 & 0.68$\pm$0.04 & 1.50$\pm$0.06 & 2.55$\pm$0.18& 3.65$\pm$0.20& 5.55$\pm$0.50& 8.15$\pm$0.72& 12.35$\pm$0.25& 15.48$\pm$1.02& 24.77$\pm$2.21& 43.84$\pm$2.58\\

\textbf{Causal Transformer (with substitute)} &  0.46$\pm$0.02 & 0.67$\pm$0.02& 1.46$\pm$0.03& 2.48$\pm$0.08& 3.53$\pm$0.09& 5.23$\pm$0.11& 7.72$\pm$0.18& 11.86$\pm$0.17& 15.22$\pm$0.17& 20.12$\pm$0.35& 33.58$\pm$0.45\\

\textbf{Causal Transformer (oracle)} & 0.46$\pm$0.02&  0.60$\pm$0.03 & 1.48$\pm$0.03 & 2.35$\pm$ 0.06& 3.30$\pm$0.07& 5.11$\pm$0.09& 7.34$\pm$0.13& 11.55$\pm$0.25& 16.98$\pm$0.29& 18.64$\pm$0.31& 28.45$\pm$0.33\\

 \hline
\textbf{G-Net} & 0.62$\pm$0.05&  0.80$\pm$0.05& 4.90$\pm$0.03& 5.56$\pm$0.05& 4.82$\pm$0.15& 5.79$\pm$0.12& 10.36$\pm$0.23& 15.17$\pm$0.25& 23.89$\pm$0.54& 32.75$\pm$1.20& 49.35$\pm$2.35\\

\textbf{G-Net (with substitute)} & 0.56$\pm$0.04&  0.75$\pm$0.01& 3.61$\pm$0.02& 4.99$\pm$0.20& 4.27$\pm$0.18& 5.50$\pm$0.15& 8.34$\pm$0.64& 13.55$\pm$0.97& 17.97$\pm$1.83& 19.25$\pm$2.04& 40.21$\pm$2.10\\

\textbf{G-Net (oracle)} & 0.48$\pm$0.02& 0.69$\pm$0.03& 3.10$\pm$0.05& 4.36$\pm$0.08& 4.45$\pm$0.12& 5.28$\pm$0.17& 8.28$\pm$0.23& 13.10$\pm$0.50& 17.47$\pm$0.65& 16.22$\pm$0.95& 35.35$\pm$1.77\\
 \hline

\textbf{CRN} & 0.53$\pm$0.02& 0.68$\pm$0.03& 1.63$\pm$0.04& 2.94$\pm$0.11& 5.14$\pm$0.17& 6.66$\pm$0.19& 9.08$\pm$0.25& 11.93$\pm$0.37& 16.54$\pm$0.65& 18.68$\pm$0.67& 29.66$\pm$1.12\\

\textbf{CRN (with substitute)} & 0.48$\pm$0.01& 0.65$\pm$0.01& 1.51$\pm$0.02& 2.56$\pm$0.18 & 3.98$\pm$0.21 & 6.05$\pm$0.35 & 6.81$\pm$0.65 & 8.50$\pm$1.16 & 13.81$\pm$0.76 & 16.23$\pm$0.73 & 26.11$\pm$1.41 \\

\textbf{CRN (oracle)} & 0.53$\pm$0.01& 0.60$\pm$0.01& 1.69$\pm$0.02& 2.87$\pm$0.09& 3.75$\pm$0.13& 5.69$\pm$0.17& 8.92$\pm$0.22& 9.65$\pm$0.31& 13.49$\pm$0.54& 15.64$\pm$0.61& 25.98$\pm$0.97\\

 \hline
\textbf{RMSN} & 0.57$\pm$0.02& 0.67$\pm$0.02& 1.60$\pm$0.03& 2.67$\pm$0.05& 4.31$\pm$0.15& 5.58$\pm$0.17& 7.40$\pm$0.32& 11.25$\pm$0.57& 15.01$\pm$0.89& 19.41$\pm$1.13& 25.07$\pm$0.97\\

\textbf{RMSN (with substitute)} & 0.45$\pm$0.01& 0.67$\pm$0.02& 1.51$\pm$0.04 & 2.31$\pm$0.03& 3.61$\pm$0.20& 4.61$\pm$0.20& 6.14$\pm$0.50& 7.58$\pm$0.82& 10.63$\pm$1.31& 18.53$\pm$1.50& 21.08$\pm$1.60\\

\textbf{RMSN (oracle)} & 0.48$\pm$0.01& 0.62$\pm$0.01& 1.43$\pm$0.03& 1.97$\pm$0.03& 3.42$\pm$0.13& 4.43$\pm$0.15& 6.00$\pm$0.27& 7.31$\pm$0.34& 9.20$\pm$0.48& 17.06$\pm$0.83& 19.32$\pm$1.26\\
 \hline
 \end{tabular}%
}
\label{tab:perf_sim_combined}
\end{table}

\paragraph{Robustness to Number of Prior Components} The Table \ref{tab:ablation_arsim_n_clusters} gives detailed results summarized in Figure \ref{fig:ablation_arsim_n_clusters} that assess the sensitivity of CDVAE to the variation of the prior cluster numbers \(K\). 
\begin{table}[!htbp]
 \caption{Results of CDVAE when varying the number of components \(K\) of the prior. The study is conducted on the synthetic data and is reported by PEHE. Smaller is better.}
 \centering
\resizebox{\textwidth}{!}{%
\begin{tabular}{|c|c|c|c|c|c|c|c|c|c|c|c|} 
\hline
Model       & $\gamma_{(1)}^{YU} = 0$ & $\gamma_{(1)}^{YU} = 0.25$ & $\gamma_{(1)}^{YU} = 0.5$ & $\gamma_{(1)}^{YU} = 0.75$ & $\gamma_{(1)}^{YU} = 1$ & $\gamma_{(1)}^{YU} = 1.25$ & $\gamma_{(1)}^{YU} = 1.5$ & $\gamma_{(1)}^{YU} = 1.75$ & $\gamma_{(1)}^{YU} = 2$ & $\gamma_{(1)}^{YU} = 2.25$ & $\gamma_{(1)}^{YU} = 2.5$ \\ \hline 

\textbf{CDVAE (ours)} & \textbf{0.43$\pm$0.02}& \textbf{0.50$\pm$0.03}& \textbf{0.96$\pm$0.09}& \textbf{1.57$\pm$0.08}& \textbf{1.90$\pm$0.10}&  \textbf{2.35$\pm$0.18}& \textbf{3.57$\pm$0.17}& \textbf{4.80$\pm$0.20}& \textbf{6.84$\pm$0.20}& \textbf{7.64$\pm$0.48}& \textbf{9.03$\pm$0.50}\\
 \hline
  \textbf{CDVAE ($K=2$)}& 0.43$\pm$0.01& 0.50$\pm$0.01& 0.96$\pm$0.03& 1.52$\pm$0.04& 2.07$\pm$0.07& 2.51$\pm$0.14& 4.10$\pm$0.41& 4.44$\pm$0.43& 6.98$\pm$0.38& 7.90$\pm$0.33& 8.88$\pm$0.45\\ \hline

 \textbf{CDVAE ($K=5$)}& 0.42$\pm$0.01& 0.48$\pm$0.02& 0.93$\pm$0.02& 1.41$\pm$0.11& 2.02$\pm$0.03& 2.52$\pm$0.06& 3.27$\pm$0.22& 4.25$\pm$0.45& 6.32$\pm$0.25& 7.97$\pm$0.31&8.12$\pm$0.48\\\hline
 
 \textbf{CDVAE ($K=8$)}& 0.40$\pm$0.01& 0.46$\pm$0.01& 0.96$\pm$0.06& 1.57$\pm$0.03& 2.13$\pm$0.04& 2.59$\pm$0.07& 3.20$\pm$0.26& 4.15$\pm$0.45& 6.63$\pm$0.48& 6.93$\pm$0.25&8.91$\pm$0.19\\\hline
 
 \textbf{CDVAE ($K=11$)}& 0.42$\pm$0.02& 0.47$\pm$0.01& 0.94$\pm$0.03& 1.40$\pm$0.05& 2.09$\pm$0.07& 2.47$\pm$0.22& 3.76$\pm$0.28& 5.09$\pm$0.52& 6.48$\pm$0.14& 7.73$\pm$1.232& 9.02$\pm$1.22\\\hline

 \end{tabular}%
}
\label{tab:ablation_arsim_n_clusters}
\end{table}

\section{Experiments on MIMIC-III data}

\subsection{Additional results}
\label{appendix_cdvae:mimic_extended_results}
\paragraph{Results of baselines on the semi-synthetic MIMIC III} The following Table \ref{tab:perf_mimic} provides the detailed results responsible for Figures \ref{fig:perf_mimic} related to baselines with the three different approaches.
\begin{table}[!htbp]
 \caption{Results on the MIMIC III data reported by PEHE. Smaller is better.}
 \centering
\resizebox{0.4\textwidth}{!}{%
\begin{tabular}{|c|c|} 
\hline
Model      & $\mathrm{PEHE}$ \\ \hline 
\textbf{CDVAE (ours)} & \textbf{17.63$\pm$0.25}\\
\hline
\textbf{Causal CPC} & 19.27$\pm$0.25\\
\textbf{Causal CPC (with substitute)} & 18.45$\pm$0.26\\
\textbf{Causal CPC (oracle)} & 17.98$\pm$0.21\\
 \hline
\textbf{Causal Transformer} & 19.68$\pm$0.20 $\pm$\\
\textbf{Causal Transformer (with substitute)} & 18.58$\pm$ 0.21 \\
\textbf{Causal Transformer (oracle)} & 17.91 $\pm$ 0.20 \\
 \hline
\textbf{G-Net} & 19.75$\pm$0.21 \\
\textbf{G-Net (with substitute)} & 18.60$\pm$0.25 \\
\textbf{G-Net (oracle)} & 17.95$\pm$ 0.23\\
 \hline
\textbf{CRN} & 19.80$\pm$0.23 \\
\textbf{CRN (with substitute)} & 18.58$\pm$0.22\\
\textbf{CRN (oracle)} & 17.91$\pm$ 0.21 \\
 \hline
\textbf{RMSN} & 19.85$\pm$0.25 \\
\textbf{RMSN (with substitute)} &  18.66$\pm$0.23\\
\textbf{RMSN (oracle)} & 18.01$\pm$ 0.19 \\
 \hline
 \end{tabular}%
}
\label{tab:perf_mimic}
\end{table}

\section{Models hyperparameters Details} 
\label{appendix_cdvae:hyperparams_details}
We report in the following tables the search space of hyperparameters for all baselines.

\begin{table}[!htbp]
\centering
\caption{Hyper-parameters search range for RMSN}
\resizebox{0.9\textwidth}{!}{%
\begin{tabular}{|c|c|c|c|c|}
\hline
\textbf{Model} & \textbf{Sub-model} & \textbf{Hyperparameter} & \textbf{Synthetic data}& \textbf{MIMIC III}\\
\hline
\multirow{7}{*}{RMSNs} 
& \multirow{7}{*}{Propensity Treatment Network} 
& LSTM layers & 1 & 1 \\
\cline{3-5}
& & Learning rate & $0.01, 0.005, 0.001, 0.0001$ & $0.01, 0.005, 0.001, 0.0001$ \\
\cline{3-5}
& & Batch size & $32, 64, 128$ & $32, 64, 128$ \\
\cline{3-5}
& & LSTM hidden units & $6, 8, \dots, 12,14$& $4, 6, \dots, 20$\\
\cline{3-5}
& & LSTM dropout rate & - & - \\
\cline{3-5}
& & Max gradient norm & $0.5, 1, 2$ & $0.5, 1, 2$ \\
\cline{3-5}
& & Early Stopping (min delta) & 0.001& 0.001\\
\cline{3-5}
& & Early Stopping (patience) & 10& 30 \\
\hline
&\multirow{6}{*}{Propensity History Network} & LSTM layers & 1 & 1 \\
\cline{3-5}
& & Learning rate & $0.01, 0.005, 0.001, 0.0001$ & $0.01, 0.005, 0.001, 0.0001$ \\
\cline{3-5}
& & Batch size & $32, 64, 128$ & $64, 128, 256$ \\
\cline{3-5}
& & LSTM hidden units & $6, 8, \dots, 12,14$& $4, 6, \dots, 30$ \\
\cline{3-5}
& & LSTM dropout rate & - & - \\
\cline{3-5}
& & Early Stopping (min delta) & 0.001& 0.0001 \\
\cline{3-5}
& & Early Stopping (patience) & 10& 30 \\
\hline
& \multirow{6}{*}{Encoder} & LSTM layers & 1 & 1 \\
\cline{3-5}
& & Learning rate & $0.01, 0.005, 0.001, 0.0001$ & $0.01, 0.005, 0.001, 0.0001$ \\
\cline{3-5}
& & Batch size & $32, 64, 128,256$& $32, 64, 128$ \\
\cline{3-5}
& & LSTM hidden units & $6, 8, \dots, 18,20$& $6, 8, \dots, 18,20$\\
\cline{3-5}
& & LSTM dropout rate & - & - \\
\cline{3-5}
& & Early Stopping (min delta) & 0.001& 0.001\\
\cline{3-5}
& & Early Stopping (patience) & 10& 30 \\
\hline
& \multirow{6}{*}{Decoder} & LSTM layers & 1 & 1 \\
\cline{3-5}
& & Learning rate & $0.01, 0.005, 0.001, 0.0001$ & $0.01, 0.005, 0.001, 0.0001$ \\
\cline{3-5}
& & Batch size & $32, 64, 128,256$& $128, 512, 1024$ \\
\cline{3-5}
& & LSTM hidden units & $6, 8, \dots, 18,20$& $6, 8, \dots, 18,20$\\
\cline{3-5}
& & LSTM dropout rate & - & - \\
\cline{3-5}
& & Max gradient norm & $0.5, 1, 2$ & $0.5, 1, 2$ \\
\cline{3-5}
& & Early Stopping (min delta) & 0.001& 0.0001 \\
\cline{3-5}
& & Early Stopping (patience) & 10& 30 \\
\hline
\end{tabular}%
}
\end{table}

\begin{table}[!htbp]
\centering
\caption{Hyper-parameters search range for CRN}
\resizebox{0.7\textwidth}{!}{%
\begin{tabular}{|c|c|c|c|c|}
\hline
\textbf{Model} & \textbf{Sub-model} & \textbf{Hyperparameter} & \textbf{Synthetic data}& \textbf{MIMIC III)}\\
\hline
\multirow{8}{*}{CRN} 
& \multirow{8}{*}{Encoder} 
& LSTM layers & 1 & 1 \\
\cline{3-5}
& & Learning rate & $0.01, 0.005, 0.001, 0.0001$ & $0.01, 0.005, 0.001, 0.0001$ \\
\cline{3-5}
& & Batch size & $32, 64, 128,256$& $32, 64, 128$ \\
\cline{3-5}
& & LSTM hidden units & $6, 8, \dots, 18,20$& $6, 8, \dots, 18,20$\\
\cline{3-5}
& & LSTM dropout rate & - & - \\
\cline{3-5}
& & BR size & $6, 8, \dots, 18,20$& $6, 8, \dots, 18,20$\\
\cline{3-5}
& & Early Stopping (min delta) & 0.001& 0.001\\
\cline{3-5}
& & Early Stopping (patience) & 10& 30 \\
\hline
&\multirow{7}{*}{Decoder} & LSTM layers & 1 & 1 \\
\cline{3-5}
& & Learning rate & $0.01, 0.005, 0.001, 0.0001$ & $0.01, 0.005, 0.001, 0.0001$ \\
\cline{3-5}
& & Batch size & $128, 256, 512$ & $256, 512, 1024$ \\
\cline{3-5}
& & LSTM hidden units & $6, 8, \dots, 18,20$& $6, 8, \dots, 18,20$\\
\cline{3-5}
& & LSTM dropout rate & - & - \\
\cline{3-5}
& & BR size & $6, 8, \dots, 18,20$& $6, 8, \dots, 18,20$\\
\cline{3-5}
& & Early Stopping (min delta) & 0.001& 0.001\\
\cline{3-5}
& & Early Stopping (patience) & 10& 30 \\
\hline
\end{tabular}%
}
\end{table}

\begin{table}[!htbp]
\centering
\caption{Hyper-parameters search range for G-Net}
\resizebox{0.7\textwidth}{!}{%
\begin{tabular}{|c|c|c|}
\hline
\textbf{Hyperparameter} & \textbf{Cancer simulation} & \textbf{MIMIC III (SS)} \\
\hline
LSTM layers & 1 & 1  \\
 %\cline{1-4}
Learning rate & $0.01,0.005, 0.001, 0.0001$ &  $0.01,0.005, 0.001, 0.0001$ \\
 % %\cline{1-4}
Batch size & $32, 64, 128$ &  $32, 64, 128$ \\
 %\cline{1-4}
LSTM hidden units & $6, 8, \dots, 18,20$ & $6, 8, \dots, 18,20$ \\
%\cline{1-4}
FC hidden units & $6, 8, \dots, 18,20$&  $6, 8, \dots, 18,20$ \\
 %\cline{1-4}
LSTM dropout rate & - & -  \\
 %\cline{1-4}
R size& $6, 8, \dots, 18,20$& $4,6, \dots, 30$ \\
 %\cline{1-4}
MC samples & 50 & 50 \\
Early Stopping (min delta)& 0.001&  0.001\\
Early Stopping (patience)& 10& 30 \\
\cline{1-3}
\end{tabular}%
}
\end{table}

\begin{table}[!htbp]
\centering
\caption{Hyper-parameters search range for Causal Transformer}
\resizebox{0.7\textwidth}{!}{%
\begin{tabular}{|c|c|c|}
\hline
\textbf{Hyperparameter} & \textbf{Cancer simulation} & \textbf{MIMIC III (SS)} \\
\hline
Transformer blocks & 1 & 1 \\
 %\cline{1-4}
Learning rate & $0.01,0.005, 0.001, 0.0001$ & $0.01,0.005, 0.001, 0.0001$  \\
 %\cline{1-4}
Batch size & $32, 64, 128$ & $32, 64, 128$ \\
 %\cline{1-4}
Attention heads & $2$ & $2$ \\
 %\cline{1-4}
Transformer units & $4,6, \dots, 20$& $4,6, \dots, 20$ \\
 %\cline{1-4}
LSTM dropout rate & -  & - \\
%\cline{1-4}
BR size& $6, 8, \dots, 18,20$&  $4,6, \dots, 20$ \\
%\cline{1-4}
FC hidden units & $6, 8, \dots, 18,20$&   $4,6, \dots, 20$ \\
Sequential dropout rate & $0.1,0.2, 0.3$& $0.1,0.2, 0.3$ \\
Max positional encoding & $15$& $20$  \\
Early Stopping (min delta)& 0.001& 0.001 \\
Early Stopping (patience)& 10& 30 \\
\cline{1-3}
\end{tabular}%
}
\end{table}

\begin{table}[!htbp]
\centering
\caption{Hyper-parameters search range for Causal CPC}
\resizebox{0.9\textwidth}{!}{%
\begin{tabular}{|c|c|c|c|c|}
\hline
\textbf{Model} & \textbf{Sub-model} & \textbf{Hyperparameter} & \textbf{Cancer simulation} & \textbf{MIMIC III (SS)} \\
\hline
\multirow{9}{*}{Causal CPC} & \multirow{9}{*}{Encoder} 
& GRU layers & 1 & 1 \\
\cline{3-5}
& & Learning rate & $0.01, 0.005, 0.001, 0.0001$ & $0.01, 0.005, 0.001, 0.0001$ \\
\cline{3-5}
& & Batch size & $32, 64, 128$ & $64, 128, 256$ \\
\cline{3-5}
& & GRU hidden units & $6, 8, \dots, 18,20$& $6, 8, \dots, 18,20$\\
\cline{3-5}
& & GRU dropout rate & - & - \\
\cline{3-5}
& & Local features (LF) size & $6, 8, \dots, 18,20$& $4, 6, \dots, 20$ \\
\cline{3-5}
& & Context Representation (CR) size & $6, 8, \dots, 18,20$& $4, 6, \dots, 20$ \\
\cline{3-5}
& & Early Stopping (min delta) & 0.001 & 0.001 \\
\cline{3-5}
& & Early Stopping (patience) & 10& 30\\
\hline
& \multirow{13}{*}{Decoder} & GRU layers & 1 & 1 \\
\cline{3-5}
& & Learning rate (decoder w/o treatment sub-network) & $0.01, 0.005, 0.001, 0.0001$ & $0.01, 0.005, 0.001, 0.0001$ \\
\cline{3-5}
& & Learning rate (encoder fine-tuning) & $0.001, 0.0005, 0.0001, 0.00005$ & $0.001, 0.0005, 0.0001, 0.00005$ \\
\cline{3-5}
& & Learning rate (treatment sub-network) & $0.05, 0.01, 0.005, 0.0001$ & $0.05, 0.01, 0.005, 0.0001$ \\
\cline{3-5}
& & Batch size & $32, 64, 128$ & $32, 64, 128$ \\
\cline{3-5}
& & GRU hidden units & CR size & CR size \\
\cline{3-5}
& & GRU dropout rate & - & - \\
\cline{3-5}
& & BR size & CR size & CR size \\
\cline{3-5}
& & GRU layers (Treat Encoder) & 1 & 1 \\
\cline{3-5}
& & GRU hidden units (Treat Encoder) & 6 & 6 \\
\cline{3-5}
& & FC hidden units & $6, 8, \dots, 18,20$& $4, 6, \dots, 20$ \\
\cline{3-5}
& & Random time indices (m) & 10\% & 10\% \\
\cline{3-5}
& & Early Stopping (min delta) & 0.001 & 0.001 \\
\cline{3-5}
& & Early Stopping (patience) & 10& 30\\
\hline
\end{tabular}%
}
\end{table}

\begin{table}[!htbp]
\centering
\caption{Hyper-parameters search range for CDVAE}
\resizebox{0.9\textwidth}{!}{%
\begin{tabular}{|c|c|c|c|c|}
\hline
\textbf{Model} & \textbf{Sub-model} & \textbf{Hyperparameter} & \textbf{Synthetic data}& \textbf{MIMIC III}\\
\hline
\multirow{7}{*}{CDVAE} 
& \multirow{4}{*}{Inference Network} & GRU layers & 1 & 1 \\
\cline{3-5}
& & GRU hidden units & $6, 8, \dots, 12,14$& $4, 6, \dots, 20$\\
\cline{3-5}
& & GRU dropout rate& - & - \\
\cline{3-5}
& & Latent dim of \(\mathbf{z}\) & 0.001& 0.001\\
\hline
& \multirow{1}{*}{Propensity Network} & FC hidden units & $6, 8, \dots, 12,14$& $4, 6, \dots, 30$ \\
\hline
& \multirow{4}{*}{Representation Learner} & LSTM layers & 1 & 1 \\
\cline{3-5}
& & GRU hidden units & $6, 8, \dots, 18,20$& $6, 8, \dots, 18,20$\\
\cline{3-5}
& & GRU dropout rate & - & - \\
\cline{3-5}
& & Dimension of representation & $6, 8, \dots, 18,20$& $4, 6, \dots, 20$ \\
\hline
& \multirow{1}{*}{Decoder} & FC hidden units & $(dim(\mathbf{z})+dim(\Phi(\mathbf{H}_t)) / 2$& $(dim(\mathbf{z})+dim(\Phi(\mathbf{H}_t)) / 2$\\
\hline
& \multirow{4}{*}{Global} & Learning rate (w/o propensity network) & $0.01, 0.005, 0.001, 0.0001$ & $0.01, 0.005, 0.001, 0.0001$ \\
\cline{3-5}
& & Learning rate (propensity network) & $0.01, 0.005, 0.001, 0.0001$ & $0.01, 0.005, 0.001, 0.0001$ \\
\cline{3-5}
& & Batch size & $32, 64, 128,256$& $128, 512, 1024$ \\
\cline{3-5}
& & Max gradient norm & $0.5, 1, 2$ & $0.5, 1, 2$ \\
\cline{3-5}
& & Number of components in Prior & $2, 4, \dots, 18, 20$& $2, 4, \dots, 20$ \\
\hline
\end{tabular}%
}
\end{table}

\section{The Neural Architecture of CDVAE}
\label{appendix_cdvae:extended_archi_CDVAE}
The extended neural architecture of CDVAE comprises multiple components which we did not explicit in Section \ref{sect_cdvae:CDVAE_archi}. We first begin by detailing neural network functions related to the generative model. The Table \ref{tab:archi_phi_rep_learner} outlines the architecture for the Representation Learner $\Phi$ which encodes the context history, Table \ref{tab:archi_f_theta} presents the identical architecture for both $f_{\theta_{y}^1}$ and $f_{\theta_{y}^0}$ responsible for generating the two potential outcomes. Meanwhile, Table \ref{tab:archi_e_theta} illustrates the design of propensity network $e_{\theta_{\omega}}(.)$ built on the top of the shared representation. Lastly, Tables \ref{tab:archi_inf_net} depict the architecture used to learn both the mean and covariance matrix for the approximate posterior assumed to be Gaussian. 

\begin{table}[!htbp]
\centering
\begin{tabular}{|c|}
\hline Inputs: $\{\Phi(\mathbf{h}_t)\}_{ 1 \leq t \leq T}$, $\mathbf{z}$ \\
\hline Concatenate: $[\Phi(\mathbf{h}_t), \mathbf{z}]_{ 1 \leq t \leq T}$\\
\hline Linear Layer \\ 
\hline Weight Normalization \\
\hline ELU  \\
\hline Linear Layer \\
\hline Weight Normalization \\
\hline Linear Layer  \\
\hline Output: $\{\hat{Y}_{t+1}(\omega)\}_{ 1 \leq t \leq T-1}$ \\ 
\hline
 \end{tabular}
\caption{Architecture of the outcome model prediction, i.e., the decoder.}
\label{tab:archi_f_theta}
\end{table}

\begin{table}[!htbp]
\centering
\begin{minipage}{0.33\textwidth}
\centering
\begin{tabular}{|c|}
\hline Inputs: $\{y_{t}, \mathbf{x}_{t}, \omega_{t}\}_{ 1 \leq t \leq T}$ \\
\hline Concat: $[y_{t}, \mathbf{x}_{t}, \omega_{t}]_{ 1 \leq t \leq T}$ \\
\hline GRU layer \\
\hline Linear Layer \\
\hline Tanh  \\
\hline Outputs: $\{\Phi(\textbf{h}_t)\}_{ 1 \leq t \leq T}$\\ \hline
\end{tabular}
\caption{Architecture: representation learner $\phi$ of CDVAE}
\label{tab:archi_phi_rep_learner}
\end{minipage}%
\begin{minipage}{0.33\textwidth}
\centering
\begin{tabular}{|c|}
\hline Inputs: $\{\Phi(\mathbf{h}_t)\}_{ 1 \leq t \leq T}$ \\
\hline Linear Layer \\
\hline ELU  \\
\hline Sigmoid  \\
\hline Output: $\{\hat{W}_{t+1}(\omega)\}_{ 1 \leq t \leq T-1}$ 
 \\ \hline\end{tabular}
\caption{Architecture: propensity network  $e_{\theta_{\omega}}(.)$.}
\label{tab:archi_e_theta}
\end{minipage}
\begin{minipage}{0.33\textwidth}
\centering
\begin{tabular}{|c|} \hline 

Inputs: $\{y_{t}, \mathbf{x}_{t}, \omega_{t}\}_{1 \leq t \leq T}$ \\ \hline  
Concat: $[y_{t}, \mathbf{x}_{t}, \omega_{t}]_{1 \leq t \leq T}$ \\ \hline  
GRU layer \\ \hline 

\begin{tabular}{c|c}  Linear Layer & Linear Layer  \end{tabular}\\ \hline 

\begin{tabular}{c|c}  $\Sigma_{\phi_3}\left(\mathbf{g}_T\right)$ & $\mu_{\phi_2}\left(\mathbf{g}_T\right)$ \end{tabular}\\ \hline 

\end{tabular}
\caption{Inference network $q_\phi\left(\mathbf{z} \mid y_{\leq T}, \mathbf{x}_{\leq T}, \omega_{\leq T}\right)$}
\label{tab:archi_inf_net}
\end{minipage}
\end{table}
