# Supplementary material for: Learning Causality for Longitudinal Data
Source: arXiv:2512.04980 source file (2025-12-04)
Supplement: Supplementary file 2 [file 4.tex]

\chapter{Appendix: Chapter \ref{chapter:ccpc}}
  
\section{Experiments on semi-synthetic data: Details} 

\subsection{Additional results}
\label{appendix_ccpc:detailed_results_mimic}

\subsubsection{Comparison to benchmark models: standard train/test split}
\label{appendix_ccpc:results_orig_mimic}
We also tested Causal CPC on MIMIC III semi-synthetic data using the same experimental protocol as \cite{Melnychuk2022CausalTF}, namely by using the split of patients into train/validation/test as 800/200/200. As a result, baseline performances in Table \ref{tab: perf_mimic_orig_data} are exactly the same as in \cite{Melnychuk2022CausalTF}. 
\begin{table}[!htbp]
 \caption{Results over the MIMIC III semi-synthetic data set (same experimental protocol as in \cite{Melnychuk2022CausalTF}): mean$\pm$standard deviation of Rooted Mean Squared Errors (RMSEs). The best value for each metric is given in bold: smaller is better.}
 \centering
\resizebox{\textwidth}{!}{%
\begin{tabular}{|c |c |c |c |c |c  |c |c |c |c |c|} 
\hline
Model       & $\rho = 1$   &   $\rho = 2$& $\rho = 3$&   $\rho = 4$&  $\rho = 5$&   $\rho = 6$& $\rho = 7$&  $\rho = 8$&   $\rho = 9$ & $\rho = 10$\\ \hline  

\textbf{Causal CPC (ours)}  &   0.25 $\pm$ 0.03  & \textbf{0.37 $\pm$ 0.02}  &\textbf{0.40 $\pm$ 0.01} & \textbf{0.45 $\pm$ 0.01} & \textbf{0.49 $\pm$ 0.02} & \textbf{0.52 $\pm$ 0.02} & \textbf{0.55 $\pm$ 0.03}  &\textbf{0.56 $\pm$ 0.03 } &\textbf{0.58 $\pm$ 0.04} & \textbf{0.60 $\pm$ 0.03} \\ 
\hline  
\textbf{Causal Transformer} & \textbf{ 0.20 $\pm$ 0.01 } & 0.38 $\pm$ 0.01  &0.45 $\pm$ 0.01 & 0.49 $\pm$ 0.01 & 0.52 $\pm$ 0.02 & 0.53 $\pm$ 0.02 & 0.55 $\pm$ 0.02  &\textbf{0.56 $\pm$ 0.02}  &\textbf{0.58 $\pm$ 0.02} & \textbf{0.59 $\pm$ 0.02}  \\ 
\hline  
\textbf{G-Net} & 0.34 $\pm$ 0.01& 0.67 $\pm$ 0.03& 0.83 $\pm$ 0.04& 0.94 $\pm$ 0.04& 1.03 $\pm$ 0.05 &1.10 $\pm$ 0.05 &1.16 $\pm$ 0.05 &1.21 $\pm$ 0.06& 1.25 $\pm$ 0.06 & 1.29 $\pm$ 0.06\\ 
\hline  
\textbf{CRN} &  0.30 $\pm$ 0.01& 0.48 $\pm$ 0.02 &0.59 $\pm$ 0.02& 0.65 $\pm$ 0.02 &0.68 $\pm$ 0.02& 0.71 $\pm$ 0.01 &0.72 $\pm$ 0.01 &0.74 $\pm$ 0.01 &0.76 $\pm$ 0.01& 0.78 $\pm$ 0.02\\ 
\hline  
\textbf{RMSN} &   0.24 $\pm$ 0.01& 0.47 $\pm$ 0.01& 0.60 $\pm$ 0.01& 0.70 $\pm$ 0.02& 0.78 $\pm$ 0.04 &0.84 $\pm$ 0.05 &0.89 $\pm$ 0.06& 0.94 $\pm$ 0.08 & 0.97 $\pm$ 0.09& 1.00 $\pm$ 0.11 \\ 
\hline  
\textbf{MSM} & 0.37 $\pm$ 0.01& 0.57 $\pm$ 0.03& 0.74 $\pm$ 0.06 &0.88 $\pm$ 0.03& 1.14 $\pm$ 0.10 &1.95 $\pm$ 1.48 &3.44 $\pm$ 4.57 &$>$ 10.0 & $>$ 10.0 & $>$ 10.0\\ 
\hline  
 \end{tabular}
 }
\label{tab: perf_mimic_orig_data}
\end{table}

\section{Proofs of theoretical results}
\label{appendix_ccpc:proofs}
\subsection{Relation between InfoNCE loss and mutual information}

\begin{proposition}
    $$I(\mathbf{F}_{t+j}, \mathbf{C}_{t}) \geq \log(|\mathcal{B}|) - \mathcal{L}^{(InfoNCE)}_j$$
\end{proposition}

\begin{proof}

In the following, we draw inspiration from the proof of \citet{oord2018representation}. The InfoNCE loss can be interpreted as the categorical cross-entropy of correctly classifying the positive sample \(\mathbf{F}_{t+j}\) given the context \(\mathbf{C}_t^{\mathrm{enc}}\). This is done with probability
\[
\frac{\exp\bigl(T_j(\mathbf{F}_{t+j}, \mathbf{C}_t)\bigr)}%
{\sum_{l = 1}^{|\mathcal{B}|} \exp\bigl(T_j(\mathbf{F}_{l,t+j}, \mathbf{C}_t)\bigr)},
\]
where \(\mathbf{F}_{t+j}\) is treated as the positive sample within the batch \(\mathcal{B}\), and the remaining elements serve as negative samples. Let $\texttt{pos} \in \{1, \dots, |\mathcal{B}|\}$ be the indicator of the positive sample $\mathbf{F}_{t+j}$.  The optimal probability is 
\[
\begin{aligned}
p(\mathrm{Index} = \mathtt{pos} \mid \mathcal{B}, \mathbf{C}_t^{\mathrm{enc}}) 
&= \frac{p(\mathbf{f}_{\mathtt{pos}, t+j} \mid \mathbf{C}_t^{\mathrm{enc}}) 
\prod_{\substack{l=1 \\ l \ne \mathtt{pos}}}^{\mathcal{B}} p(\mathbf{f}_{l, t+j})}
{\sum_{j=1}^{\mathcal{B}} \left[ p(\mathbf{f}_{j, t+j} \mid \mathbf{C}_t^{\mathrm{enc}}) 
\prod_{\substack{l=1 \\ l \ne j}}^{\mathcal{B}} p(\mathbf{f}_{l, t+j}) \right]} \\[1.5ex]
&= \frac{ \dfrac{p(\mathbf{f}_{\mathtt{pos}, t+j} \mid \mathbf{C}_t^{\mathrm{enc}})}{p(\mathbf{f}_{\mathtt{pos}, t+j})} }
{\sum_{j=1}^{\mathcal{B}} \dfrac{p(\mathbf{f}_{j, t+j} \mid \mathbf{C}_t^{\mathrm{enc}})}{p(\mathbf{f}_{j, t+j})}}.
\end{aligned}
\]

Now, for  the score $\exp(T_j(\mathbf{F}_{t+j},\mathbf{C}_{t}))$  to be optimal, it should be proportional to $ \frac{p(\mathbf{f}_{\texttt{pos}, t+j} \vert c)}{p(\mathbf{f}_{\texttt{pos}, t+j})}$.  The MI lower bound comes from the fact that $ \exp(T_j(\mathbf{F}_{t+j},\mathbf{C}_{t})) $ estimates the density ratio $ \frac{p(\mathbf{f}_{\texttt{pos}, t+j} \vert c)}{p(\mathbf{f}_{\texttt{pos}, t+j})}$.

\begin{equation}
\begin{aligned}
\mathcal{L}^{(InfoNCE)}_j & =-\mathbb{E}_{\mathcal{B}} \log \left[\frac{\frac{p\left(\mathbf{f}_{t+j} \mid \mathbf{C}_t^{\mathrm{enc}}\right)}{p\left(\mathbf{f}_{t+j}\right)}}{\frac{p\left(\mathbf{f}_{t+j} \mid \mathbf{C}_t^{\mathrm{enc}}\right)}{p\left(\mathbf{f}_{t+j}\right)}+\sum_{\mathbf{f}_{l, t+j} \in \mathcal{B}_{\text {neg }}} \frac{p\left(\mathbf{f}_{l, t+j} \mid \mathbf{C}_t^{\mathrm{enc}}\right)}{p\left(\mathbf{f}_{l, t+j}\right)}}\right] \\
& =\mathbb{E}_{\mathcal{B}} \log \left[1+\frac{p\left(\mathbf{f}_{t+j}\right)}{p\left(\mathbf{f}_{t+j} \mid \mathbf{C}_t^{\mathrm{enc}}\right)} \sum_{\mathbf{f}_{l, t+j} \in \mathcal{B}_{\text {neg }}} \frac{p\left(\mathbf{f}_{l, t+j} \mid \mathbf{C}_t^{\mathrm{enc}}\right)}{p\left(\mathbf{f}_{l, t+j}\right)}\right] \\
& \approx \mathbb{E}_{\mathcal{B} }\log \left[1+\frac{p\left(\mathbf{f}_{t+j}\right)}{p\left(\mathbf{f}_{l, t+j} \mid \mathbf{C}_t^{\mathrm{enc}}\right)}(|\mathcal{B}|-1) \mathbb{E}_{\mathbf{F}_{t+j}} \frac{p\left(\mathbf{f}_{l, t+j}\mid \mathbf{C}_t^{\mathrm{enc}}\right)}{p\left(\mathbf{f}_{l, t+j}\right)}\right] \\
& =\mathbb{E}_{\mathcal{B}} \log \left[1+\frac{p\left(\mathbf{f}_{t+j}\right)}{p\left(\mathbf{f}_{t+j} \mid \mathbf{C}_t^{\mathrm{enc}}\right)}(|\mathcal{B}|-1)\right] \\
& \geq \mathbb{E}_{\mathcal{B}} \log \left[\frac{p\left(\mathbf{f}_{t+j}\right)}{p\left(\mathbf{f}_{t+j}\mid \mathbf{C}_t^{\mathrm{enc}}\right)} |\mathcal{B}|\right] \\
& =-I\left(\mathbf{f}_{t+j}, \mathbf{C}_t^{\mathrm{enc}}\right)+\log (|\mathcal{B}|),
\end{aligned}
\label{eq:infonce_proof}
\end{equation}

The approximation in the third equation, Eq. \eqref{eq:infonce_proof}, becomes more precise as the batch size increases.
\end{proof}

\subsection{Relation between InfoMax and input reconstruction}
 We now prove the proposition \ref{prop:lb_infomax} stating that : $ I(\mathbf{C}_t^{\mathrm{enc},h},\mathbf{C}_t^{\mathrm{enc},f})\leq I(\mathbf{H}_{t}, (\mathbf{C}_t^{\mathrm{enc},h}, \mathbf{C}_t^{\mathrm{enc},f}))$
 \begin{proof}
    This is followed by two applications of the data processing inequality \cite{cover1999elementsInfo}, which states that for random variables \(A\), \(B\), and \(C\) satisfying the Markov relation \(A \to B \to C\), we have
\[
I(A;C) \leq I(A;B).
\]

First, note that
\[
\mathbf{C}_t^{\mathrm{enc},h} = \Phi_{\theta_{1},\theta_{2}}(\mathbf{H}_t^h), \quad
\mathbf{C}_t^{\mathrm{enc},f} = \Phi_{\theta_{1},\theta_{2}}(\mathbf{H}_t^f),
\]
where \(\mathbf{H}_t^h = \mathrm{trunc}_f(\mathbf{H}_t)\) and \(\mathbf{H}_t^f = \mathrm{trunc}_h(\mathbf{H}_t)\). Here, \(\mathrm{trunc}_f\) and \(\mathrm{trunc}_h\) truncate the future and history processes, respectively, relative to a splitting time \(t_0\).

We now observe the Markov relation
\[
\mathbf{C}_t^{\mathrm{enc},h} 
\xleftarrow{\Phi_{\theta_{1},\theta_{2}} \circ \mathrm{trunc}_f} 
\mathbf{H}_t 
\xrightarrow{\Phi_{\theta_{1},\theta_{2}} \circ \mathrm{trunc}_h}
\mathbf{C}_t^{\mathrm{enc},f},
\]
which is Markov equivalent to
\[
\mathbf{C}_t^{\mathrm{enc},h}
\xrightarrow{\Phi_{\theta_{1},\theta_{2}} \circ \mathrm{trunc}_f}
\mathbf{H}_t
\xrightarrow{\Phi_{\theta_{1},\theta_{2}} \circ \mathrm{trunc}_h}
\mathbf{C}_t^{\mathrm{enc},f}.
\]
By the data processing inequality, this gives
\[
I(\mathbf{C}_t^{\mathrm{enc},h}; \mathbf{C}_t^{\mathrm{enc},f})
\leq I(\mathbf{H}_t; \mathbf{C}_t^{\mathrm{enc},h}).
\]

On the other hand, we trivially have the Markov relation
\[
\mathbf{H}_t \to (\mathbf{C}_t^{\mathrm{enc},h}, \mathbf{C}_t^{\mathrm{enc},f}) \to \mathbf{C}_t^{\mathrm{enc},h},
\]
which yields
\[
I(\mathbf{H}_t; \mathbf{C}_t^{\mathrm{enc},h})
\leq I(\mathbf{H}_t; (\mathbf{C}_t^{\mathrm{enc},h}, \mathbf{C}_t^{\mathrm{enc},f})).
\]

Combining the two inequalities proves the proposition.
\end{proof}
\subsection{Proof of Theorem \ref{thm:tightness_lb_info}}

To begin, we split the process history into two non-overlapping views (Figure \ref{fig:ccpc_archi}): $\mathbf{H}_t^h \coloneqq \mathbf{F}_{1:t_0}$ and $\mathbf{H}_t^f \coloneqq \mathbf{F}_{t_0+1:t}$, representing a historical subsequence and a future subsequence within the process history $\mathbf{H}_{t}$, respectively. We then computed representations of these two views denoted $\mathbf{C}_t^{\mathrm{enc},h}$ and $\mathbf{C}_t^{\mathrm{enc},f}$, respectively. This naturally gives rise to the Markov chain, as in showed in the proof of proposition \ref{prop:lb_infomax}:
\[
\mathbf{C}_t^{\mathrm{enc},h} \xleftarrow[]{} \mathbf{H}_t \xrightarrow[]{} \mathbf{C}_t^{\mathrm{enc},f}
\]
which is Markov equivalent to:
\[
\mathbf{C}_t^{\mathrm{enc},h} \xrightarrow{} \mathbf{H}_t \xrightarrow[]{} \mathbf{C}_t^{\mathrm{enc},f}
\]
Following this Markov chain, we can show that \cite{shwartz2024compress}:
\[
I(\mathbf{C}_t^{\mathrm{enc},f}, \mathbf{C}_t^{\mathrm{enc},h}) = I(\mathbf{H}_t, \mathbf{C}_t^{\mathrm{enc},h}) - \mathbb{E}_{\mathbf{h}_t \sim \mathbb{P}_{\mathbf{H}_t}} \mathbb{E}_{\mathbf{c}_{t}^f \sim \mathbb{P}_{\mathbf{C}_{t}^f \mid \mathbf{h}_t}} \left[ D_{KL}[\mathbb{P}_{\mathbf{C}_{t}^h \mid \mathbf{h}_t} || \mathbb{P}_{\mathbf{C}_{t}^h \mid \mathbf{c}_{t}^f }] \right]
\]
On the other hand, by applying the chain rule of the mutual information to $I(\mathbf{H}_{t}; (\mathbf{C}_t^{\mathrm{enc},h}, \mathbf{C}_t^{\mathrm{enc},f}))$ we get:
\[
I(\mathbf{H}_{t}; (\mathbf{C}_t^{\mathrm{enc},f}, \mathbf{C}_t^{\mathrm{enc},h})) = I(\mathbf{H}_t, \mathbf{C}_t^{\mathrm{enc},h}) + I(\mathbf{H}_t; \mathbf{C}_t^{\mathrm{enc},f} \mid \mathbf{C}_t^{\mathrm{enc},h}) 
\]
Combining these equations, the tightness of our bounds can be written as:
\begin{equation}
\begin{aligned}
I(\mathbf{H}_{t}; (\mathbf{C}_t^{\mathrm{enc},f}, \mathbf{C}_t^{\mathrm{enc},h})) 
&- I(\mathbf{C}_t^{\mathrm{enc},f}, \mathbf{C}_t^{\mathrm{enc},h}) \\
&= I(\mathbf{H}_t; \mathbf{C}_t^{\mathrm{enc},f} \mid \mathbf{C}_t^{\mathrm{enc},h}) \\
&\quad + \mathbb{E}_{\mathbf{h}_t \sim \mathbb{P}_{\mathbf{H}_t}} 
\mathbb{E}_{\mathbf{c}_{t}^f \sim \mathbb{P}_{\mathbf{C}_{t}^f \mid \mathbf{h}_t}} 
\bigg[
    D_{\mathrm{KL}}\bigl(
        \mathbb{P}_{\mathbf{C}_{t}^h \mid \mathbf{h}_t}
        \,\big\|\, 
        \mathbb{P}_{\mathbf{C}_{t}^h \mid \mathbf{c}_{t}^f}
    \bigr)
\bigg].
\end{aligned}
\end{equation}

\subsection{On the relation between conditional entropy and reconstruction}
\label{appendix: zero_cond_H}
We now prove the statement in the core paper, saying that the conditional entropy $H(\mathbf{H}_{t}\mid (\mathbf{C}_t^{\mathrm{enc},h}, \mathbf{C}_t^{\mathrm{enc},f})) \geq 0$ is minimized if $\mathbf{H}_{t}$ is a function of $(\mathbf{C}_t^{\mathrm{enc},h}, \mathbf{C}_t^{\mathrm{enc},f})$ almost surely.
\begin{proposition}
\label{prop:zero_cond_H}
$H(\mathbf{A} \mid \mathbf{B}) =  0$ implies that $\mathbf{A} = f(\mathbf{B})$ almost surely.
\end{proposition}
\begin{proof}
   For simplicity, suppose \(\mathbf{A}\) and \(\mathbf{B}\) are discrete. Assume, by contradiction, that there exists \(\mathbf{b}_0\) and two distinct values \(\mathbf{a}_1\) and \(\mathbf{a}_2\) such that \(p(\mathbf{a}_1 \mid \mathbf{b}_0), p(\mathbf{a}_2 \mid \mathbf{b}_0) > 0\). Then the conditional entropy is given by:
\[
H(\mathbf{A} \mid \mathbf{B}) 
= -\sum_{\mathbf{b}} p(\mathbf{b}) \sum_{\mathbf{a}} p(\mathbf{a} \mid \mathbf{b}) \log p(\mathbf{a} \mid \mathbf{b}).
\]
In particular, we have:
\[
H(\mathbf{A} \mid \mathbf{B}) 
\geq p(\mathbf{b}_0) \bigg(-p(\mathbf{a}_1 \mid \mathbf{b}_0) \log p(\mathbf{a}_1 \mid \mathbf{b}_0) 
- p(\mathbf{a}_2 \mid \mathbf{b}_0) \log p(\mathbf{a}_2 \mid \mathbf{b}_0)\bigg) > 0,
\]
where we used the fact that \(-t \log t \geq 0\) for \(0 \leq t \leq 1\), with strict inequality for \(t \notin \{0,1\}\).  

Therefore, \(H(\mathbf{A} \mid \mathbf{B}) = 0\) if and only if \(\mathbf{A}\) is a function of \(\mathbf{B}\) almost surely.
% Reformulate !!!!!!!!!!!!!!!!!!!
\end{proof}

\subsection{Proof of theorem \ref{thm:blancing_iclub}} 

To prove the Theorem \ref{thm:blancing_iclub}, we first prove the following lemma and proposition.
\begin{lemma}
    Let $\Phi$ be a fixed representation function. Given that $q(W_{t+1} \mid \Phi(\mathbf{H}_t)) $ is the conditional likelihood of observing the treatment $W_{t+1}$, denote the probability of observing each treatment value as $q^j=q(\Phi(\mathbf{H}_t))\coloneqq q(W_{t+1} = j \mid \Phi(\mathbf{H}_t))$ for $j \in \{0,1,\dots, K-1\}$. Then, the optimal treatment prediction function is such that 
    \begin{equation}
        q^{j, *}(\Phi(\mathbf{H}_t) ) = \frac{p(\Phi(\mathbf{H}_t)\mid W_{t+1} = j)}{\sum_{l=0}^{K-1}p(\Phi(\mathbf{H}_t)\mid W_{t+1} = l)p(W_{t+1} = l)}
    \end{equation}
    \label{lem: optimal_q}
\end{lemma}
\begin{proof}
    For a fixed representation \(\Phi\), finding the optimal treatment probabilities reduces to solving the following constrained optimization problem:
\begin{equation}
    \begin{aligned}
        \max_{q} \;\; & \mathbb{E}_{\mathbb{P}(\Phi(\mathbf{H}_t), W_{t+1})} 
        \left[ \log q(W_{t+1} \mid \Phi(\mathbf{H}_t)) \right] \\
        \textrm{subject to} \;\; & \sum_{l=0}^{K-1} q^l(\Phi(\mathbf{H}_t)) = 1.
    \end{aligned}
    \label{eq:max_treat_constrained}
\end{equation}
First, we write the likelihood $q(W_{t+1} \mid \Phi(\mathbf{H}_t))$ using the conditional probabilities $q^j(\Phi(\mathbf{H}_t))$.
\begin{equation*}
    q(W_{t+1} \mid \Phi(\mathbf{H}_t)) = \prod_{j=0}^{K-1}q^j(\Phi(\mathbf{H}_t))^{\indicator{W_{t+1}=j}}
\end{equation*}
Then, the treatment likelihood can be written as   
\begin{align*}
    \mathbb{E}_{\mathbb{P}(\Phi(\mathbf{H}_t), W_{t+1})} \left[ \log q(W_{t+1} \mid \Phi(\mathbf{H}_t)) \right] 
    &=  \mathbb{E}_{\mathbb{P}(\Phi(\mathbf{H}_t), W_{t+1})} \left[ \sum_{l=0}^{K-1} \log(q^{l}(\Phi(\mathbf{H}_t))) \mathbb{1}_{\{W_{t+1}=l\}} \right] \\
    &=  \sum_{l=0}^{K-1} \int \log(q^{l}(\Phi(\mathbf{H}_t))) \mathbb{1}_{\{W_{t+1}=l\}}\, p(W_{t+1} \mid \Phi(\mathbf{H}_t))\, p(\Phi(\mathbf{H}_t))\, dW_{t+1}\, d\Phi(\mathbf{H}_t) \\
    &= \sum_{l=0}^{K-1} \int \log(q^{l}(\Phi(\mathbf{H}_t)))\, p(W_{t+1} = l \mid \Phi(\mathbf{H}_t))\, p(\Phi(\mathbf{H}_t))\, d\Phi(\mathbf{H}_t) \\
    &= \sum_{l=0}^{K-1} \int \log(q^{l}(\Phi(\mathbf{H}_t)))\, p(\Phi(\mathbf{H}_t) \mid W_{t+1} = l)\, p(W_{t+1} = l)\, d\Phi(\mathbf{H}_t)
\end{align*}
Let's denote $\alpha_l = p(W_{t+1} = l)$,  the marginal probability of observing the $l$-th treatment regime, and $p_{l}^{\Phi}(\mathbf{H}_t) = p(\Phi(\mathbf{H}_t)\mid W_{t+1} = l )$ with a corresponding probability distribution $\mathbb{P}_{l}^{\Phi}$.  We intend to maximize point-wise the objective in Eq. \eqref{eq:max_treat_constrained}. Plugging the latter formulation of the conditional likelihood in Eq. \eqref{eq:max_treat_constrained}  and writing the Lagrangian function, we get
\begin{equation}
    \max_{q} \sum_{l=0}^{K-1} \log(q^{l}(\Phi(\mathbf{H}_t))p_{j}^{\Phi}(\mathbf{H}_t) \alpha_l + \lambda (\sum_{l=0}^{K-1}q^{l}(\Phi(\mathbf{H}_t)) - 1)  
\end{equation}
Computing the gradient w.r.t $q^{l}(\Phi(\mathbf{H}_t))$ for  $l \in \{0,1,\dots, K-1\}$ and setting to zero, we have
\begin{equation}
    q^{l, *}(\Phi(\mathbf{H}_t)) = -\frac{\alpha_l p_{j}^{\Phi}(\mathbf{H}_t)}{\lambda}
\end{equation}
Then, by the equality constraint, we find that $\lambda = -\sum_{l=0}^{K-1}\alpha_l p_{j}^{\Phi}(\mathbf{H}_t)$.
\end{proof}
\begin{proposition}
\label{prop:iclub_form}
    Let $\Phi$ be a fixed representation function.  The $I_{CLUB}$ objective when the treatment prediction function is optimal (i.e. $ q=q^{*})$ has the following form: 
     \begin{equation}
I_{CLUB} = \sum_{j=0}^{K-1}\alpha_l D_{KL}(\mathbb{P}_j^{\Phi}|| \sum_{l=0}^{K-1}\alpha_l \mathbb{P}_l^{\Phi}) 
+ \mathbb{E}_{\mathbb{P}_{\Phi(\mathbf{H}_t)}}\left[ D_{KL}(\mathbb{P}_{W_{t+1}}||\mathbb{P}_{W_{t+1}|\Phi(\mathbf{H}_t)} )  \right]
         \label{eq:i_club_optimal_q}
     \end{equation}
\end{proposition}
\begin{proof}
 First, recall that
\begin{equation*}
    \begin{aligned}
        I_{\mathrm{CLUB}}(\Phi(\mathbf{H}_t), W_{t+1}; q^*) 
        &= \mathbb{E}_{\mathbb{P}_{(\Phi(\mathbf{H}_{t+1}), W_{t+1})}}
        \left[ \log q^*(W_{t+1} \mid \Phi(\mathbf{H}_{t+1})) \right] \\
        &\quad - \mathbb{E}_{\mathbb{P}_{\Phi(\mathbf{H}_{t+1})}}
        \mathbb{E}_{\mathbb{P}_{W_{t+1}}}
        \left[ \log q^*(W_{t+1} \mid \Phi(\mathbf{H}_{t+1})) \right].
    \end{aligned}
\end{equation*}
\begin{equation*}
        I_{\text{CLUB}}(\Phi(\mathbf{H}_t), W_{t+1}; q^{*}) =  A - B
    \end{equation*}
    Let's detail $A$ and $B$ separately, 
    \begin{equation*}
        \begin{aligned}
        A &= \sum_{j=0}^{K-1} \int \alpha_j \log(q^{l, *}(\Phi(\mathbf{H}_t)) p_{j}^{\Phi}(\mathbf{H}_t) d\Phi(\mathbf{H}_t) \\ 
        &= \sum_{j=0}^{K-1} \int\alpha_j \log(\frac{\alpha_j p_{j}^{\Phi}(\mathbf{H}_t)}{\sum_{l=0}^{K-1}p_{l}^{\Phi}(\mathbf{H}_t)\alpha_l}) p_{j}^{\Phi}(\mathbf{H}_t) d\Phi(\mathbf{H}_t) \\ 
        &= \sum_{j=0}^{K-1} \int \alpha_j \log(\frac{p_{j}^{\Phi}(\mathbf{H}_t)}{\sum_{l=0}^{K-1}p_{l}^{\Phi}(\mathbf{H}_t)\alpha_l}) p_{j}^{\Phi}(\mathbf{H}_t) d\Phi(\mathbf{H}_t) +\log(\alpha_j)\alpha_j \\
         &= \sum_{j=0}^{K-1} \alpha_j D_{KL}(\mathbb{P}_j^{\Phi}|| \sum_{l=0}^{K-1}\alpha_l \mathbb{P}_l^{\Phi}) +  \sum_{j=0}^{K-1} \log(\alpha_j)\alpha_j \\ 
        \end{aligned}
    \end{equation*}

    Finally, we can write 
    \begin{equation}
    A = \sum_{j=0}^{K-1} \alpha_j D_{KL}(\mathbb{P}_j^{\Phi}|| \sum_{l=0}^{K-1}\alpha_l \mathbb{P}_l^{\Phi})  - H(W_{t+1}) 
        \label{eq:A_final_form}
    \end{equation}
    For the remaining term $B$, we have
     \begin{equation*}
        \begin{aligned}
        B &= \mathbb{E}_{\mathbb{P}_{\Phi(\mathbf{H}_t)}}\mathbb{E}_{\mathbb{P}_{W_{t+1}}}\left( \log q^{*}(W_{t+1} \mid \Phi(\mathbf{H}_{t+1})) \right] \\ 
        &= \sum_{j=0}^{K-1} \mathbb{E}_{\mathbb{P}_{\Phi(\mathbf{H}_t)}} \mathbb{E}_{\mathbb{P}_{W_{t+1}}} \left[ \log(q^{j}(\Phi(\mathbf{H}_t))) \mathbb{1}_{\{W_{t+1}=j\}} \right] \\ 
        &= \sum_{j=0}^{K-1} \mathbb{E}_{\mathbb{P}_{\Phi(\mathbf{H}_t)}}\left[ \alpha_j \log(q^{j}(\Phi(\mathbf{H}_t)))\right] \\ 
        &= \sum_{j=0}^{K-1}\alpha_j \int \log\left[ \frac{\alpha_j p_{j}^{\Phi}(\mathbf{H}_t)}{\sum_{l=0}^{K-1}p_{l}^{\Phi}(\mathbf{H}_t)\alpha_l}\right]p(\Phi(\mathbf{H}_t))d\Phi(\mathbf{H}_t) \\ 
       &= \sum_{j=0}^{K-1}\alpha_j \int \log\left[ \frac{p(\Phi(\mathbf{H}_t))}{\sum_{l=0}^{K-1}p_{l}^{\Phi}(\mathbf{H}_t)\alpha_l} \frac{p(W_{t+1} =j \mid \Phi(\mathbf{H}_t))}{p(W_{t+1} =j)}\right]p(\Phi(\mathbf{H}_t))d\Phi(\mathbf{H}_t)\\ 
       &- H(W_{t+1})  \\ 
       &= \sum_{j=0}^{K-1}\alpha_j \int \underbrace{\log\left[ \frac{p(\Phi(\mathbf{H}_t))}{\sum_{l=0}^{K-1}p_{l}^{\Phi}(\mathbf{H}_t)\alpha_l}\right]}_{=0}p(\Phi(\mathbf{H}_t))d\Phi(\mathbf{H}_t) \\ 
        &+ \sum_{j=0}^{K-1}\alpha_j \int \log\left[\frac{p(W_{t+1} =j \mid \Phi(\mathbf{H}_t))}{p(W_{t+1} =j)}\right] p(\Phi(\mathbf{H}_t))d\Phi(\mathbf{H}_t) - H(W_{t+1}) \\
        \end{aligned}
    \end{equation*}
    The final form of $B$ is therefore 
    \begin{equation}
    B = - \int D_{KL}(\mathbb{P}_{W_{t+1}}| \mathbb{P}_{W_{t+1}| \Phi(\mathbf{H}_t)})p(\Phi(\mathbf{H}_t)) d\Phi(\mathbf{H}_t)
       - H(W_{t+1}) 
        \label{eq:B_final_form}
    \end{equation}
    The proposition follows immediately from Equations \eqref{eq:A_final_form} and \eqref{eq:B_final_form}.
\end{proof}

\begin{proof}(Theorem \ref{thm:blancing_iclub})
Since by lemma \ref{lem: optimal_q}, the $I_{CLUB}$ formulation in  proposition \ref{prop:iclub_form} holds, then to prove that the representation is balanced, it is enough to see that by the positivity of $D_{KL}$

\begin{equation}
\label{eq:iclub_ineq_at_optimal}
    I_{CLUB} \geq  \mathbb{E}_{\mathbb{P}_{\Phi(\mathbf{H}_t)}}\left[ D_{KL}(\mathbb{P}_{W_{t+1}}||\mathbb{P}_{W_{t+1}|\Phi(\mathbf{H}_t)} )\right] \geq 0  
\end{equation}
$I_{CLUB}$ is minimal when $I_{CLUB} =0$, which happens if and only if for $j \in \{0,1,\dots, K-1\}$  $p(W_{t+1} =j ) = p(W_{t+1} =j \mid \Phi(\mathbf{H}_t))$ almost surely which, by Bayes rule is equivalent to say $p(\Phi(\mathbf{H}_t)) = p(\Phi(\mathbf{H}_t) \mid W_{t+1} =j) $.
% To prove inequality  in \eqref{eq:iclub_ineq_at_optimal}, we use that fact the Keullbeick Leibler divergence $(p, q) \rightarrow D(p||q)$ is convex over the pair of the probability distributions so that we have the property 

% \begin{equation*}
%     D(\sum_{j=0}^{K-1}\lambda_j p_j||\sum_{j=0}^{K-1}\lambda_jq_j) \leq \sum_{j=0}^{K-1}\lambda_j D(p_j||q_j)
% \end{equation*}
%     such that $ 0 \leq \lambda_j \leq 1 $ and $\sum_{j=0}^{K-1}\lambda_j=1$. 

%     Going back to our $I_{CLUB}$ formulation in Eq. \eqref{eq:i_club_optimal_q} we have 
%     \begin{equation}
%     \begin{aligned}
%         D_{KL}(p^{\Phi}||  \sum_{l=0}^{K-1}\alpha_l p_l^{\Phi}) &= D_{KL}(p^{\Phi}||  \sum_{l=0}^{K-1}\alpha_l p_l^{\Phi}) \\ 
%         & = D_{KL}(p^{\Phi}||  \sum_{l=0}^{K-1}\alpha_l p_l^{\Phi}) &= D_{KL}(p^{\Phi}||  \sum_{l=0}^{K-1}\alpha_l p_l^{\Phi})
%         \end{aligned}
        
%     \end{equation}
    
\end{proof}

\section{Causal CPC: Architecture details}
\label{appendix_ccpc:archi_ccpc}
\begin{table}[!htbp]
\centering
\begin{tabular}{c}
\hline \textbf{Inputs}: $[\mathbf{X}_{t}, W_{t-1}, Y_{t-1}]$\\
\hline Linear Layer\\
\hline WeightNorm\\
\hline SELU\\
\hline Linear Layer  \\
\hline WeightNorm\\
\hline \textbf{Outputs}: $\mathbf{Z}_t = \Phi_{\theta_1}([\mathbf{X}_{t}, W_{t-1}, Y_{t-1}])$\\
\end{tabular}
\caption{Architecture for learning local features $\mathbf{Z}_t$}
\label{tab: archi_loc_feat}
\end{table}

\begin{table}[!htbp]
\centering
\begin{tabular}{c}
\hline \textbf{Inputs}: $\mathbf{Z}_{\leq t}$\\
\hline GRU (1 layer)\\
\hline \textbf{Outputs}: Hidden state $\mathbf{C}_t^{\mathrm{enc}} = \Phi_{\theta_2}^{ar}(\mathbf{Z}_{\leq t})$\\
\end{tabular}
\caption{Architecture for learning context representation $\mathbf{C}_t^{\mathrm{enc}}$ }
\label{tab: archi_context }
\end{table}

\begin{table}[!htbp]
\centering
\begin{tabular}{c}
\hline \textbf{Inputs}: $[\mathbf{\Phi}_t, W_t]$\\
\hline Linear Layer\\
\hline WeightNorm\\
\hline SELU\\
\hline Linear Layer  \\
\hline WeightNorm\\
\hline \textbf{Outputs}: $\hat{Y}_t$\\
\end{tabular}
\caption{Architecture for outcome prediction}
\label{tab: archi_outc_pred}
\end{table}

\begin{table}[!htbp]
\centering
\begin{tabular}{c}
\hline \textbf{Inputs}: $\mathbf{\Phi}_t$\\
\hline Linear Layer\\
\hline SpectralNorm\\
\hline SELU\\
\hline Linear Layer  \\
\hline SpectralNorm\\
\hline \textbf{Outputs}: $\hat{W}_t$\\
\end{tabular}
\caption{Architecture for treatment prediction}
\label{tab: archi_treat_pred}
\end{table}

\newpage
\section{Models hyperparameters}
\label{appendix_ccpc:huperparams_details}

In this section, we report the range of all hyperparameters to be fine-tuned, as well as fixed hyperparameters for all models and across the different datasets used in experiments. Best hyperparameter values are reported in the configuration files in the code repository.

\begin{table}[!htbp]
\centering
\caption{Hyper-parameters search range for RMSN}
\resizebox{0.9\textwidth}{!}{%
\begin{tabular}{|c|c|c|c|c|}
\hline
\textbf{Model} & \textbf{Sub-model} & \textbf{Hyperparameter} & \textbf{Cancer simulation} & \textbf{MIMIC III (SS)} \\
\hline
\multirow{7}{*}{RMSNs} 
& \multirow{7}{*}{Propensity Treatment Network} 
& LSTM layers & 1 & 1 \\
\cline{3-5}
& & Learning rate & $0.01, 0.005, 0.001, 0.0001$ & $0.01, 0.005, 0.001, 0.0001$ \\
\cline{3-5}
& & Batch size & $32, 64, 128$ & $32, 64, 128$ \\
\cline{3-5}
& & LSTM hidden units & $4, 6, \dots, 12$ & $4, 6, \dots, 30$ \\
\cline{3-5}
& & LSTM dropout rate & - & - \\
\cline{3-5}
& & Max gradient norm & $0.5, 1, 2$ & $0.5, 1, 2$ \\
\cline{3-5}
& & Early Stopping (min delta) & 0.0001 & 0.0001 \\
\cline{3-5}
& & Early Stopping (patience) & 30 & 30 \\
\hline
\multirow{6}{*}{Propensity History Network} 
& & LSTM layers & 1 & 1 \\
\cline{3-5}
& & Learning rate & $0.01, 0.005, 0.001, 0.0001$ & $0.01, 0.005, 0.001, 0.0001$ \\
\cline{3-5}
& & Batch size & $32, 64, 128$ & $64, 128, 256$ \\
\cline{3-5}
& & LSTM hidden units & $4, 6, \dots, 20$ & $4, 6, \dots, 30$ \\
\cline{3-5}
& & LSTM dropout rate & - & - \\
\cline{3-5}
& & Early Stopping (min delta) & 0.0001 & 0.0001 \\
\cline{3-5}
& & Early Stopping (patience) & 30 & 30 \\
\hline
\multirow{6}{*}{Encoder} 
& & LSTM layers & 1 & 1 \\
\cline{3-5}
& & Learning rate & $0.01, 0.005, 0.001, 0.0001$ & $0.01, 0.005, 0.001, 0.0001$ \\
\cline{3-5}
& & Batch size & $32, 64, 128$ & $32, 64, 128$ \\
\cline{3-5}
& & LSTM hidden units & $4, 6, \dots, 20$ & $4, 6, \dots, 30$ \\
\cline{3-5}
& & LSTM dropout rate & - & - \\
\cline{3-5}
& & Early Stopping (min delta) & 0.0001 & 0.0001 \\
\cline{3-5}
& & Early Stopping (patience) & 30 & 30 \\
\hline
\multirow{6}{*}{Decoder} 
& & LSTM layers & 1 & 1 \\
\cline{3-5}
& & Learning rate & $0.01, 0.005, 0.001, 0.0001$ & $0.01, 0.005, 0.001, 0.0001$ \\
\cline{3-5}
& & Batch size & $32, 64, 128$ & $128, 512, 1024$ \\
\cline{3-5}
& & LSTM hidden units & $4, 6, \dots, 20$ & $4, 6, \dots, 30$ \\
\cline{3-5}
& & LSTM dropout rate & - & - \\
\cline{3-5}
& & Max gradient norm & $0.5, 1, 2$ & $0.5, 1, 2$ \\
\cline{3-5}
& & Early Stopping (min delta) & 0.0001 & 0.0001 \\
\cline{3-5}
& & Early Stopping (patience) & 30 & 30 \\
\hline
\end{tabular}%
}
\end{table}

% \begin{table}[!htbp]
% \centering
% \caption{Hyper-parameters search range for CRN}
% \resizebox{0.7\textwidth}{!}{%
% \begin{tabular}{|c|c|c|c|c|}
% \hline
% \textbf{Model} & \textbf{Sub-model} & \textbf{Hyperparameter} & \textbf{Cancer simulation} & \textbf{MIMIC III (SS)} \\
% \hline
% \multirow{CRN} 
% & \multirow{Encoder} 
% & LSTM layers & 1 & 1 \\
% %\cline{3-6}
% & & Learning rate & $0.01,0.005, 0.001, 0.0001$ &$0.01,0.005, 0.001, 0.0001$ \\
% %\cline{3-6}
% & & Batch size & $32, 64, 128$ & $32, 64, 128$ \\
% %\cline{3-6}
% & & LSTM hidden units & $4,6, \dots, 30$&  $4,6, \dots, 30$ \\
% %\cline{3-6}
% & & LSTM dropout rate & - & - \\
% %\cline{3-6}
% & & BR size & $4,6, \dots, 20$  & $4,6, \dots, 30$\\
% & & Early Stopping (min delta)& 0.0001  & 0.0001\\
% & & Early Stopping (patience)& 30 &  30\\
% \hline
% & \textbf{Decoder} & LSTM layers & 1 & 1\\
% %\cline{3-6}
% & & Learning rate & $0.01,0.005, 0.001, 0.0001$ & $0.01,0.005, 0.001, 0.0001$\\
% %\cline{3-6}
% & & Batch size & $128,256,512$& $256,512,1024$ \\
%  %%\cline{3-6}
% & & LSTM hidden units & $4,6, \dots, 30$& $4,6, \dots, 30$  \\
%  %%\cline{3-6}
% & & LSTM dropout rate& - & -  \\
%  %%\cline{3-6}
%  & & BR size & $4,6, \dots, 20$& $4,6, \dots, 30$ \\
%   & & Early Stopping (min delta)& 0.0001&  0.0001\\
%  & & Early Stopping (patience)& 30& 30\\
% \hline
% \end{tabular}%
% }
% \end{table}

\begin{table}[!htbp]
\centering
\caption{Hyper-parameters search range for CRN}
\resizebox{0.7\textwidth}{!}{%
\begin{tabular}{|c|c|c|c|c|}
\hline
\textbf{Model} & \textbf{Sub-model} & \textbf{Hyperparameter} & \textbf{Cancer simulation} & \textbf{MIMIC III (SS)} \\
\hline
\multirow{8}{*}{CRN} 
& \multirow{8}{*}{Encoder} 
& LSTM layers & 1 & 1 \\
\cline{3-5}
& & Learning rate & $0.01, 0.005, 0.001, 0.0001$ & $0.01, 0.005, 0.001, 0.0001$ \\
\cline{3-5}
& & Batch size & $32, 64, 128$ & $32, 64, 128$ \\
\cline{3-5}
& & LSTM hidden units & $4, 6, \dots, 30$ & $4, 6, \dots, 30$ \\
\cline{3-5}
& & LSTM dropout rate & - & - \\
\cline{3-5}
& & BR size & $4, 6, \dots, 20$ & $4, 6, \dots, 30$ \\
\cline{3-5}
& & Early Stopping (min delta) & 0.0001 & 0.0001 \\
\cline{3-5}
& & Early Stopping (patience) & 30 & 30 \\
\hline
\multirow{7}{*}{Decoder} 
& & LSTM layers & 1 & 1 \\
\cline{3-5}
& & Learning rate & $0.01, 0.005, 0.001, 0.0001$ & $0.01, 0.005, 0.001, 0.0001$ \\
\cline{3-5}
& & Batch size & $128, 256, 512$ & $256, 512, 1024$ \\
\cline{3-5}
& & LSTM hidden units & $4, 6, \dots, 30$ & $4, 6, \dots, 30$ \\
\cline{3-5}
& & LSTM dropout rate & - & - \\
\cline{3-5}
& & BR size & $4, 6, \dots, 20$ & $4, 6, \dots, 30$ \\
\cline{3-5}
& & Early Stopping (min delta) & 0.0001 & 0.0001 \\
\cline{3-5}
& & Early Stopping (patience) & 30 & 30 \\
\hline
\end{tabular}%
}
\end{table}

\begin{table}[!htbp]
\centering
\caption{Hyper-parameters search range for G-Net}
\resizebox{0.7\textwidth}{!}{%
\begin{tabular}{|c|c|c|}
\hline
\textbf{Hyperparameter} & \textbf{Cancer simulation} & \textbf{MIMIC III (SS)} \\
\hline
LSTM layers & 1 & 1  \\
 %\cline{1-4}
Learning rate & $0.01,0.005, 0.001, 0.0001$ &  $0.01,0.005, 0.001, 0.0001$ \\
 % %\cline{1-4}
Batch size & $32, 64, 128$ &  $32, 64, 128$ \\
 %\cline{1-4}
LSTM hidden units & $4,6, \dots, 30$ & $4,6, \dots, 30$ \\
%\cline{1-4}
FC hidden units & $4,6, \dots, 30$ &  $4,6, \dots, 30$ \\
 %\cline{1-4}
LSTM dropout rate & - & -  \\
 %\cline{1-4}
R size& $4,6, \dots, 20$& $4,6, \dots, 30$ \\
 %\cline{1-4}
MC samples & 10 & 10 \\
Early Stopping (min delta)& 0.0001&  0.0001\\
Early Stopping (patience)& 30& 30 \\
\cline{1-3}
\end{tabular}%
}
\end{table}

\begin{table}[!htbp]
\centering
\caption{Hyper-parameters search range for Causal Transfomer}
\resizebox{0.7\textwidth}{!}{%
\begin{tabular}{|c|c|c|}
\hline
\textbf{Hyperparameter} & \textbf{Cancer simulation} & \textbf{MIMIC III (SS)} \\
\hline
Transformer blocks & 1 & 1 \\
 %\cline{1-4}
Learning rate & $0.01,0.005, 0.001, 0.0001$ & $0.01,0.005, 0.001, 0.0001$  \\
 %\cline{1-4}
Batch size & $32, 64, 128$ & $32, 64, 128$ \\
 %\cline{1-4}
Attention heads & $2$ & $2$ \\
 %\cline{1-4}
Transformer units & $4,6, \dots, 20$& $4,6, \dots, 20$ \\
 %\cline{1-4}
LSTM dropout rate & -  & - \\
%\cline{1-4}
BR size& $4,6, \dots, 20$&  $4,6, \dots, 20$ \\
%\cline{1-4}
FC hidden units & $4,6, \dots, 20$&   $4,6, \dots, 20$ \\
Sequential dropout rate & $0.1,0.2, 0.3$& $0.1,0.2, 0.3$ \\
Max positional encoding & $15$& $15$  \\
Early Stopping (min delta)& 0.0001& 0.0001 \\
Early Stopping (patience)& 30& 30 \\
\cline{1-3}
\end{tabular}%
}
\end{table}

\begin{table}[!htbp]
\centering
\caption{Hyper-parameters search range for Causal CPC}
\resizebox{0.9\textwidth}{!}{%
\begin{tabular}{|c|c|c|c|c|}
\hline
\textbf{Model} & \textbf{Sub-model} & \textbf{Hyperparameter} & \textbf{Cancer simulation} & \textbf{MIMIC III (SS)} \\
\hline
\multirow{9}{*}{Causal CPC} & \multirow{9}{*}{Encoder} 
& GRU layers & 1 & 1 \\
\cline{3-5}
& & Learning rate & $0.01, 0.005, 0.001, 0.0001$ & $0.01, 0.005, 0.001, 0.0001$ \\
\cline{3-5}
& & Batch size & $32, 64, 128$ & $64, 128, 256$ \\
\cline{3-5}
& & GRU hidden units & $4, 6, \dots, 30$ & $4, 6, \dots, 30$ \\
\cline{3-5}
& & GRU dropout rate & - & - \\
\cline{3-5}
& & Local features (LF) size & $4, 6, \dots, 20$ & $4, 6, \dots, 20$ \\
\cline{3-5}
& & Context Representation (CR) size & $4, 6, \dots, 20$ & $4, 6, \dots, 20$ \\
\cline{3-5}
& & Early Stopping (min delta) & 0.001 & 0.001 \\
\cline{3-5}
& & Early Stopping (patience) & 100 & 100 \\
\hline
\multirow{13}{*}{Decoder} & & GRU layers & 1 & 1 \\
\cline{3-5}
& & Learning rate (decoder w/o treatment sub-network) & $0.01, 0.005, 0.001, 0.0001$ & $0.01, 0.005, 0.001, 0.0001$ \\
\cline{3-5}
& & Learning rate (encoder fine-tuning) & $0.001, 0.0005, 0.0001, 0.00005$ & $0.001, 0.0005, 0.0001, 0.00005$ \\
\cline{3-5}
& & Learning rate (treatment sub-network) & $0.05, 0.01, 0.005, 0.0001$ & $0.05, 0.01, 0.005, 0.0001$ \\
\cline{3-5}
& & Batch size & $32, 64, 128$ & $32, 64, 128$ \\
\cline{3-5}
& & GRU hidden units & CR size & CR size \\
\cline{3-5}
& & GRU dropout rate & - & - \\
\cline{3-5}
& & BR size & CR size & CR size \\
\cline{3-5}
& & GRU layers (Treat Encoder) & 1 & 1 \\
\cline{3-5}
& & GRU hidden units (Treat Encoder) & 6 & 6 \\
\cline{3-5}
& & FC hidden units & $4, 6, \dots, 20$ & $4, 6, \dots, 20$ \\
\cline{3-5}
& & Random time indices (m) & 10\% & 10\% \\
\cline{3-5}
& & Early Stopping (min delta) & 0.001 & 0.001 \\
\cline{3-5}
& & Early Stopping (patience) & 50 & 50 \\
\hline
\end{tabular}%
}
\end{table}
%%%%%%%%%%%%%%%%%%%%%%%%%%%%%%%%%%%%%%%%%%%%%%%%%%%%%%%%%%%%
