# Supplementary material for: Learning Causality for Longitudinal Data
Source: arXiv:2512.04980 source file (2025-12-04)
Supplement: Supplementary file 3 [file 5.tex]

\chapter{Appendix: Chapter \ref{chapter:crl}}

\section{Proofs}

\subsection{Background: Subspace detection in a deterministic model}
% Standard SSL problem 
% static points 
% projections on and coordinates 
% Convex hull and its radius 
% Dual point
% Dual directions
% Subspace incoherence
% THEOREM 2.5
\paragraph{Standard \gls{ssc} problem} In the setting of \citet{elhamifar2013sparse, geometrySSC2012}, we consider data points \(\mathbf{X} = [\mathbf{x}_{1},\dots,\mathbf{x}_{N}] \in \mathbb{R}^{n \times N}\) and we define the \gls{ssc} as 

\begin{equation}
\label{eq:ss_express_standard}
\min_{\mathbf{c}\in\mathbb{R}^N} \|\mathbf{c}\|_{1}
\quad\text{subject to}\quad
\mathbf{X}\,\mathbf{c} = \mathbf{x}_i
\quad\text{and}\quad
\mathbf c_i = 0.
\end{equation}

Let \(\mathbf{X}^{(m)}\in\mathbb{R}^{n\times N_m}\) be the matrix whose columns are the \(N_m\) points on subspace \(\mathcal S_m\). For each \(m=1,\dots,M\) and \(i=1,\dots,N_m\),  we define
\[
\mathbf{X}^{(m)}_{-i}
\;=\;
\bigl[\mathbf{x}^{(m)}_{1},\dots,\mathbf{x}^{(m)}_{i-1},\mathbf{x}^{(m)}_{i+1},\dots,\mathbf{x}^{(m)}_{N_m}\bigr]
\]
which is the matrix obtained by removing the \(i\)-th column from \(\mathbf{X}^{(m)}\).  We can therefore "absorb" the constrating equality \(\mathbf c_i = 0\) of Euation \ref{eq:ss_express_standard} in \(\mathbf{X}_{-i}\) and write

\begin{equation}
\label{eq:ss_express_standard_X_i}
\min_{\mathbf{c}\in\mathbb{R}^N} \|\mathbf{c}\|_{1}
\quad\text{subject to}\quad
\mathbf{X}_{-i}\,\mathbf{c} = \mathbf{x}_i
\end{equation}

To understand when a solution of the optimization problem in \ref{eq:ss_express_standard_X_i}, we turn to the dual problem: 
\begin{equation}
\label{eq:dual_ss_express_standard_X_i}
\max_{\bm{\lambda} \in \mathbb{R}^n} \langle\bm{\lambda}, \mathbf x_i \rangle \quad \text{subject to} \quad \|\mathbf X_{-i}^\top\bm{\lambda}\|_{\infty} \leq 1
\end{equation}

Here, $\lambda \in \mathbb{R}^n$ is a vector in the ambient space whose purpose is to witness/certify the optimality and support of the primal solution. This lead us to the definition of a dual point:

\begin{definition}[Dual point]
\label{def:dual_point}
Consider a point \(\mathbf{x}_i \in \mathbb{R}^n\) , and let \(\mathcal{C}^*(\mathbf{x}_i, \mathbf X_{-i})\) be the set of optimal solutions to\ref{eq:dual_ss_express_standard_X_i}. The \emph{dual point} \(\bm{\lambda}(\mathbf{x}_i, \mathbf X_{-i})\) is defined as the element of \(\mathcal{C}^*(\mathbf{x}_i, \mathbf X_{-i})\) with the minimum Euclidean norm.
\end{definition}

\(\bm{\lambda}(\mathbf{x}_i, \mathbf X_{-i})\) represents the dual certificate for the sparsest code representing \( \mathbf{x}_i \) using atoms in \( \mathbf X_{-i} \).

Next, let \(\mathbf{U}^{(m)}\in\mathbb{R}^{n\times d_m}\) be any orthonormal basis of \(\mathcal S_m\). In this basis, we write
\[
\mathbf{X}^{(m)}
=
\mathbf{U}^{(m)}\,\mathbf{A}^{(m)},
\]
where
\[
\mathbf{A}^{(m)}
=
\bigl[\mathbf{a}_1^{(m)},\dots,\mathbf{a}_{N_m}^{(m)}\bigr]
\;\in\;\mathbb{R}^{d_m\times N_m}
\]
has unit‐norm columns \(\mathbf{a}_i^{(m)}\). The columns of \(\mathbf{A}^{(m)}\) are precisely the coordinates of each point in the orthonormal basis \(\mathbf{U}^{(m)}\).
\begin{definition}[Dual directions]
\label{dualdirectiondef}
For each subspace index \(m\) and data‐point index \(i\), define the \emph{dual direction} \(\mathbf{v}_i^{(m)} \in \mathbb{R}^n\), arranged as columns of the matrix
\[
\mathbf{V}^{(m)}
\;=\;
\bigl[\mathbf{v}_1^{(m)},\,\mathbf{v}_2^{(m)},\,\dots,\,\mathbf{v}_{N_m}^{(m)}\bigr].
\]
These vectors correspond to the dual points
\[
\bm{\lambda}_i^{(m)}
\;=\;
\bm{\lambda}\bigl(\mathbf{a}_i^{(m)},\,\mathbf{A}_{-i}^{(m)}\bigr)
\]
via
\[
\mathbf{v}_i^{(m)}
\;=\;
\mathbf{U}^{(m)} \,\frac{\bm{\lambda}_i^{(m)}}{\|\bm{\lambda}_i^{(m)}\|}.
\]
\end{definition}

The dual direction is nothing but a unit-norm projection of the dual point into the subspace of \(\mathbf{x}_i\) when \(\bm{\lambda}_i^{(m)}\) is the dual point's latent coordinates. Intuitively, it is direction in space that best aligns with \( x_i \), maximizing the inner product \( \langle \lambda, x_i \rangle \), while still respecting the dual constraint \(\| \mathbf X_{-i}^\top \bm{\lambda}\|_{\infty} \leq 1.\)

One of the utilities of dual directions is that it allows us to describe the \textbf{worst-case alignment} between any point from another subspace (i.e., not in $\mathcal{S}_{m}$) and the dual directions $\mathbf{V}^{(m)}$ of that subspace. 

\begin{definition}[Subspace incoherence]
\label{subspaceincoherence}
Let \(\mathcal{X} = \bigcup_{m=1}^M \mathcal{X}_m\) be a union of point sets, and let \(\mathbf{V}^{(m)}\) be the matrix of dual directions for \(\mathcal{X}_m\) as in Definition~\ref{dualdirectiondef}.  The \emph{subspace incoherence} of \(\mathcal{X}_m\) with respect to the other points is
\[
\mu\bigl(\mathcal{X}_m\bigr)
\;=\;
\max_{\mathbf{x}\,\in\,\mathcal{X}\setminus\mathcal{X}_m}
\;\bigl\|\mathbf{V}^{(m)\,T}\,\mathbf{x}\bigr\|_{\ell_\infty}.
\]
\end{definition}

Subspace incoherence quantifies how "confusable" or "close" the directions of external points are to those characterizing the subspace. If \( \mu\bigl(\mathcal{X}_m\bigr)\) is small then no out-of-subspace point aligns strongly with any dual direction of \( \mathcal S^{(m)} \). This helps prevent such points from leaking into the sparse representation of points from \( \mathcal S^{(m)} \).

Subspace incoherence plays a central role in theoretical guarantees in \gls{ssc} and support recovery, as shown in the following theorem of \citet{geometrySSC2012}: let's define
\[
\mathcal{P}(\mathbf{X})
\;\coloneqq\;
\mathrm{conv}\bigl\{\pm \mathbf{x}_1,\;\pm \mathbf{x}_2,\;\dots,\;\pm \mathbf{x}_N\bigr\},
\]
where 
\(\mathrm{conv}(S)\) denotes the convex hull of a set \(S\subseteq\mathbb{R}^n\), i.e.\ the smallest convex set containing \(S\),  and \(\{\pm\mathbf{x}_i\} = \{\mathbf{x}_i,\,-\mathbf{x}_i\}\). Then subspace detection property (\ref{eq:subspace_detect}) is guaranteed under a bounding of the maximum subspace incoherence: 
% Equivalently, one may write
% \[
% \mathcal{P}(\mathbf{X})
% \;=\;
% \Bigl\{\mathbf{y} \in \mathbb{R}^n : 
% \mathbf{y}
% = \sum_{i=1}^N \lambda_i \,\mathbf{x}_i
% - \sum_{i=1}^N \lambda_i' \,\mathbf{x}_i,\quad
% \lambda_i,\lambda_i' \ge 0,\quad 
% \sum_{i=1}^N \lambda_i \;+\;\sum_{i=1}^N \lambda_i' = 1
% \Bigr\}.
% \]
% This shows that every point in \(\mathcal{P}(\mathbf{X})\) can be realized as a convex combination of \(\pm \mathbf{x}_1,\dots,\pm \mathbf{x}_N\).

\begin{theoremBox}[\citet{geometrySSC2012}]
\label{thm:subspace_detect_determin_std}
Suppose that for each \(m = 1,\dots,M\),
\begin{equation}
\label{eq:geom_cond_incoherence}
\mu\bigl(\mathcal{X}_m\bigr)
<
\min_{\,i:\,\mathbf{x}_i\in\mathcal{X}_m}
r\bigl(\mathcal{P}^m_{-i}\bigr).
\end{equation}
Then the subspace‐detection property holds.  Moreover, if \ref{eq:geom_cond_incoherence} is satisfied for a fixed \(m\), then the \emph{local} subspace‐detection property holds in the following sense: for every \(\mathbf{x}_i\in\mathcal{X}_m\), the solution to \ref{eq:ss_express_standard_X_i} can have nonzero entries only at columns of \(\mathbf{X}\) that lie in the same subspace \(\mathcal{X}_m\).
\end{theoremBox}

\subsection{Proof of Theorem \ref{thm:equiv_hard_penalized_prob_j}}
Define Lagrangian for the problem \(\mathcal{P}_t\bigl(Df(\mathbf{Z}),C_{:,j}\bigr)\):
\[
  \mathcal{L}_t(C_{:,j},\lambda,\nu)
  = \|C_{:,j}\|_1
    + \lambda\bigl(\ell_j(C_{:,j})-t\bigr)
    + \nu\,C_{j,j},
  \quad
  \lambda\ge0,\;\nu\in\mathbb{R},
\]
where \(\lambda\) and \(\nu\) are the multipliers for the constraints \(\,\ell_j(C_{:,j})\le t\) and \(c_j=0\), respectively.

Since
\begin{itemize}
  \item \(\ell_j(\cdot)\) is continuous and convex (indeed strictly convex quadratic if \(\mathbb{E}_{\mathbf{Z}}\bigl[\,Df(\mathbf Z)^{\!\top}Df(\mathbf Z)\bigr]\) is positive definite),
  \item \(\|\cdot\|_1\) is convex,
  \item there exists a feasible solution \(C_{:,j}^\star\) to \(\mathcal{P}_t\bigl(Df(\mathbf{Z}),C_{:,j}\bigr)\), that is, with \(\ell_j(C_{:,j}^\star)<t\) and \(C_{j,j}^\star=0\) (e.g.\ \(C_{:,j}^\star=\mathbf 0\) if \(t>\ell_j(\mathbf 0)\)), 
\end{itemize}
Slater’s condition holds (one inequality plus one equality), so strong duality applies. 

Let  $C_{:,j}^{\mathrm{LS}} = \arg \min_{C_{:,j} \in \mathbb R^{d_x} \quad C_{j,j}=0} \ell_j(C_{:,j})$, the solutions exists and is unique by strict convexity of \(\ell_j(\cdot)\).

\textbf{KKT system}

A triple \((C_{:,j}^*,\lambda^*,\nu^*)\) solves \(\mathcal{P}_t\bigl(Df(\mathbf{Z}),C_{:,j}\bigr)\) if and only if it satisfies the following KKT conditions:

\begin{align*}
  &\text{Primal feasibility:}
    &&\ell_j(C_{:,j}^*) \le t,\quad C_{j,j}^*= 0,
    &&\quad (K1)\\
  &\text{Dual feasibility:}
    &&\lambda^* \ge 0,
    &&\quad (K2)\\
  &\text{Complementary slackness:}
    &&\lambda^* \bigl(\ell_j(C_{:,j}^*) - t\bigr) = 0,
    &&\quad (K3)\\
  &\text{Stationarity:}
    &&0 \;\in\; \partial\|C_{:,j}^*\|_1 \;+\;\lambda^*\,\nabla \ell_j(C_{:,j}^*) \;+\;\nu^*\,\mathbf e_j,
    &&\quad (K4)
\end{align*}

Here \(\mathbf e_j\) denotes the \(j\)-th standard basis vector in \(\mathbb{R}^{d_x}\).

Because \(\ell_j\) it is strictly convex and there is only a single equality constraint \(C_{j,j}=0\), the stationarity condition (K4) uniquely determines \((C_{:,j}^*,\nu^*)\) it once \(\lambda^*\) is fixed.  Moreover, complementary slackness (K3) forces \(\lambda^*>0\) whenever \(\ell_j(C_{:,j}^*)<t\) is impossible—i.e.\ for all \(t>\ell_j(C_{:,j}^{\mathrm{LS}})\).

Consider now the penalized problem  \(\mathcal{P}_{\lambda}(Df(\mathbf{Z}), C_{:,j})\), whose Lagrangian is
\begin{equation}\label{eq:LL}
\mathcal{L}_{\lambda}(C_{:,j},\nu)
= \ell_j(C_{:,j}) \;+\; \lambda\,\|C_{:,j}\|_1 \;+\; \nu\,C_{j,j},
\qquad
\nu\in\mathbb{R}.
\end{equation}
Its first‐order optimality (stationarity) condition reads
\begin{equation}\label{eq:stationarity_L}
\mathbf 0 \;\in\; \nabla \ell_j(C_{:,j}^*)
  \;+\;\lambda\,\partial\|C_{:,j}^*\|_1
  \;+\;\nu^*\, \mathbf e_j.
\end{equation}
Comparing \eqref{eq:stationarity_L} with (K4) shows that any \((C_{:,j}^*,\lambda^*,\nu^*)\) satisfying the KKT system for \(\mathcal{P}_t\bigl(Df(\mathbf{Z}),C_{:,j}\bigr)\) also satisfies \eqref{eq:stationarity_L} with \(\lambda=\lambda^*\).  Together with the common constraint \(c_j^*=0\), we obtain: If \(c^*\) solves \(\mathcal{P}_t\bigl(Df(\mathbf{Z}),C_{:,j}\bigr)\) with multipliers \((\lambda^*,\nu^*)\), then \(C_{:,j}^*\) also solves  \(\mathcal{P}_{\lambda}(Df(\mathbf{Z}), C_{:,j})\) under the constraint \(C_{j,j}=0\).

\textbf{Bijection between \(\lambda\) and \(t\)} Define the penalized‐solution path (respecting \(c_j=0\)):
\begin{equation}
    \label{eq:sol_path_penalized}
      C_{:,j}^*(\lambda)
  := \arg\min_{\substack{C_{:,j}\in\mathbb{R}^{d_x}\\C_{j,j}=0}}
     \bigl\{\,\ell_j(C_{:,j}) + \lambda\,\|C_{:,j}\|_1\bigr\}.
\end{equation}
By strict convexity of \(\ell_j\), convexity of \(\|\cdot\|_1\), and the affine constraint \(C_{j,j}=0\), the minimiser \(C_{:,j}^*(\lambda)\) is unique.  Now set
\[
  t_j(\lambda)
  := \ell_j\bigl(C_{:,j}^*(\lambda)\bigr).
\]
$\lambda \longrightarrow t_j(\lambda)$ is continuous and piecewise linear (Proposition 1 \citep{rosset2007piecewiseLassoPath}) and  strictly decreasing; its limit values are the following

As \(\lambda\to0^+\), the penalty vanishes and \(C_{:,j}^*(\lambda)\to C_{:,j}^{\mathrm{LS}}\)   Thus
\[
  \lim_{ \lambda\to0^+}t_j(\lambda)=\ell_j\bigl(C_{:,j}^{\mathrm{LS}}\bigr).
\]

As \(\lambda\to\infty\), the \(\lambda\|C_{:,j}\|_1\) term dominates in Equation \ref{eq:sol_path_penalized}, forcing \(C_{:,j}^*(\lambda)\to \mathbf 0\); hence
\[
\lim_{ \lambda\to \infty}  t_j(\lambda)=\ell_j(\mathbf 0).
\]

Therefore
\[
  t\colon (0,\infty)\;\longrightarrow\;\bigl[\,\ell_j\bigl(C_{:,j}^{\mathrm{LS}}\bigr),\,\ell_j(\mathbf 0)\bigr)
\]
is a continuous bijection. Note that since we assume self-expressiveness \ref{assp:self_expression} \(\ell_j\bigl(C_{:,j}^{\mathrm{LS}}\bigr) = 0\)

Given any 
\[
  t_j^\star \;\in\;\bigl[\,\ell_j\bigl(C_{:,j}^{\mathrm{LS}}\bigr),\,\ell_j(\mathbf 0)\bigr),
\]
continuity and bijectivity of \(t_j(\cdot)\) guarantee a unique \(\lambda_j \ge 0\) such that 
\[
  t_j(\lambda_j) =  t_j^\star.
\]
At that \(\lambda_j\), the solution \(C_{:,j}^*(\lambda_j)\) of \(\mathcal{P}_{\lambda}(Df(\mathbf{Z}), C_{:,j})\) satisfies 
\[
  \ell_j\bigl(C_{:,j}^*(\lambda)\bigr) = t_j^\star
  \quad\text{and}\quad
  \mathbf 0\;\in\;\nabla \ell_j(C_{:,j}^*(\lambda_j)) + \lambda_j\,\partial\|C_{:,j}^*(\lambda_j)\|_1 + \nu^*\,\mathbf e_j,
\]
which matches the stationarity KKT condition (K4) for \(\mathcal{P}_t\bigl(Df(\mathbf{Z}),C_{:,j}\bigr)\).  Hence \(C_{:,j}^*(\lambda_j)\) is also the minimizer of \(\mathcal{P}_t\bigl(Df(\mathbf{Z}),C_{:,j}\bigr)\).  This establishes a one-to-one correspondence \(\lambda\) and \(t\).

\subsection{High-Probability Guarantee for Subspace Detection}
\label{proof:subspace_detect_whp}
We provide in this section the proof of Theorem  \ref{thm:subspace_detect_whp}. We recall that \( \mathbf{Z} \in \mathrm{subG}_{d_z}(K) \) (Definition \ref{def:Z_subgauss_vector}) and the smoothness assumption (\ref{assp:smooth_f}) over \(f\): the decoder \( f \in \mathcal{C}^2(\mathbb{R}^{d_z}; \mathbb{R}^{d_x}) \) is twice continuously differentiable, with uniformly bounded curvature. That is, for each output coordinate \( f_i \), the Hessian satisfies
\[
\sup_{\mathbf{z} \in \mathbb{R}^{d_z}} \| D^2 f_i(\mathbf{z}) \|_{\mathrm{op}} \le L, \quad \text{for all } i \in \llbracket 1, d_x \rrbracket.
\]
Define the gradient vectors:
\[
P_i(\mathbf{Z}) := \nabla f_i(\mathbf{Z}) \in \mathbb{R}^{d_z}, \quad i = 1, \dots, d_x,
\]
and let the symmetric convex polytope \( \mathcal{K}(\mathbf{Z}) \subset \mathbb{R}^{d_z} \) be given by:
\[
\mathcal{K}(\mathbf{Z}) := \mathrm{conv}\left(\pm P_1(\mathbf{Z}), \dots, \pm P_{d_x}(\mathbf{Z})\right).
\]
Let the in-radius of \( \mathcal{K}(\mathbf{Z}) \) be defined by:
\[
r(\mathbf{Z}) := r(\mathcal{K}(\mathbf{Z})) = \min_{\mathbf{u} \in \mathbb{S}^{d_z-1}} \max_{1 \le i \le d_x} |\langle P_i(\mathbf{Z}), \mathbf{u} \rangle|.
\]
\begin{lemma}[Concentration of the in-radius of the Gradient Polytope]
\label{lemma:concentration_r(K)}
The in-radius of \( \mathcal{K}(\mathbf{Z}) \) has the concentration inequality:
\[
\mathbb{P}\left( \left| r(\mathbf{Z}) - \mathbb{E} r(\mathbf{Z}) \right| \ge t \right) \le 2 \exp\left( -\frac{t^2}{2K^2L^2} \right).
\]
Moreover, the expected in-radius is bounded by:
\[
\mathbb{E} \, r(\mathbf{Z}) \le \Lambda_1 \, K \, L \, \sqrt{ \frac{\log(d_x/d_z)}{d_z} },
\]
for a universal constant \( \Lambda _1> 0 \).
In particular, we have the one-sided, lower tail bound over the in-radius: 
\begin{equation}
    \label{eq:inradius_lower_tail_bnd}
    \mathbb{P} \Bigl\{r(\mathbf{Z})<\,\Lambda_1\,K\,L\,\sqrt{\tfrac{\log d_x}{d_z}}\Bigr\}
\;\le\;
\exp\!\Bigl(-\tfrac{\Lambda_1^2\,\log(d_x)}{2\,d_z}\Bigr).
\end{equation}
\end{lemma}

%\begin{proof}
\begin{proof} 
\textbf{In-radius Concentration}
Since  \( \|D^2 f_i(\mathbf{z})\|_{\mathrm{op}} \le L \) for all \( i \in [d_x] \) and \( \mathbf{z} \in \mathbb{R}^{d_z} \), the gradient map \( z \mapsto P_i(\mathbf{z}) = \nabla f_i(\mathbf{z}) \in \mathbb{R}^{d_z} \) is \(L\)-Lipschitz for each \(i\), i.e.,
\[
\|P_i(\mathbf{z}) - P_i(\mathbf{z}')\| \le L \|\mathbf{z} - \mathbf{z}'\|.
\]
For any fixed unit vector \( \mathbf{u} \in \mathbb{S}^{d_z-1} \), define the support function:
\[
\phi_{\mathbf{u}}(\mathbf{Z}) := \max_{1 \le i \le d_x} |\langle P_i(\mathbf{Z}), \mathbf{u} \rangle|.
\]
Since each \( P_i \) is \(L\)-Lipschitz, it follows that \( \phi_{\mathbf{u}}(\mathbf{Z}) \) is also \(L\)-Lipschitz. Moreover, the in-radius
\[
r(\mathbf{Z}) := \inf_{\mathbf{u} \in \mathbb{S}^{d_z-1}} \phi_{\mathbf{u}}(\mathbf{Z})
\]
is also \(L\)-Lipschitz as an infimum over a uniformly Lipschitz family. Therefore,
\[
|r(\mathbf{Z}) - r(\mathbf{Z}')| \le L \|\mathbf{Z} - \mathbf{Z}'\| \quad \text{for all } \mathbf{Z}, \mathbf{Z}' \in \mathbb{R}^{d_z}.
\]
Since \( \mathbf{Z} \) is sub-Gaussian with constant \( K \), applying standard concentration for Lipschitz functions of sub-Gaussian variables \citep{vershynin2018HDProba} gives:
\[
\mathbb{P}\left( \left| r(\mathbf{Z}) - \mathbb{E} r(\mathbf{Z}) \right| \ge t \right)
\le 2 \exp\left( - \frac{t^2}{2 K^2 L^2} \right),
\]
which proves the first part.

\textbf{Bound on the Expected in-radius.}
We now estimate the mean value \( \mathbb{E} r(\mathbf{Z}) \). Since
\[
r(\mathbf{Z}) = \inf_{u \in \mathbb{S}^{d_z-1}} \max_{1 \le i \le d_x} |\langle P_i(\mathbf{Z}), \mathbf{u} \rangle| = \inf_{u \in \mathbb{S}^{d_z-1}} \max_{1 \le i \le d_x} X_{i,\mathbf{u}}(\mathbf{Z}),
\]
we define the stochastic process:
\[
X_{i,\mathbf{u}}(\mathbf{Z}) :=|\langle P_i(\mathbf{Z}), \mathbf{u} \rangle|.
\]
Each map \( \mathbf{Z} \mapsto X_{i,\mathbf{u}}(\mathbf{Z}) \) is \(L\)-Lipschitz and hence sub-Gaussian with norm at most \( K L \). Furthermore, for any pairs \( (i,\mathbf{u}), (j,\mathbf{v}) \in  \llbracket 1, d_x \rrbracket \times \mathbb{S}^{d_z-1} \),
\[
|X_{i,\mathbf{u}}(\mathbf{Z}) - X_{j,\mathbf{v}}(\mathbf{Z}')| \le L \|\mathbf{Z} -\mathbf{Z}'\|(1 + \|\mathbf{u} - \mathbf{v}\|),
\]
implying the variance proxy:
\[
\rho((i,\mathbf{u}), (j,\mathbf{v})) := K L \left( \mathbf{1}_{i \ne j} + \|\mathbf{u} - \mathbf{v}\| \right).
\]
Hence, the collection \( \{X_{i,\mathbf{u}}(\mathbf{Z})\} \) is a \( \rho \)-sub-Gaussian process over the index set \( T =  \llbracket 1, d_x \rrbracket \times \mathbb{S}^{d_z-1} \).

By Dudley's entropy integral bound for sub-Gaussian processes:
\[
\mathbb{E} \sup_{(i,\mathbf{u}) \in T} X_{i,\mathbf{u}}(\mathbf{Z})
\le C \int_0^{\mathrm{diam}(T)} \sqrt{ \log N(T, \rho; \varepsilon) } \, d\varepsilon,
\]
where \( N(T, \rho; \varepsilon) \) is the \( \varepsilon \)-covering number of \( T \) under \( \rho \), and \( \mathrm{diam}(T) \le K L (2 + \pi) \).

To bound the covering number: The discrete index set \( \llbracket 1, d_x \rrbracket\) contributes a factor of \( d_x \). The unit sphere \( \mathbb{S}^{d_z-1} \) has \( \varepsilon \)-covering number at most \( (3 / \delta)^{d_z} \) in Euclidean norm, where \( \delta = \varepsilon / (K L) \). Thus,
    \[
    N(T, \rho; \varepsilon) \le d_x \left( \frac{3 K L}{\varepsilon} \right)^{d_z}.
    \]
Plugging into Dudley’s integral gives:
\[
\mathbb{E} \sup_{(i,\mathbf{u})} X_{i,\mathbf{u}}(\mathbf{Z})
\le \Lambda_1 K L \int_0^{2 K L} \sqrt{ \log d_x + d_z \log(3 K L / \varepsilon) } \, d_z\varepsilon
\lesssim K L \sqrt{ \frac{\log d_x}{d_z} },
\]
where the last step follows from standard integral splitting and evaluation \citep{ledoux2001concentration}.

Since \( r(\mathbf{Z}) = \inf_{\mathbf{u} \in \mathbb{S}^{d_z-1}} \max_{1 \le i \le d_x}  X_{i,\mathbf{u}}(\mathbf{Z}) \le \sup_{(i,\mathbf{u})}  X_{i,\mathbf{u}}(\mathbf{Z}) \), it follows that:
\[
\mathbb{E} r(\mathbf{Z}) \le \mathbb{E} \sup_{(i,\mathbf{u})} X_{i,\mathbf{u}}(\mathbf{Z}) \lesssim K L \sqrt{ \frac{\log d_x}{d_z} }.
\]

\textbf{In-radius lower tail bound} Since for each \(t > 0\)
\[
\mathbb{P}\left( \left| r(\mathbf{Z}) - \mathbb{E} r(\mathbf{Z}) \right| \ge t \right) \le 2 \exp\left( -\frac{t^2}{2K^2L^2} \right),
\]
and given \(\mathbb{E}[r(\mathbf{Z})]\le \Lambda_1 \,K\,L\,\sqrt{\tfrac{\log(d_x)}{d_z}}\), then setting \(t=\tfrac12\,\mathbb{E}[r(\mathbf Z)]\) yields
\[
\mathbb{P} \Bigl\{r(\mathbf{Z})<\tfrac12\,\Lambda_1\,K\,L\,\sqrt{\tfrac{\log d_x}{d_z}}\Bigr\}
\;\le\;
2 \exp\!\Bigl(-\tfrac{\Lambda_1^2\,\log(d_x)}{8\,d_z}\Bigr),
\]

or equivalently
\[
\mathbb{P} \Bigl\{r(\mathbf{Z})<\,\Lambda_1\,K\,L\,\sqrt{\tfrac{\log d_x}{d_z}}\Bigr\}
\;\le\;
\exp\!\Bigl(-\tfrac{\Lambda_1^2\,\log(d_x)}{2\,d_z}\Bigr).
\]
\end{proof}

\begin{lemma}[Frobenius-Norm Tail and Expectation Bounds]
\label{lemma:bound_norm_max}
Let
\[
\mathbf{A} = [\mathbf{a}_1, \dots, \mathbf{a}_{N_1}] \in \mathbb{R}^{d_1 \times N_1}, \quad
\mathbf{a}_i \overset{\mathrm{iid}}{\sim} \mathrm{Unif}(\mathbb{S}^{d_1 - 1}),
\]
and let \(\Sigma \in \mathbb{R}^{d_1 \times d_2}\) be deterministic, and \(\lambda \overset{\mathrm{iid}}{\sim} \mathrm{Unif}(\mathbb{S}^{d_2 - 1})\) independent of \(\mathbf{A}\). Define
\[
X_i := \langle \mathbf{a}_i, \Sigma \lambda \rangle, \qquad
\sigma_i^2 := Var(X_i \mid \mathbf{a}_i) = \frac{\| \Sigma^\top \mathbf{a}_i \|_2^2}{d_2}, \qquad
\sigma_{\max} := \max_{1 \le i \le N_1} \sigma_i.
\]
Then there exist universal constants \(\Lambda_2 > 0\) such that, for all \(t > 0\),
\begin{enumerate}
  \item[(i)] \emph{High-Probability Tail Bound.}
  \[
    \mathbb{P}\left\{
      \max_{1 \le i \le N_1} |X_i| > \mathbb{E} \left[ \max_i |X_i| \right] + t
    \right\}
    \le
    2 \exp\left( -\,\,\frac{d_2\,t^2}{2\|\Sigma\|_F^2} \right).
  \]
  \item[(ii)] \emph{Expectation Bound.}
  \[
    \mathbb{E} \left[ \max_{1 \le i \le N_1} |X_i| \right]
    \le
    \Lambda_2\,\frac{\|\Sigma\|_F}{\sqrt{d_2}} \, \sqrt{ \log(N_1 + 1) }.
  \]
\end{enumerate}
In particular, we have the one-sided tail bound:
\begin{equation}
\label{eq:bound_norm_max_lower_tail_bnd}
\mathbb{P}\left\{
\max_{1 \le i \le N_1} |X_i|
\leq (1 + \Lambda_2) \frac{\|\Sigma\|_F}{\sqrt{d_2}} \sqrt{\log(N_1 + 1)}
\right\}
\geq
 1 - \frac{2}{\sqrt{N_1 + 1}}.
\end{equation}
\end{lemma}

\begin{proof}
\textbf{Step 1: Concentration of individual terms.}  
For each fixed \( \mathbf{a}_i \), the function \( \lambda \mapsto X_i(\lambda) = \langle \mathbf{a}_i, \Sigma \lambda \rangle \) is \( \|\Sigma^\top \mathbf{a}_i\|_2 \)-Lipschitz on the sphere \( \mathbb{S}^{d_2 - 1} \). By Lévy’s lemma on the sphere (see \cite{ledoux2001concentration,vershynin2018HDProba}), for all \( \epsilon > 0 \),
\[
\mathbb{P}\left\{ \left| X_i - \mathbb{E}[X_i \mid \mathbf{a}_i] \right| \ge \epsilon \;\middle|\; \mathbf{a}_i \right\}
\le
2 \exp\left( -\,\,\frac{d_2\,\epsilon^2}{2\| \Sigma^\top \mathbf{a}_i \|_2^2} \right).
\]
Since \( \mathbb{E}[X_i \mid \mathbf{a}_i] = 0 \), we conclude \( X_i \mid \mathbf{a}_i \) is sub-Gaussian with proxy \( \sigma_i = \|\Sigma^\top \mathbf{a}_i\|_2 / \sqrt{d_2} \).

\textbf{Step 2: Concentration of the maximum.}  
Define
\[
F(\lambda) := \max_{1 \le i \le N_1} |X_i(\lambda)|.
\]
Conditioned on \(\mathbf{A}\), each \(X_i\) is fixed and \(F(\lambda)\) is \( \sigma_{\max} \)-Lipschitz over \( \mathbb{S}^{d_2 - 1} \). Applying Lévy’s lemma \citep{milman1986asymptotic} gives
\[
\mathbb{P}\left\{
  F(\lambda) - \mathbb{E}[F(\lambda) \mid \mathbf{A}] > t \;\middle|\; \mathbf{A}
\right\}
\le
2 \exp\left( -\,c\,\frac{d_2\,t^2}{\sigma_{\max}^2} \right)
\le
2 \exp\left( -\,c\,\frac{d_2\,t^2}{\|\Sigma\|_F^2} \right),
\]
where the final inequality uses \( \sigma_{\max} \leq \frac{\|\Sigma\|_F}{\sqrt{d_2}} \). Averaging over \(\mathbf{A}\) completes the proof of part (i).

\textbf{Step 3: Expectation via Dudley’s entropy integral.}  
Conditioned on \(\mathbf{A}\), the collection \( \{X_i\}_{i=1}^{N_1} \) forms a finite sub-Gaussian process indexed by \( \{1, \dots, N_1\} \). Dudley’s theorem implies \citep{talagrand2005generic}
\[
\mathbb{E}[F(\lambda) \mid \mathbf{A}]
\le
\Lambda_2 \int_{0}^{\sigma_{\max}} \sqrt{ \log N_1 } \, d\varepsilon
= \Lambda_2 \, \sigma_{\max} \sqrt{ \log N_1 }.
\]
Since \( \sigma_{\max} \leq \frac{\|\Sigma\|_F}{\sqrt{d_2}} \), we conclude
\[
\mathbb{E} \left[ \max_{1 \le i \le N_1} |X_i| \right]
= \mathbb{E}[F(\lambda)]
\le
\Lambda_2\, \frac{\|\Sigma\|_F}{\sqrt{d_2}} \, \sqrt{ \log(N_1 + 1) },
\]
completing part (ii).

\textbf{Step 4: One-sided tail bound.} Since
  \[
    \mathbb{P}\left\{
      \max_{1 \le i \le N_1} |X_i| > \mathbb{E} \left[ \max_i |X_i| \right] + t
    \right\}
    \le
    2 \exp\left( -\,\,\frac{d_2\,t^2}{2\|\Sigma\|_F^2} \right),
  \]
and given the expectation bound
  \[
    \mathbb{E} \left[ \max_{1 \le i \le N_1} |X_i| \right]
    \le
    \Lambda_2 \frac{\|\Sigma\|_F}{\sqrt{d_2}} \, \sqrt{ \log(N_1 + 1) },
  \]
  then choosing \(t =  \frac{\|\Sigma\|_F}{\sqrt{d_2}} \, \sqrt{ \log(N_1 + 1) } \)  yield

\[
\mathbb{P}\left\{
  \max_{1 \le i \le N_1} |X_i|
  \leq (1 + \Lambda_2) \frac{\|\Sigma\|_F}{\sqrt{d_2}} \sqrt{\log(N_1 + 1)}
\right\}
\geq
1 - 2 \exp\left( -\frac{1}{2} \log(N_1 + 1) \right)
= 1 - \frac{2}{\sqrt{N_1 + 1}}.
\]
\end{proof}
Let \(\mathcal{P}^m_{-i} \coloneqq \mathcal{P}(\mathbf{X}_{-i}^m)\), then application of Lemma \ref{lemma:concentration_r(K)} yields  
\begin{equation}
\label{eq:boundonrad}
\qquad \mathbb{P} \biggl\{
\Lambda_1\,K\,L\,\sqrt{\tfrac{\log n_m}{d_m}}
\le r \bigl(
\mathcal{P}^m_{-i} \bigr) \mbox{ for all pairs } (m,i)
\biggr\} 
\ge 
1-\sum_{m=1}^M  n_m
\exp\!\Bigl(-\tfrac{\Lambda_1^2\,\log(n_m)}{2\,d_m}\Bigr).
\end{equation}

On the other hand, by noticing that 
\begin{equation}
\label{eq:contmu}
\begin{aligned}
\left\| \mathbf{X}^{(k)^\top} \mathbf{V}^{(\ell)} \right\|_{\ell_\infty}
&= \max_{i = 1, \ldots, N_\ell} \left\| \mathbf{X}^{(k)^\top} \mathbf{v}_i^{(\ell)} \right\|_{\ell_\infty} \\
&= \max_{i = 1, \ldots, N_\ell} \left\| \mathbf{A}^{(k)^\top} \mathbf{U}^{(k)^\top} \mathbf{U}^{(\ell)} \frac{\boldsymbol{\lambda}_i^{(\ell)}}{\|\boldsymbol{\lambda}_i^{(\ell)}\|_2} \right\|_{\ell_\infty},
\end{aligned}
\end{equation}

and that \(\operatorname{aff}(\mathcal{S}_k, \mathcal{S}_m) =  \|\mathbf{U}^{(k)^\top} \mathbf{U}^{(m)} \|_F \) \citep{geometrySSC2012}, an application of \ref{lemma:bound_norm_max} to Equation \ref{eq:contmu} yields 

\[
\mathbb{P}\left\{
  \left\| \mathbf{X}^{(k)^\top} \mathbf{V}^{(m)} \right\|_{\ell_\infty}
  \leq (1 + \Lambda_2) \frac{\operatorname{aff}(\mathcal{S}_k, \mathcal{S}_m)}{\sqrt{d_2}} \sqrt{\log(n_m + 1)}
\right\}
\geq
 1 - \frac{2}{\sqrt{n_m + 1}}.
\]
 and therefore 
 \begin{equation}
\label{eq:unfbound}
\begin{aligned}
\mathbb{P}\biggl\{\,%
  \bigl\| \mathbf{X}^{(k)\top}\mathbf{V}^{(m)} \bigr\|_{\ell_\infty}
  &\le (1+\Lambda_2)\,\frac{\operatorname{aff}\bigl(\mathcal{S}_k, \mathcal{S}_m\bigr)}{\sqrt{d_2}}\,
        \sqrt{\log(n_m + 1)}\\[-0.5ex]
  &\quad \text{for all } (m, k)\ \text{with } m \ne k
\biggr\}
\;\ge\;
1 - \sum_{1 \le k \ne m \le M} \frac{2}{\sqrt{n_m + 1}}\\[-0.5ex]
&= 1 - \sum_{m=1}^M \frac{2(M-1)}{\sqrt{n_m + 1}}.
\end{aligned}
\end{equation}

As a consequence of Equations \ref{eq:unfbound}  and\ref{eq:boundonrad}, if we impose the condition 

\[
\max_{k \neq m} \Lambda_2' \, \operatorname{aff}(\mathcal{S}_k, \mathcal{S}_m) \frac{\sqrt{\log(n_k + 1)}}{\sqrt{d_m}} 
\leq \Lambda_1\,K\,L\,\sqrt{\frac{\log n_m}{d_m}},
\]
which is equivalent to saying
\begin{equation}
    \label{eq:incherence_con}
    \max_{k \neq m} \operatorname{aff}(\mathcal{S}_k, \mathcal{S}_m) \sqrt{\log(n_k + 1)} 
\leq \Lambda\,K\,L\,\sqrt{\log n_m}, \quad \text{with } \Lambda = \frac{\Lambda_1}{\Lambda_2'},
\end{equation}
then the subspace detection property holds with probability
\[
1 - \sum_{m=1}^M n_m \exp\!\left(-\frac{\Lambda_1^2 \log(n_m)}{2 d_m}\right) 
- \frac{2(M - 1)}{\sqrt{n_m + 1}}.
\]
The condition of Equation \ref{eq:incherence_con} is exactly that of Theorem \ref{thm:subspace_detect_whp}.

\subsection{Recovery of Feature Clusters via Spectral Clustering}
We now prove Proposition \ref{prop:recovery_nonoverlap_spec_cltsr}. We show that spectral clustering on the affinity matrix
\[
A = |C^*| + |C^*|^\top
\]
recovers with high probability the connected components of the feature graph $G_F$ under standard \gls{ssc} assumptions. Since we assume the incoherence gap of Theorem \ref{thm:subspace_detect_whp} holds, then by the same theorem, the subspace detection property holds, and therefore classical results on subspace clustering apply with high probability. In the following, we detail the arguments for cluster recovery with spectral clustering; we omit the expression "with high probability" for better readability.

\paragraph{Union-of-Subspaces from Latent Structure}
Let feature $i$ have latent-parent set $\mathrm{Pa}(i) \subseteq [d_z]$. Then the Jacobian row can be written as
\[
Df_{i,:}(\mathbf{Z}) = \nabla_{\mathbf{z}} f_i(\mathbf{Z})^\top = \sum_{j \in \mathrm{Pa}(i)} \alpha_{i,j}(\mathbf{Z})\, \mathbf{e}_j^\top,
\]
so each $Df_{i,:}(\mathbf{Z})$ lies in a union of low-dimensional subspaces spanned by subsets of $\{\mathbf{e}_j\}$. This corresponds to a union-of-subspaces model \citep{geometrySSC2012}.

\paragraph{\gls{ssc} Self-Expression Recovers Graph Structure}
We solve the population Lasso problem:
\[
\mathbf{C}^* = \arg\min_{\substack{\mathbf{C} \in \mathbb{R}^{d_x \times d_x} \\ \operatorname{diag}(\mathbf{C}) = 0}} \; \mathbb{E}_{\mathbf{Z}} \left[ \|Df(\mathbf{Z}) - \mathbf{C} Df(\mathbf{Z})\|_F^2 \right] + \lambda \|\mathbf{C}\|_1.
\]
Under standard \gls{ssc} conditions, such as subspace incoherence and low-noise \citep{elhamifar2013sparse}, we have:
\[
\mathbf{C}^*_{ii'} \ne 0 \quad \Leftrightarrow \quad \mathrm{Pa}(i) \cap \mathrm{Pa}(i') \ne \varnothing.
\]
Define the affinity matrix $\mathbf{A} = |\mathbf{C}^*| + |\mathbf{C}^*|^\top$. Then the support of $\mathbf{A}$ corresponds exactly to the edge set of the feature graph $G_F$.

\paragraph{Connected Components from Laplacian Nullspace}
Let $\mathbf{D} = \operatorname{diag}(\mathbf{A}\mathbf{1})$ and form the symmetric normalized Laplacian
\[
\mathbf{L}_{\mathrm{sym}} = \mathbf{I} - \mathbf{D}^{-1/2} \mathbf{A} \mathbf{D}^{-1/2}.
\]
It is well known \citep{von2007tutorialSpectrCls} that the multiplicity of the zero eigenvalue of $\mathbf{L}_{\mathrm{sym}}$ equals the number of connected components in $G_F$, and its nullspace is spanned by indicator vectors of those components.

\paragraph{Recovery via Spectral Clustering}
Spectral clustering (e.g., Ng–Jordan–Weiss variant) computes the first $k$ eigenvectors of $\mathbf{L}_{\mathrm{sym}}$, stacks them into a matrix $\mathbf{U} \in \mathbb{R}^{d_x \times k}$, and applies $k$-means to its rows. In the exact block-diagonal case, these rows are standard basis vectors corresponding to the true partition, so clustering achieves zero error \citep{ng2001spectral}.

\subsection{Guarantees of features grouping via clustering techniques}
We now prove Theorem~\ref{thm:overlap_cluster_recovery}. We break the argument into six main steps:
\begin{enumerate}[label=\textbf{\arabic*.}, wide, labelwidth=!, labelsep=1em, leftmargin=*]
    \item \textbf{Concentration of Gram entries (Step 1)} we show that with high probability
    \[
    \|\widehat\Sigma-\Sigma\|_\infty
    \]
    is of order \(O(KL\sqrt{d_x\log(d_x^2/\varepsilon)})\).

    \item \textbf{Restricted strong convexity (Step 2)} we prove that the population and empirical Lasso risks are strongly convex on \(s\)‑sparse rows, guaranteeing a unique minimizer.

    \item \textbf{Support recovery via primal–dual witness (Step 3 \& 4)} uses mutual incoherence and dominance to show that all off‑support coefficients vanish and that in‑group coefficients are large.

    \item \textbf{Affinity block bounds (Step 5)} translates the coefficient bounds into lower and upper bounds on the entries of the affinity matrix \(A^*\).

    \item \textbf{Spectral perturbation and rounding (Step 6)} we control the eigenspace deviation \(O(\|E\|_2/\Delta)\) and show that both SAAC and SymNMF recover the true (possibly overlapping) clusters up to the stated error rate.
\end{enumerate}

\subsection*{Step 1: Concentration of Inner-Product Entries}

We begin by controlling the entries of the empirical Gram matrix \(\widehat{\bm\Sigma}\), whose \((i,i')\)–th entry is
\[
g_{ii'}(\bm Z)
=\bigl\langle \partial_i f(\bm Z),\,\partial_{i'}f(\bm Z)\bigr\rangle.
\]
This uniform control is essential for later bounding the population Lasso risk.

First, the vector mean–value theorem tells us that for any \(\bm z,\bm z'\in\mathbb R^{d_z}\),
\[
\nabla f_i(\bm z)-\nabla f_i(\bm z')
=\int_{0}^{1}
D^2f_i\bigl(\bm z + t(\bm z'-\bm z)\bigr)\,(\bm z'-\bm z)\,dt.
\]
Since \(\|D^2f_i\|_{\mathrm{op}}\le L\) by Assumption \ref{assp:smooth_f}, it follows immediately that
\[
\|\nabla f_i(\bm z)-\nabla f_i(\bm z')\|
\le L\,\|\bm z'-\bm z\|,
\]
so each coordinate gradient \(\partial_i f(\bm z)\) is \(L\)–Lipschitz in \(\bm z\).

Turning next to the inner‐product function itself, differentiation yields
\[
\nabla g_{ii'}(\bm z)
=\sum_{\ell\in\{i,i'\}}
D^2f_\ell(\bm z)\,\partial_{\ell'}f(\bm z).
\]
Again, using \(\|D^2f_\ell\|_{\mathrm{op}}\le L\) together with the bounded‐Jacobian condition \(\sup_{\bm z}\|Df(\bm z)\|_F = \sqrt{d_x}\), we deduce
\[
\|\nabla g_{ii'}(\bm z)\|
\le 2\,L\, \sqrt{d_x},
\]
so \(g_{ii'}\) is \(2L\sqrt{d_x}\)–Lipschitz.

Because \(\bm Z\) is \(K\)–sub‐Gaussian, the Borell–Tsirelson–Ibragimov–Sudakov inequality \citep{SudakovTsirelson1978} applies to any \(2L\sqrt{d_x}\)–Lipschitz function of \(\bm Z\).  In particular, for each pair \((i,i')\) and any \(t>0\),
\[
\Pr\bigl(|g_{ii'}(\bm Z)-\mathbb E_{\bm Z}\,g_{ii'}(\bm Z)|\ge t\bigr)
\le 2\exp\!\Bigl(-\frac{t^2}{2K^2L^2d_x}\Bigr).
\]
A union bound over the \(\binom{d_x}{2}\) entries then shows that for any \(\varepsilon\in(0,1)\), with probability at least \(1-\varepsilon/3\),
\[
\|\widehat{\bm\Sigma} - \bm\Sigma\|_{\infty}
= \max_{i,i'}\bigl|g_{ii'}(\bm Z)-\mathbb E_{\bm Z}\,g_{ii'}(\bm Z)\bigr|
\le c_2\,K\,L\;\sqrt{d_x\log\!\bigl(d_x^2/\varepsilon\bigr)},
\]
where \(c_2>0\) is an absolute constant.  We denote this event by \(E_1\).  Establishing \(E_1\) completes our concentration argument for the inner‐product entries and sets the stage for analyzing the population Lasso estimator.  

\subsection*{Step 2: Primal–Dual Witness for the Population Lasso}

Building on the Gram‐matrix control from the previous section, we now analyze the population‐level Lasso problem.  Recall the population Gram
\[
\bm{\Sigma} \;=\;\mathbb{E}_{\bm{Z}}\bigl[Df(\bm{Z})\,Df(\bm{Z})^\top\bigr],
\]
and consider the estimator
\[
\min_{C\in\mathbb{R}^{d_x\times d_x}}
\;\mathbb{E}_{\bm{Z}}\bigl\lVert Df(\bm{Z}) - C\,Df(\bm{Z})\bigr\rVert_F^2
\;+\;\lambda\|C\|_1.
\]
\noindent\emph{Restricted strong convexity.}
By Assumption \ref{assp:restrict_eigenval}, the population Gram satisfies
\[
\bm{v}^\top\bm{\Sigma}\,\bm{v}
\;\ge\;
\kappa\,\|\bm{v}\|_2^2
\quad\text{whenever }\|\bm{v}\|_0\le s.
\tag{3.1a}
\]
Hence, the smooth part of the objective has the Hessian
\[
\,D^2Q(C)[\Delta C,\Delta C]
=2\sum_{i}(\Delta C)_{i,:}\,\bm{\Sigma}\,(\Delta C)_{i,:}^\top
\ge2\kappa\|\Delta C\|_F^2,
\]
so \(Q(C)\) is \(2\kappa\)–strongly convex on all row‑wise \(s\)–sparse directions, implying a unique minimizer \(C^*\).

\noindent \emph{Sample curvature.}
In practice, we replace \(\Sigma\) by its sample version \(\widehat\Sigma=\tfrac1N\sum_tDf(Z^{(t)})Df(Z^{(t)})^\top\). \cite{raskutti10a} shows that if \(N\gtrsim s\log d_z\), then with probability greater than \(1-\varepsilon/3\),
\[
\bm{v}^\top\widehat\Sigma\,\bm{v}
\;\ge\;
(\kappa/2)\|\bm{v}\|_2^2
\quad\forall\,\|\bm{v}\|_0\le s.
\tag{3.1b}
\]
Thus, the empirical risk is also strongly convex with high probability, again guaranteeing a unique minimizer over \(s\)–sparse rows. % (lemma 1 in raskutti10a)

\noindent\emph{Dual feasibility and setting \(\lambda\).}
Let \(S\) denote the true support of \(C^*\).  The KKT conditions on the complement \(S^c\) read
\[
\nabla_{S^c}\,\mathbb{E}\|Df - C\,Df\|_F^2\big|_{C=C^*}
\;+\;\lambda\,U_{S^c}
\;=\;0,
\]
with \(U_{S^c}\in[-1,1]^{|S^c|}\).  Enforcing the primal–dual witness \(C^*_{S^c}=0\) yields
\[
2\,\bm{\Sigma}_{S^c,S}\,C^*_{S} + \lambda\,U_{S^c} = 0
\quad\Longrightarrow\quad
\|\bm{\Sigma}_{S^c,S}C^*_{S}\|_\infty<\lambda.
\]
By mutual incoherence, \(\|\Sigma_{S^c,S}\Sigma_{S,S}^{-1}\|_\infty\le1-\gamma\), and dominance ensures \(\|\Sigma_{S,S}C^*_{S}\|_\infty\approx m_{\max}\), so deterministically \(\|\Sigma_{S^c,S}C^*_{S}\|_\infty\le(1-\gamma)m_{\max}\). Meanwhile, the high‑probability event \(E_1\) controls random fluctuations by \(\delta_{\rm rand}=c_2KL\sqrt{d_x\log(d_x^2/\varepsilon)}\).  Thus, choosing
\[
\lambda
=\Bigl(1-\tfrac\gamma2\Bigr)\,m_{\max}
\;+\;
c_2\,K\,L\;\sqrt{d_x\log\!\bigl(d_x^2/\varepsilon\bigr)}
\]
strictly exceeds \((1-\gamma)m_{\max}+\delta_{\rm rand}\), forcing \(C^*_{S^c}=0\).

\noindent At this point, we have shown that under \(E_1\) and the RE event, the population Lasso solution \(C^*\) recovers the correct support with high probability.  In the next section, we translate these coefficient bounds into affinity‐matrix guarantees and, ultimately, into clustering accuracy.

\subsection*{Step 3: Sign Consistency \& In‑Group Recovery}

Next, we show that any two features \(i,i'\), $i \neq i'$, in the same latent group \(G_j\) obtain a large positive self‑expression coefficient
\[
C^*_{ii'} 
\;=\;
\arg\min_{c\in\mathbb R}\;
\mathbb E_{\bm Z}\bigl\|\partial_i f(\bm Z)-c\,\partial_{i'} f(\bm Z)\bigr\|_2^2,
\]
and in particular 
\[
C^*_{ii'}\;\ge\;1 - (\delta+\mu)\;-\;\frac{c_2\,K\,L\,\sqrt{d_x}\,\log(d_x^2/\varepsilon)}{m_j}.
\]

To see this, note first that on the true one‑dimensional support \(S=\{(i,i')\}\), the \(\ell_1\) penalty drops out and \(C^*_{ii'}\) solves the simple least‑squares problem
\[
\min_{c\in\mathbb R}\;\mathbb E_{\bm Z}\bigl\|\partial_i f(\bm Z)-c\,\partial_{i'} f(\bm Z)\bigr\|_2^2.
\]
Differentiating under the expectation and setting to zero gives the closed‑form
\[
C^*_{ii'}
=\frac{\mathbb E_{\bm Z}\langle \partial_i f(\bm Z),\;\partial_{i'}f(\bm Z)\rangle}
       {\mathbb E_{\bm Z}\|\partial_{i'}f(\bm Z)\|_2^2}.
\]
We now bound the numerator and denominator in turn.  By Dominance \ref{assp:dominance_partial}, the key partial \(\partial f_i/\partial z_j\) satisfies
\[
\mathbb E_{\bm Z}\Bigl|\frac{\partial f_i}{\partial \bm  z_j}(\bm  Z)\Bigr|
\ge(1-\delta)\,\sqrt{\mathbb E_{\bm Z}\|\nabla_{\bm z} f_i(\bm Z)\|^2}
=(1-\delta)\sqrt{m_j}.
\]
Moreover, Mutual Incoherence ensures that cross‑terms contribute at most \(\mu\,\sqrt{m_j^2}\), so altogether
\[
\mathbb E_{\bm Z}\langle \partial_i f(\bm Z),\;\partial_{i'}f(\bm Z)\rangle
\;\ge\;(1-\delta-\mu)\,m_j.
\]

On the other hand, from the uniform deviation event \(E_1\) we know each entry of the empirical Gram deviates by at most \(\Delta:=c_2\,K\,L\sqrt{d_x\log(d_x^2/\varepsilon)}\).  In particular,
\[
\bigl|\|\partial_{i'}f(\bm Z)\|_2^2 - \mathbb E_{}\|\partial_{i'}f(\bm Z)\|_2^2\bigr|
\le\Delta,
\]
and since \(\mathbb E_{\bm Z}\|\partial_{i'}f(\bm Z)\|_2^2=m_j\), we have
\[
\mathbb E_{\bm Z}\|\partial_{i'}f(\bm Z)\|_2^2
\;\le\;
m_j + \Delta.
\]

Putting these together,
\[
C^*_{ii'}
=\frac{\mathbb E_{\bm Z}\langle \partial_i f(\bm Z),\partial_{i'}f(\bm Z)\rangle}{\mathbb E_{\bm Z}\|\partial_{i'}f(\bm Z)\|_2^2}
\;\ge\;
\frac{(1-\delta-\mu)\,m_j}{\,m_j+\Delta\,}
\;\ge\;
1 - (\delta+\mu) - \frac{\Delta}{m_j},
\]
which is the stated bound 
\[
\displaystyle
C^*_{ii'}\ge1 - (\delta+\mu) - \tfrac{c_2KL\sqrt{d_x}\,\log(d_x^2/\varepsilon)}{m_j}.
\]
\subsection*{Step 4: Affinity Matrix \& Block Bounds}

With the support recovery and coefficient bounds in place, define the induced affinity
\[
A^*_{ii'} \;=\; |C^*_{ii'}| \;+\; |C^*_{i'i}|.
\]
On the intersection of our two high‑probability events \(E_1\) (uniform deviation of \(\widehat\Sigma\)) and \(E_2\) (empirical RE), we obtain sharp “block” estimates separating in‑group from cross‑group affinities.

\vspace{0.5em}
\emph{Intra‑cluster bound.}
If \(i,i'\in Ch(j)\), then by the sign‑consistency argument, each of \(C^*_{ii'}\) and \(C^*_{i'i}\) obeys
\[
C^*_{\bullet\,\bullet}\;\ge\;1 - (\delta+\mu)
\;-\;\frac{c_2\,K\,L\,\sqrt{d_x\,\log(d_x^2/\varepsilon)}}{m_j},
\]
so summing yields
\[
A^*_{ii'}
\;\ge\;
2\Bigl(1 - (\delta+\mu)\Bigr)
\;-\;\frac{2\,c_2\,K\,L\,\sqrt{d_x\,\log(d_x^2/\varepsilon)}}{m_j}.
\]
Absorbing constants into \(C_3=2c_2\) and re‑scaling by \(m_j\) gives the clean form
\[
A^*_{ii'} 
\;\ge\;
\bigl(1 - \delta - \mu\bigr)\,m_j
\;-\;
C_3\,K\,L\,\sqrt{d_x\,\log\!\bigl(\tfrac{d_x^2}{\varepsilon}}\bigr).
\]

\vspace{0.5em}
\emph{Inter‑cluster bound.}
If \(i\in Ch(j)\) and \(i'\in Ch(k)\) with \(k\neq j\), then dual‑feasibility forces \(C^*_{ii'}=0\) on the population level, and concentration adds at most \(c_2KL\sqrt{d_x\log(d_x^2/\varepsilon)}\) to each coefficient.  Hence
\[
A^*_{ii'}
\;\le\;
\Bigl|\mathbb E_{\bm Z}\langle\partial_i f(\bm Z),\partial_{i'} f(\bm Z)\rangle\Bigr|
\;+\;
C_3\,K\,L\,\sqrt{d_x\,\log\!\bigl(\tfrac{d_x^2}{\varepsilon}\bigr)}
\;\le\;
\mu\,\sqrt{m_jm_k}
\;+\;
C_3\,K\,L\,\sqrt{d_x}\,\log\!\bigl(\tfrac{d_x^2}{\varepsilon}\bigr),
\]
which in the symmetric‐affinity form becomes
\[
A^*_{ii'} 
\;\le\;
\mu\,m_j\,m_k
\;+\;
C_3\,K\,L\,\sqrt{d_x\,\log\!\bigl(\tfrac{d_x^2}{\varepsilon}\bigr)}.
\]

These two inequalities reveal a gap between “strong” in‑group affinities and “weak” cross‑group affinities—precisely the structure needed for the subsequent spectral perturbation and clustering steps.  

\subsection*{Step 5: Spectral Perturbation \& Eigenspace Deviation}

To transition from coefficient bounds to clustering, we compare the observed affinity \(A^*\) with the ideal block matrix 
\[
H=\sum_{j}m_{j}\,1_{G_j}1_{G_j}^\top,
\]
and let the perturbation be 
\[
E = A^* - H.
\]
Our goal is to show that \(E\) is small in operator norm and thus the leading eigenspaces of \(A^*\) and \(H\) remain close.

Gershgorin’s circle \citep{horn2012matrix} theorem first controls the size of \(E\).  Since each row of \(E\) has at most \(d_x\) nonzero entries, each is bounded in magnitude by 
\[
C_3\,K\,L\,\sqrt{d_x\,\log\!\bigl(d_x^2/\varepsilon\bigr)},
\]
we obtain
\[
\|E\|_2\;\le\;\|E\|_{1,\infty}
\;\le\;d_x\,C_3\,K\,L\,\sqrt{d_x\,\log\!\bigl(d_x^2/\varepsilon\bigr)}.
\]

Next, Weyl’s inequality for symmetric matrices \citep{horn2012matrix} implies that every eigenvalue of \(A^*\) deviates from its counterpart in \(H\) by at most \(\|E\|_2\):
\[
\bigl|\lambda_i(A^*)-\lambda_i(H)\bigr|\;\le\;\|E\|_2
\quad\forall\,i.
\]

We then define the critical eigengap
\[
\Delta
=\min_j m_j \;-\;\mu\max_{k\ne j}\sqrt{m_jm_k}
\;-\;2\|E\|_2.
\]
Whenever \(\Delta>0\), the Davis–Kahan sin \(\Theta\) theorem \citep{davis1970rotation} guarantees that the distance between the top-\(d_z\) eigenspaces of \(H\) and \(A^*\) is controlled by
\[
\|\sin\Theta(\widehat U,U)\|_2
\;\le\;\frac{\|E\|_2}{\Delta},
\]
and in particular, each eigenvector satisfies
\[
\|\widehat u_i - u_i\|_2
\;\le\;\frac{\|E\|_2}{\Delta}.
\]
Thus, under the gap condition \(\Delta>0\), the spectral embeddings produced by \(A^*\) remain within a small radius of the ideal block‑model embeddings—paving the way for accurate rounding in the clustering step.  

\subsection*{Step 6.1: SAAC Rounding}

After forming the affinity matrix \(A^*\), SAAC \citep{panov2017SAAC} extracts its top \(d_z\) eigenvectors 
\[
\widehat U = \bigl[\hat u^1,\dots,\hat u^{d_z}\bigr]\in\mathbb R^{d_x\times d_z},
\]
and then fits a binary membership matrix \(Z\in\{0,1\}^{d_x\times d_z}\) alongside a prototype matrix \(X\in\mathbb R^{d_z\times d_z}\) by minimizing 
\[
\|\widehat U - Z\,X\|_F^2
\quad\text{subject to }Z_{i,\cdot}\neq0\ \forall i,
\]
so that each feature \(i\) is assigned to at least one cluster and \(\widehat U\approx ZX\).

In practice, SAAC alternates between  
\[
X \;=\;\arg\min_X\|\widehat U - Z\,X\|_F^2 
\;=\;(Z^\top Z)^{-1}Z^\top\widehat U
\]
and, for each \(i\),
\[
Z_i \;=\;\arg\min_{z\in\{0,1\}^{d_z}\setminus\{0\}}\|\widehat U_i - z\,X\|_2^2
\;=\;\begin{cases}
1 &\text{at }j=\arg\min_k\|\widehat U_i - X_k\|_2,\\
0 &\text{otherwise},
\end{cases}
\]
i.e.\ each feature picks the single prototype \(X_j\) closest in Euclidean distance to its embedding \(\widehat U_i\).  These two updates are repeated until convergence.  

The success of this \emph{nearest‑neighbor rounding} follows from our perturbation bounds: with probability \(\ge 1-\varepsilon\),  
\[
\|\widehat U_i - U_i\|_2\;\le\;\frac{\|E\|_2}{\Delta},
\]
where \(U_i\) is the ideal block‑model embedding and \(\Delta\) the eigengap.  In the noiseless block model \(H=\sum_jm_j1_{G_j}1_{G_j}^\top\), the normalized indicator eigenvectors \(\{u_j\}\) satisfy  
\[
\|u_j - u_{j'}\|_2\;\ge\;2,\quad j\neq j'.
\]
Hence if 
\[
\frac{\|E\|_2}{\Delta}<\tfrac12,
\]
then each \(\widehat U_i\) lies within \(1/2\) of its true \(U_i\) and farther from any other \(u_{j'}\).  Nearest‑neighbor rounding therefore selects the correct cluster(s), and when overlaps occur, features lie near intersections of the relevant \(\{u_j\}\), still recovered as long as the intersection angles exceed the noise radius.  Combining these facts yields the misclassification rate
\[
\max\limits_{ 1 \leq j \leq d_z} \frac{|\widehat G_j\triangle G_j|}{|G_j|}
=\mathcal O\!\Bigl(\delta + \tfrac{\mu}{\gamma} + \tfrac{K\,L\,\;\sqrt{d_x\log(d_x^2/\varepsilon)}}{\min\limits_{ 1 \leq j \leq d_z} m_j}\Bigr).
\]
as claimed in the Theorem \ref{thm:overlap_cluster_recovery}.  

\subsection*{Step 6.2: SymNMF Rounding}

SymNMF \citep{Kuang2015SymNMF} replaces the binary assignment of SAAC with a nonnegative factorization.  We fit
\[
\min_{Y\ge0}\;F(Y)\;=\;\bigl\|A^*-Y\,Y^\top\bigr\|_F^2,
\]
where each row \(Y_i\) encodes soft memberships of feature \(i\).  The classic multiplicative update of  \citet{Kuang2015SymNMF}),
\[
Y_{ij}\;\leftarrow\;Y_{ij}\;\times\;
\frac{[\,A^*Y\,]_{ij}}{[\,Y\,Y^\top Y\,]_{ij}},
\]
preserves nonnegativity and drives \(F(Y)\) downward until a stationary point \(Y^*\) is reached.

Once converged, we normalize each row,
\[
T_i = Y^*_i \bigl/\|Y^*_i\|_1\;\in\;\Delta^{d_z-1},
\]
and then “round” by hard‐thresholding:
\[
Z_{i,j} =
\begin{cases}
1, & j = \displaystyle\arg\max_k\,T_{i,k},\\[1ex]
0, & \text{otherwise}.
\end{cases}
\]
In practice, when several entries tie within a small tolerance, all corresponding clusters may be assigned to \(i\), capturing overlaps.

Under the same eigenspace perturbation bound \(\|\widehat U - U\|_{2\to\infty}\!\le\!\|E\|_2/\Delta\), the ideal block‑model solution \(Y=U\Lambda^{1/2}\) (with rows proportional to the indicator eigenvectors) is perturbed only slightly.  A perturbation smaller than half the gap between the top two coordinates of each ideal row cannot change the index of the largest entry, so hard‐thresholding recovers the exact cluster memberships.  Allowing ties yields overlap‐aware assignments.  Hence, SymNMF achieves the same misclassification rate,
\[
\max_j\frac{|\widehat G_j\triangle G_j|}{|G_j|}
=O\!\Bigl(\delta + \tfrac\mu\gamma + \tfrac{KL\sqrt{d_x\log(d_x^2/\varepsilon)}}{\min_jm_j}\Bigr),
\]
completing the proof of the theorem \ref{thm:overlap_cluster_recovery}.

\subsection{Generalization and Stability Under the Self-Expression Problem}

\paragraph{Proof of Theorem \ref{thm:genetalization_SExprLoss}}
We aim to control the uniform generalization gap:
\[
\Delta :=
\sup_{C \in \mathcal{C}_\lambda}
\left| \mathbb{E}_{\mathbf{x} \sim p_{data}}[\bar{\ell}(C, f; \mathbf{x}) ] - \frac{1}{N} \sum_{i=1}^N \bar{\ell}(C, f; \mathbf{x})  \right|,
\quad \text{where} \quad
\bar{\ell}(C, f; \mathbf{x}) = \left\| (I - C)\bar{J}_f(\mathbf{x}; q_\phi) \right\|_F^2.
\]
\subparagraph{Step 1: Symmetrization.}
By the standard symmetrization inequality (see \cite[Theorem 3.1]{bartlett2002rademacher}), we have:
\[
\mathbb{E}_{\mathbf{X}_{1:N}}[\Delta]
\le
2\,\mathbb{E}_{\mathbf{x}_{1:N},\,\sigma_{1:N}}
\left[ \sup_{C \in \mathcal{C}_\lambda}
\frac{1}{N} \sum_{i=1}^N \sigma_i\,\ell(C; \mathbf{x}_i) \right],
\]
where \( \sigma_i \in \{ \pm 1 \} \) are  Rademacher variables which are independent.

\subparagraph{Step 2: Contraction via Ledoux–Talagrand.}
Fix \(\mathbf{x} \in \mathcal{X} \subset \mathbb{R}^{d_x} \). Since \( \|\bar{J}_f(\mathbf{x}; q_\phi)\|_F \le M_\phi \), appplying the contraction inequality \citep{ledoux2001concentration} gives:
\[
\mathbb{E}_\sigma \left[
\sup_{C \in \mathcal{C}_\lambda}
\frac{1}{N} \sum_{i=1}^N \sigma_i \| \bar{\ell}(C, f; \mathbf{x}_i) \|_F^2
\right]
\le
4M \cdot \mathbb{E}_\sigma \left[
\sup_{C \in \mathcal{C}_\lambda}
\frac{1}{N} \sum_{i=1}^N \sigma_i \langle \bar{\ell}(C, f; \mathbf{x}_i) , E \rangle_F
\right],
\]
%, the function \( h \mapsto \|h\|_F^2 \) is \( 2M \)-Lipschitz on the ball of radius \( M \). 
where \( E \in \mathbb{R}^{n \times d} \) is an auxiliary matrix (a “ghost sample”) used in the contraction argument.

\subparagraph{Step 3: Reduction to linear class.}
Since
\[
\langle \bar{\ell}(C, f; \mathbf{x}_i) , E \rangle_F = \langle \bar{J}_f(\mathbf{x}_i; q_\phi), E \rangle_F - \langle C \bar{J}_f(\mathbf{x}_i; q_\phi), E \rangle_F,
\]
and the first term is independent of \( C \), we reduce to bounding:
\[
\mathbb{E}_\sigma \left[
\sup_{C \in \mathcal{C}_\lambda}
\frac{1}{N} \sum_{i=1}^N \langle C \bar{J}_f(\mathbf{x}_i; q_\phi), \sigma_i \rangle_F
\right].
\]

\subparagraph{Step 4: Bounding the Rademacher complexity.}
Define the class of self-expressive tangent maps:
\[
\mathcal{H}_{\lambda,f} := \left\{ \mathbf{x} \mapsto C \bar{J}_f(\mathbf{x}; q_\phi) \;\middle|\; C \in \mathbb{R}^{d_x \times d_x},\; \mathrm{diag}(C) = 0,\; \|C\|_1 \le \lambda \right\}.
\]
Using the duality \( \sup\limits_{\|C\|_1 \le \lambda} \langle C, A \rangle = \lambda \|A\|_\infty \), the Rademacher complexity \(\mathfrak{R}_N(\mathcal{H}_{\lambda,f})\) of \(\mathcal{H}_{\lambda,f}\) is bounded:
\[
\mathfrak{R}_N(\mathcal{H}_{\lambda,f})
\le
\frac{\lambda}{N} \mathbb{E}_\sigma \left\| \sum_{i=1}^N \sigma_i \bar{J}_f(\mathbf{x}_i; q_\phi)^\top \right\|_\infty.
\]
Since \( \|\bar{J}_f(\mathbf{x}_i; q_\phi)\|_F \le M_{\phi} \) implies \( \|\bar{J}_f(\mathbf{x}_i; q_\phi)\|_{\rm op} \le M_\phi \), classical matrix concentration \citep{tropp2012user} gives:
\[
\mathbb{E}_\sigma \left\| \sum_{i=1}^N \sigma_i \bar{J}_f(\mathbf{x}_i; q_\phi)^\top \right\|_\infty
\le
M_{\phi} \sqrt{2 N \log d_x},
\]
thus:
\[
\mathfrak{R}_N(\mathcal{H}_{\lambda,f})
\le
\lambda M_{\phi} \sqrt{ \frac{2 \log d_x}{N} }.
\]
\subparagraph{Step 5: Final bound via McDiarmid’s inequality.}
Combining the above gives:
\[
\mathbb{E}_{\mathbf{X}_{1:N}}[\Delta]
\le
8 \lambda M_\phi^2 \sqrt{ \frac{2 \log d_x}{N} }.
\]
To lift this to a high-probability bound, we apply McDiarmid’s inequality \citep{ShalevShwartzBenDavid2014}: with probability at least \( 1 - \delta \) we finally obtain
\[
\Delta
\le
8 \lambda M_\phi^2 \sqrt{ \frac{2 \log d_x}{N} }
+ M_\phi^2 \sqrt{ \frac{2 \log(1/\delta)}{N} }.
\]
% or a standard concentration result for empirical Rademacher processes

\paragraph{Proof of Proposition~\ref{prop:jacobian-perturbation}} 
Write \(A = \tilde{\mathrm{D}}f(\mathbf{Z})\), \(E = E(\mathbf{Z})\), and \(\Delta = I - C^*\). Then:
\[
\|\mathrm{D}f(\mathbf{Z})- \mathrm{D}f(\mathbf{Z})C^*\|_F^2
= \|(\tilde{\mathrm{D}}f(\mathbf{Z}) + E(\mathbf{Z}))\Delta\|_F^2
= \|\tilde{\mathrm{D}}f(\mathbf{Z})\Delta\|_F^2
+ 2\langle \tilde{\mathrm{D}}f(\mathbf{Z})\Delta, E(\mathbf{Z})\Delta\rangle_F
+ \|E(\mathbf{Z})\Delta\|_F^2.
\]
Thus, the deviation satisfies:
\[
\left| \|\mathrm{D}f(\mathbf{Z})- \mathrm{D}f(\mathbf{Z})C^*\|_F^2 - \|\tilde{\mathrm{D}}f(\mathbf{Z}) - \tilde{\mathrm{D}}f(\mathbf{Z})C^*\|_F^2 \right|
= \left| 2\langle \tilde{\mathrm{D}}f(\mathbf{Z})\Delta, E(\mathbf{Z})\Delta\rangle_F + \|E(\mathbf{Z})\Delta\|_F^2 \right|.
\]

\subparagraph{Step 1: Bounding \(\|E(\mathbf{Z})\Delta\|_F\).}
We have \(\|E(\mathbf{Z})\Delta\|_F \le \|E(\mathbf{Z})\|_F \|\Delta\|_{\mathrm{op}}\). Since \(E\) has \(d_x\) independent sub-Gaussian columns, by vector concentration \cite[Proposition 3.3.7]{vershynin2018HDProba}, there exists \(\Lambda_1 > 0\) such that for any \(\delta \in (0,1)\),
\[
\mathbb{P}\left\{ \|E(\mathbf{Z})\|_F > \Lambda_1 \varepsilon \sqrt{d_z d_x} + \varepsilon \sqrt{2d_z \ln(2d_x/\delta)} \right\} \le \delta.
\]
Thus, with probability at least \(1-\delta\),
\[
\|E(\mathbf{Z})\Delta\|_F \le \|\Delta\|_{\mathrm{op}} \left( \Lambda_1 \varepsilon \sqrt{d_z d_x} + \varepsilon \sqrt{2d_z \ln\tfrac{2d_x}{\delta}} \right).
\]

\subparagraph{Step 2: Bounding the cross term.}
By Cauchy–Schwarz inequality:
\[
\left| \langle \tilde{\mathrm{D}}f(\mathbf{Z})\Delta, E(\mathbf{Z})\Delta \rangle_F \right|
\le \|\tilde{\mathrm{D}}f(\mathbf{Z})\Delta\|_F \|E(\mathbf{Z})\Delta\|_F
\le \|\tilde{\mathrm{D}}f(\mathbf{Z})\|_F \|\Delta\|_{\mathrm{op}} \|E(\mathbf{Z})\Delta\|_F.
\]
Since \(\|\tilde{\mathrm{D}}f(\mathbf{Z})\|_F = \sqrt{d_x}\), we have:
\[
\left| \langle \tilde{\mathrm{D}}f(\mathbf{Z})\Delta, E(\mathbf{Z})\Delta \rangle_F \right|
\le \sqrt{d_x} \|\Delta\|_{\mathrm{op}} \left( \Lambda_1 \varepsilon \sqrt{d_z d_x} + \varepsilon \sqrt{2d_z \ln\tfrac{2d_x}{\delta}} \right).
\]

\subparagraph{Step 3: Final combination.}
Thus, with probability at least \(1-\delta\),
\[
\begin{aligned}
\left| \|\mathrm{D}f(\mathbf{Z})- \mathrm{D}f(\mathbf{Z})C^*\|_F^2 - \|\tilde{\mathrm{D}}f(\mathbf{Z}) - \tilde{\mathrm{D}}f(\mathbf{Z})C^*\|_F^2 \right|
&\le 2 \sqrt{d_x} \|\Delta\|_{\mathrm{op}} \left( \Lambda_1 \varepsilon \sqrt{d_z d_x} + \varepsilon \sqrt{2d_z \ln\tfrac{2d_x}{\delta}} \right) \\
&\quad + \|\Delta\|_{\mathrm{op}}^2 \left( \Lambda_1 \varepsilon \sqrt{d_z d_x} + \varepsilon \sqrt{2d_z \ln\tfrac{2d_x}{\delta}} \right)^2.
\end{aligned}
\]
Recalling \(\|\Delta\|_{\mathrm{op}} = \|I - C^*\|_{\mathrm{op}} \le 1 + \|C^*\|_{\mathrm{op}}\) and setting
\[
B(\delta) := \Lambda_1 \sqrt{d_z d_x} + \sqrt{2d_z \ln\tfrac{2d_x}{\delta}},
\]
the bound simplifies to:
\[
\left| \|\mathrm{D}f(\mathbf{Z})- \mathrm{D}f(\mathbf{Z})C^*\|_F^2 - \|\tilde{\mathrm{D}}f(\mathbf{Z}) - \tilde{\mathrm{D}}f(\mathbf{Z})C^*\|_F^2 \right|
\le (1 + \|C^*\|_{\mathrm{op}}) \left( 2\sqrt{d_x} B(\delta) \varepsilon + (1 + \|C^*\|_{\mathrm{op}}) B(\delta)^2 \varepsilon^2 \right).
\]

% \subsection{Robustness under Perturbation}
% When $A$ is only approximately block-diagonal, the Davis–Kahan $\sin\Theta$ theorem \citep{yu2014useful} implies that the top-$k$ eigenspace of $L_{\mathrm{sym}}$ remains close to the ideal indicator subspace as long as:
% \[
% \|A - A_{\text{ideal}}\|_2 \ll \lambda_{k+1} - \lambda_k.
% \]
% The eigengap $\lambda_{k+1} - \lambda_k$ is lower-bounded by the component separation, so small perturbations do not alter the cluster structure.
